# Supplementary material for: Dynamic estimation with random forests for discrete-time survival data
Source: arXiv:2103.01355 ancillary file (2021-03-03)
Supplement: Supplementary file 1 [file supplemental_material.pdf]

# Supplemental Material for "Dynamic Estimation with Random Forests for Discrete-Time Survival Data"

Hoora MORADIAN[1], Weichi YAO[2], Denis LAROCQUE[1], Jeffrey S. SIMONOFF[2], and Halina FRYDMAN[2]

[1]*Department of Decision Sciences, HEC Montréal, 3000 chemin de la Côte-Sainte-Catherine, Montréal, Québec, Canada H3T 2A7.*

[2]*Department of Technology, Operations, and Statistics, Stern School of Business, New York University, USA*

# Contents

**S1 Simulation study** **3**

S1.1 Data generation processes . . . . . . . . . . . . . . . . . . . . . . . 3

S1.2 Box-plots for each combination of $(t, u)$ . . . . . . . . . . . . . 10

S1.3 Summary tables . . . . . . . . . . . . . . . . . . . . . . . . . . . . . 59

S1.4 The shrinkage effect of the Superpp method . . . . . . . . . . . 72

**S2 Real data example** **73**

# S1 Simulation study

## S1.1 Data generation processes

The discrete-time survival data is generated based on the following steps:

1. Generate a sequence of $N$ (uncensored) survival times from the original continuous-time survival time generation scheme. Get the interval end points $0, t_1, t_2, \ldots, t_T$ for $T$ periods, where $t_i$ is the value in the sequence of the $N$ survival times at the $100 \times i/T$ percentile;

2. Generate the covariates' values $\boldsymbol{X}_0, \ldots, \boldsymbol{X}_{T-1}$ for $[0, t_1), \ldots, [t_{T-1}, t_T]$, implying that the covariates' values change $T-1$ times;

3. Compute the continuous survival times $\{T_{Ci}\}$ based on (2), and generate the censoring times $\{C_{Ci}\}$ independently. Then

$$\widetilde{T}_{Ci} = \min\{T_{Ci}, C_{Ci}\}.$$

   (I) If there exists $j \in \{1, \ldots, T\}$ such that $\widetilde{T}_{Ci} \in [t_{j-1}, t_j)$, then we set $\widetilde{T}_{Di} = j$;

   (II) If $\widetilde{T}_{Ci} > t_T$, then $\widetilde{T}_{Di} = T$.

4. The survival probability $S_D(j \mid \boldsymbol{X}_i)$ at time $j$ for given $i$-th covariates $\boldsymbol{X}_i$ is computed based on the survival probability of the corresponding continuous case $S_C(j \mid \boldsymbol{X}_i)$:

(i) For situation (I) in 3, given $j = 1, ..., T$

$$S_D(j \mid \boldsymbol{X}_i) = \mathbb{P}\big(\widetilde{T}_{Di} > j \mid \boldsymbol{X}_i\big) = \mathbb{P}\big(\widetilde{T}_{Ci} > t_j \mid \boldsymbol{X}_i\big) = S_C(t_j \mid \boldsymbol{X}_i).$$

(ii) For situation (II) in 3

$$S_D(T \mid \boldsymbol{X}_i) = \mathbb{P}\big(\widetilde{T}_{Di} > T \mid \boldsymbol{X}_i\big) = \mathbb{P}\big(\widetilde{T}_{Ci} > T \mid \boldsymbol{X}_i\big) = S_C(t_T \mid \boldsymbol{X}_i).$$

In the simulation study, there are ten covariates in total. $X_1$, $X_3$ and $X_8$ are all binary, $X_2$, $X_4$ and $X_7$ are generated from $\text{Unif}(0, 1)$, $X_5$ and $X_9$ are sampled from $\{1, 2, 3, 4, 5\}$, and $X_6$ and $X_{10}$ follows $\text{Unif}(0, 2)$. Among them, $X_1, X_2, X_7$ are time-invariant, while the rest are time-varying. The details for different variations of DGP are as follows.

**Scenario** Table S1.1 provides the different combinations of numbers of time-invariant and time-varying covariates in the true generating model considered in the simulation study. Only the first six covariates are given in the table since $X_7$ to $X_{10}$ are never involved in the true DGP.

| Scenario | Time-invariant | | Time-varying | | | |
|---|---|---|---|---|---|---|
| | $X_1$ | $X_2$ | $X_3$ | $X_4$ | $X_5$ | $X_6$ |
| 0TI + 2TV | | | | ✓ | | ✓ |
| 0TI + 4TV | | | ✓ | ✓ | ✓ | ✓ |
| 1TI + 4TV | | ✓ | ✓ | ✓ | ✓ | ✓ |
| 2TI + 1TV | ✓ | ✓ | | | | ✓ |
| 2TI + 4TV | ✓ | ✓ | ✓ | ✓ | ✓ | ✓ |

**Table S1.1:** Different combinations of numbers of time-invariant and time-varying covariates in the true generating model (Scenario).

**Survival distribution** In generating the continuous-time survival data, the survival time $T_C$ follows an Exponential distribution, a Weibull distribution or a Gompertz distribution under a proportional hazards model. Consider the underlying hazard function

$$h(t) = h_0(t) \exp \left( \vartheta(\boldsymbol{X}(t)) \right)$$

where $\vartheta(\boldsymbol{X}(t))$ is a function of the covariates $\boldsymbol{X}(t)$ (including the time-invariant ones) in the true model. The cumulative hazard function is then given by

$$H(t) = \int_0^t h_0(s) \exp \left( \vartheta(\boldsymbol{X}(s)) \right) ds,$$

implying the survival function

$$S(t) = \exp(-H(t)).$$

The three underlying true distributions of event times are as follows.

1. Exponential: the baseline hazard function is given by

   $$h_0(t) = \lambda,$$

   where $\lambda > 0$. The survival time can be simulated with $u \sim \mathcal{U}(0, 1)$ and

   $$T_C = -\frac{\log(u)}{\lambda \exp\big(\vartheta\big(\boldsymbol{X}(t_1)\big)\big)}, \qquad \text{if } -\log(u) < H(t_1),$$

   with $t_1$ the first time of change, and so on.

2. Weibull: the baseline hazard function is given by

   $$h_0(t) = \lambda \nu t^{\nu-1},$$

   where $\lambda > 0$ and $\nu > 1$. The survival time can be simulated with $u \sim \mathcal{U}(0, 1)$ and

   $$T_C = \left(-\frac{\log(u)}{\lambda \exp\big(\vartheta\big(\boldsymbol{X}(t_1)\big)\big)}\right)^{1/\nu}, \qquad \text{if } -\log(u) < H(t_1),$$

   with $t_1$ the first time of change, and so on.

3. Gompertz: the baseline hazard function is given by

   $$h_0(t) = \lambda \exp(\alpha t),$$

where $\lambda > 1$ and $\alpha = 0.1$. The survival time can be simulated with $u \sim \mathcal{U}(0, 1)$ and

$$T_C = \frac{1}{\alpha} \log \left( 1 - \frac{\alpha \log(u)}{\lambda \exp\left(\vartheta\big(\boldsymbol{X}(t_1)\big)\right)} \right), \qquad \text{if } -\log(u) < H(t_1),$$

with $t_1$ the first time of change, and so on.

**Survival relationship** We consider three survival relationships between the hazards and the covariates, a log-linear survival relationship, a log-nonlinear survival relationship and a log-interaction model. In each of the setups, the survival time $T_C$ depends on $\vartheta(\boldsymbol{X})$, which is a function of the covariates. We illustrate with the scenario 2TI + 4TV.

I. Log-linear: $\vartheta\big(\boldsymbol{X}(t)\big) = \exp\big((1, c_1\boldsymbol{X}(t))\boldsymbol{\beta}\big)$ with some constants $c_1$ and $\boldsymbol{\beta} = (\beta_0, \dots, \beta_6)'$.

II. Log-nonlinear: $\vartheta\big(\boldsymbol{X}(t)\big) = \exp\big(c_0 + c_1 \log((1, c_2\boldsymbol{X}(t))\boldsymbol{\alpha})\big)$ with some constants $c_0$, $c_1$, $c_2$ and $\boldsymbol{\alpha} = (\alpha_0, \dots, \alpha_6)'$.

III. Interaction: $\vartheta$ is determined by the value of time-invariant covariate $X_2$ and the value of time-varying covariate $X_6$. Figure S1.1 gives an example of the structure of the covariates driving the interaction survival relationship,

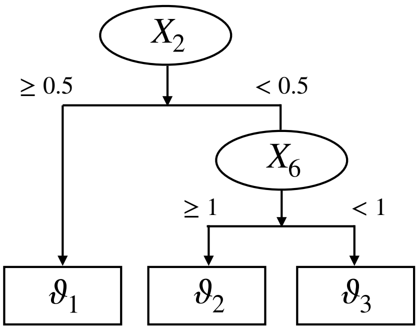


**Figure S1.1:** The structure of the covariates driving the log-interaction survival relationship in scenario 2TI + 4TV (1TI + 4TV and 2TI + 1TV)

where $\vartheta_1, \vartheta_2, \vartheta_3$ correspond to

$$\vartheta_1 = \exp\big(c_3(X_3(t) - 1)(X_5(t)/3)^2 + (X_1(t) - 1)X_4(t)^{X_2(t)}\big);$$

$$\vartheta_2 = \exp\big((1, c_1\boldsymbol{X}(t))\boldsymbol{\beta}\big);$$

$$\vartheta_3 = \exp\big(c_0 + c_1 \log(|(1, \boldsymbol{X}(t))\boldsymbol{\alpha}|)\big),$$

where $c_0$, $c_1$, $c_3$, $\boldsymbol{\beta} = (\beta_0, \ldots, \beta_6)'$ and $\boldsymbol{\alpha} = (\alpha_0, \ldots, \alpha_6)'$ are given constants.

**Signal-to-noise ratio** We manage the signal-to-noise ratio by setting different values of the coefficients for the covariates in $\vartheta(\boldsymbol{X}(t))$. From signal-to-noise ratio low to high, $c_1 = 1.5$ is increased to $c_1 = 3$, $c_2 = 1$ to $c_2 = 2$, $c_3 = 1$ to $c_3 = 3$, while keeping $\{\beta_j, j = 1, \ldots, 6\}$ and/or $\{\alpha_j, j = 1, \ldots, 6\}$ the same.

**Autocorrelations** We set the autocorrelations of the same covariate in the true model to be 0.4 for the weak case and 0.9 for the strong case, and set correlations between any two covariates in the true model to be 0.1 in the weak case and 0.2 in the strong case. For example, for the scenario 2TI + 4TV, the corresponding matrices for strong and weak autocorrelation are $C_{1,\,\text{2TI+4TV}}$ and $C_{0,\,\text{2TI+4TV}}$ defined as follows,

$$C_{1,\,\text{2TI+4TV}} = \begin{pmatrix} 1 & 0 & 0 & 0 & 0 & 0 \\ 0 & 1 & 0 & 0 & 0 & 0 \\ 0 & 0.2 & 0.9 & 0.2 & 0.2 & 0.2 \\ 0 & 0.2 & 0.2 & 0.9 & 0.2 & 0.2 \\ 0 & 0.2 & 0.2 & 0.2 & 0.9 & 0.2 \\ 0 & 0.2 & 0.2 & 0.2 & 0.2 & 0.9 \end{pmatrix},$$

$$C_{0,\,\text{2TI+4TV}} = \begin{pmatrix} 1 & 0 & 0 & 0 & 0 & 0 \\ 0 & 1 & 0 & 0 & 0 & 0 \\ 0 & 0.1 & 0.4 & 0.1 & 0.1 & 0.1 \\ 0 & 0.1 & 0.1 & 0.4 & 0.1 & 0.1 \\ 0 & 0.1 & 0.1 & 0.1 & 0.4 & 0.1 \\ 0 & 0.1 & 0.1 & 0.1 & 0.1 & 0.4 \end{pmatrix}.$$

In the scenario 1TI + 4TV, the corresponding matrices for strong and weak autocorrelation are $C_{1,\,\text{1TI+4TV}}$ and $C_{0,\,\text{1TI+4TV}}$ defined as follows,

$$C_{1,\,\text{1TI+4TV}} = \begin{pmatrix} 1 & 0 & 0 & 0 & 0 & 0 \\ 0 & 1 & 0 & 0 & 0 & 0 \\ 0 & 0.2 & 0.9 & 0.2 & 0.2 & 0.2 \\ 0 & 0.2 & 0.2 & 0.9 & 0.2 & 0.2 \\ 0 & 0.2 & 0.2 & 0.2 & 0.9 & 0.2 \\ 0 & 0.2 & 0.2 & 0.2 & 0.2 & 0.9 \end{pmatrix},$$

$$C_{0,\,\text{1TI+4TV}} = \begin{pmatrix} 1 & 0 & 0 & 0 & 0 & 0 \\ 0 & 1 & 0 & 0 & 0 & 0 \\ 0 & 0.1 & 0.4 & 0.1 & 0.1 & 0.1 \\ 0 & 0.1 & 0.1 & 0.4 & 0.1 & 0.1 \\ 0 & 0.1 & 0.1 & 0.1 & 0.4 & 0.1 \\ 0 & 0.1 & 0.1 & 0.1 & 0.1 & 0.4 \end{pmatrix}.$$

## S1.2 Box-plots for each combination of $(t, u)$

Figures S1.2 to S1.25 provide box-plots for ADIST based on the 500 simulations runs of each method for each combination $(t, u)$, and Figures S1.26 to S1.49 do the same for C-index.

In each plot for a given value of $t$, $T - t$ groups of box-plots are presented for each $u = t + 1, \ldots, T$ from left to right. For each group (with a specific pair of values $(t, u)$), the modeling methods are trained on the same test set for performance comparison. Each of these test sets includes only the subjects that are still at risk at $u$, given the information of the covariates up to $t$.

These box-plots show the measurement values for each method. For Figures S1.2 to S1.25 where results for ADIST are provided, a box-plot giving a lower median location corresponds to a better performance evaluated by ADIST. For Figures S1.26 to S1.49 where results for C-index are provided, a box-plot giving a higher median location corresponds to a better performance evaluated by C-index.

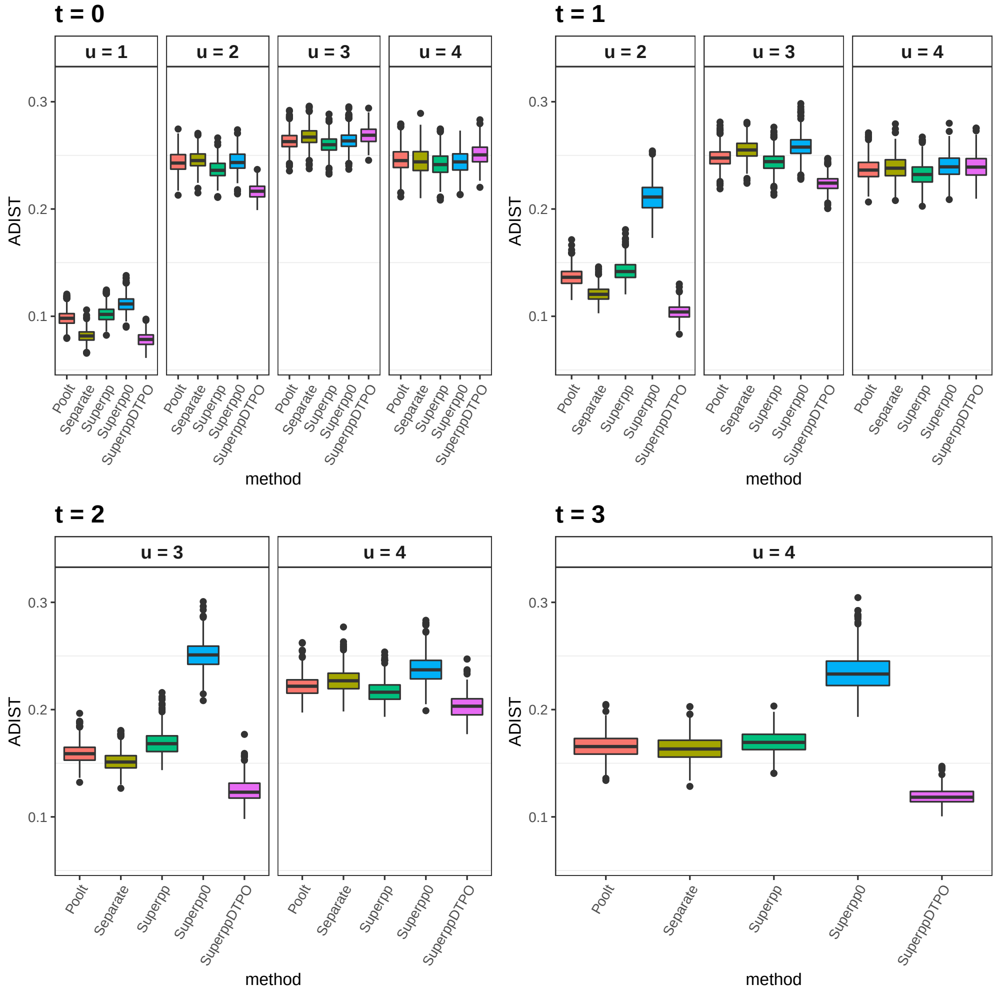


**Figure S1.2:** Simulation results comparing the distribution of ADIST on test sets across methods for each pair of $(t, u)$, trained on sample data of size 1000, 10% censoring rate, generated following a Weibull distribution with a linear survival relationship under the scenario 2TI + 4TV, high signal-to-noise ratio and strong autocorrelation. The number of periods $T = 4$.

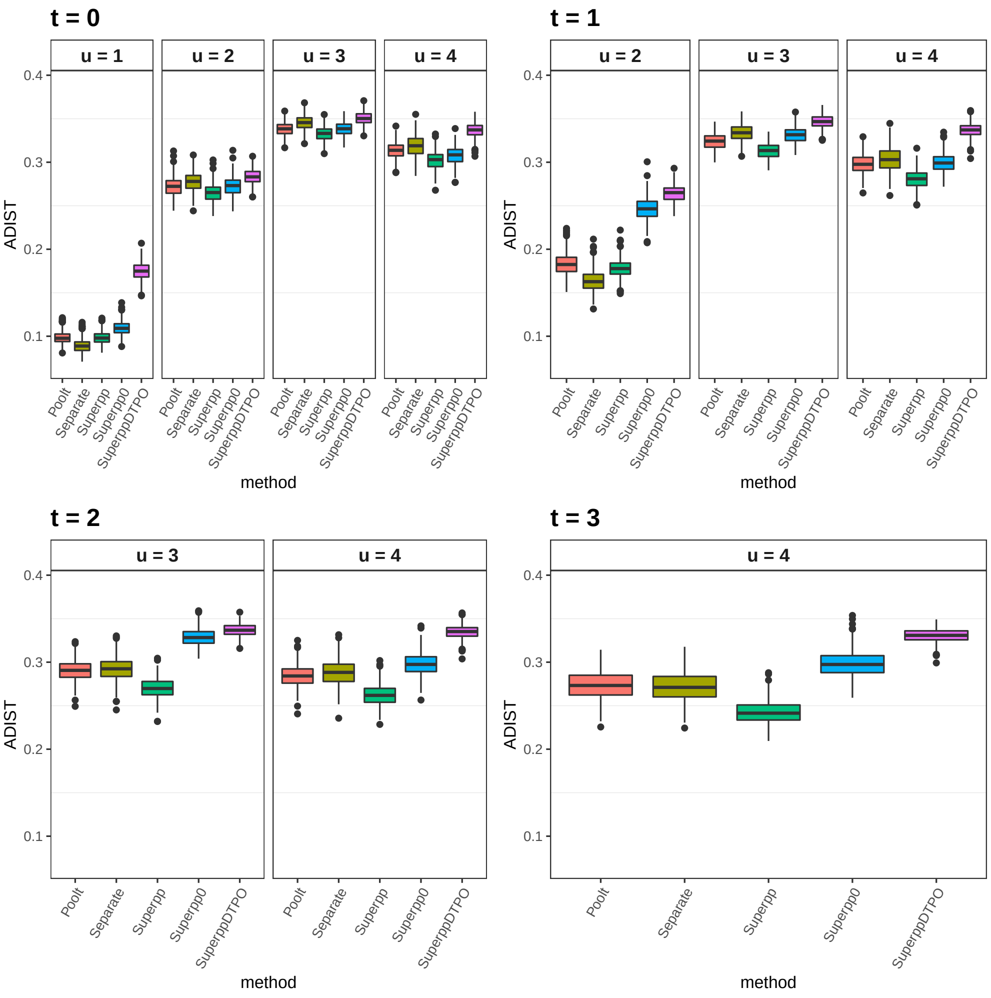


**Figure S1.3:** Simulation results comparing the distribution of ADIST on test sets across methods for each pair of $(t, u)$, trained on sample data of size 1000, 10% censoring rate, generated following a Weibull distribution with a nonlinear survival relationship under the scenario 2TI + 4TV, high signal-to-noise ratio and strong autocorrelation. The number of periods $T = 4$.

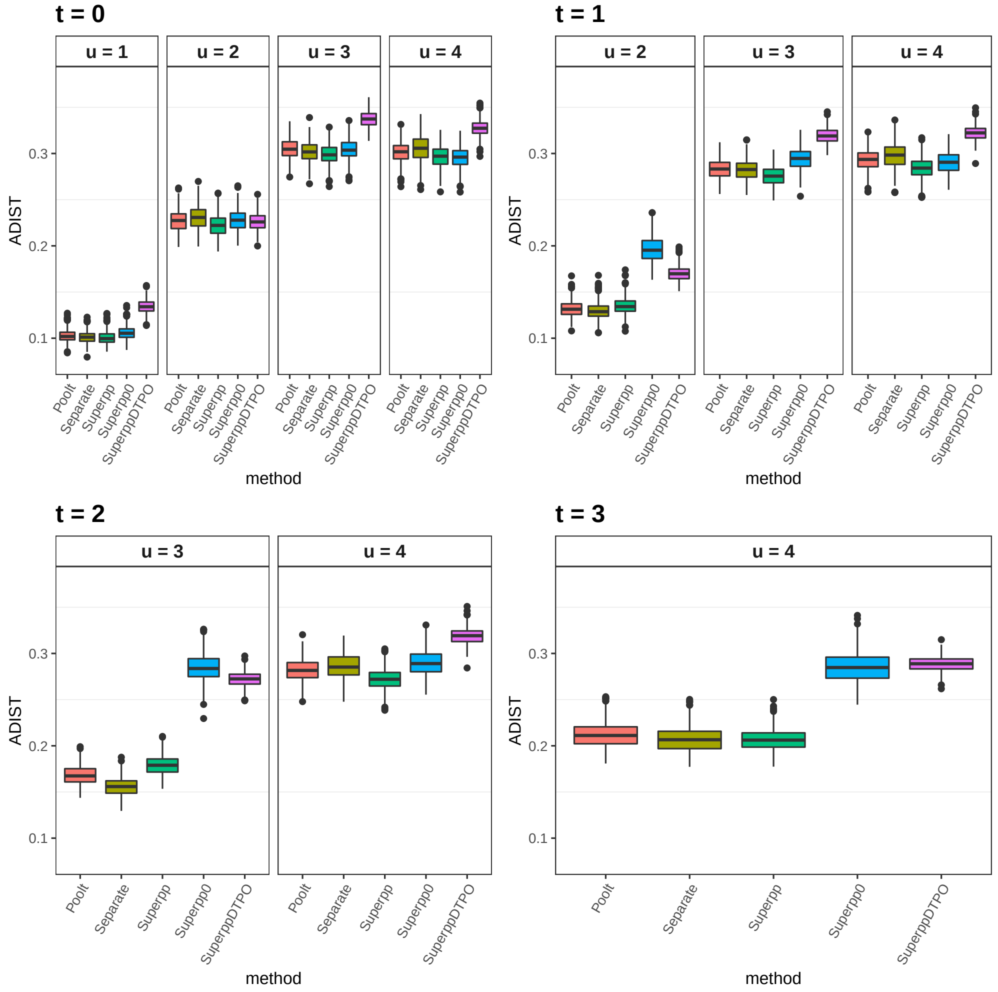


**Figure S1.4:** Simulation results comparing the distribution of ADIST on test sets across methods for each pair of $(t, u)$, trained on sample data of size 1000, 10% censoring rate, generated following a Weibull distribution with an interaction survival relationship under the scenario 2TI + 4TV, high signal-to-noise ratio and strong autocorrelation. The number of periods $T = 4$.

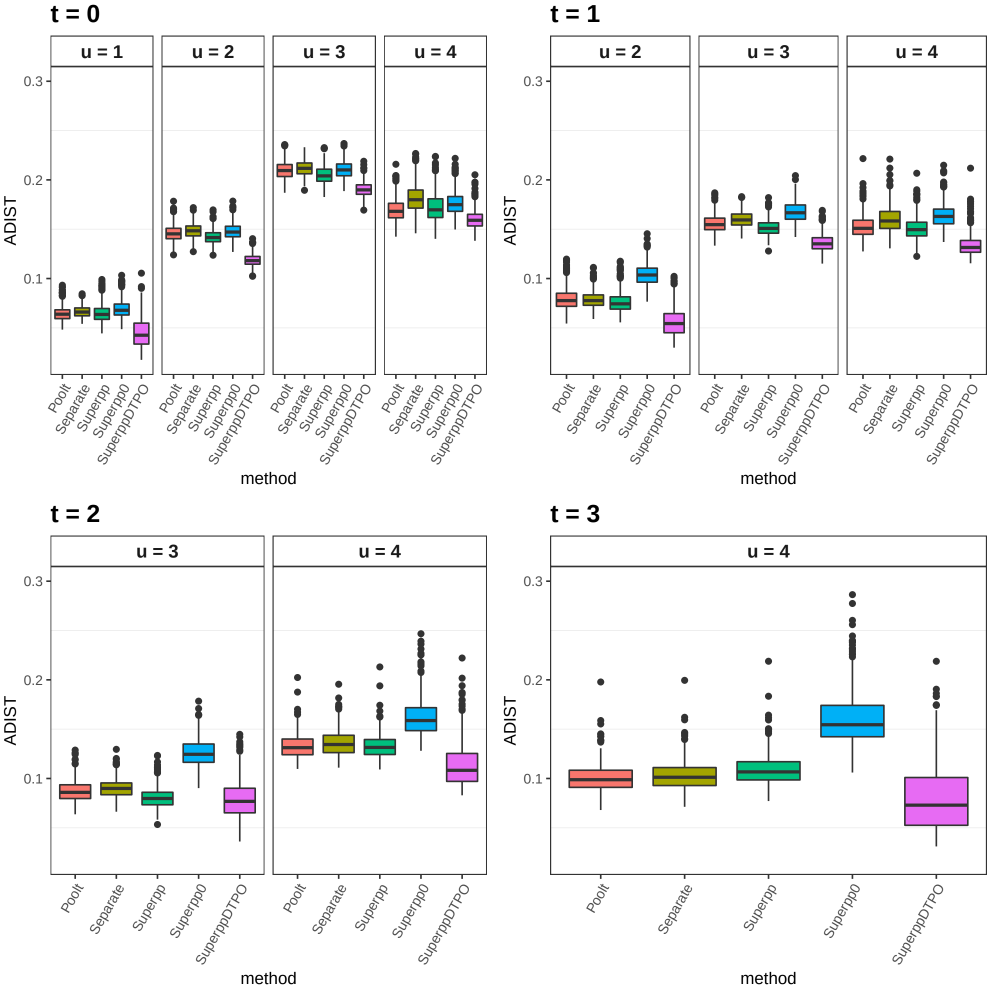


**Figure S1.5:** Simulation results comparing the distribution of ADIST on test sets across methods for each pair of $(t, u)$, trained on sample data of size 1000, 10% censoring rate, generated following a Weibull distribution with a linear survival relationship under the scenario 2TI + 4TV, low signal-to-noise ratio and strong autocorrelation. The number of periods $T = 4$.

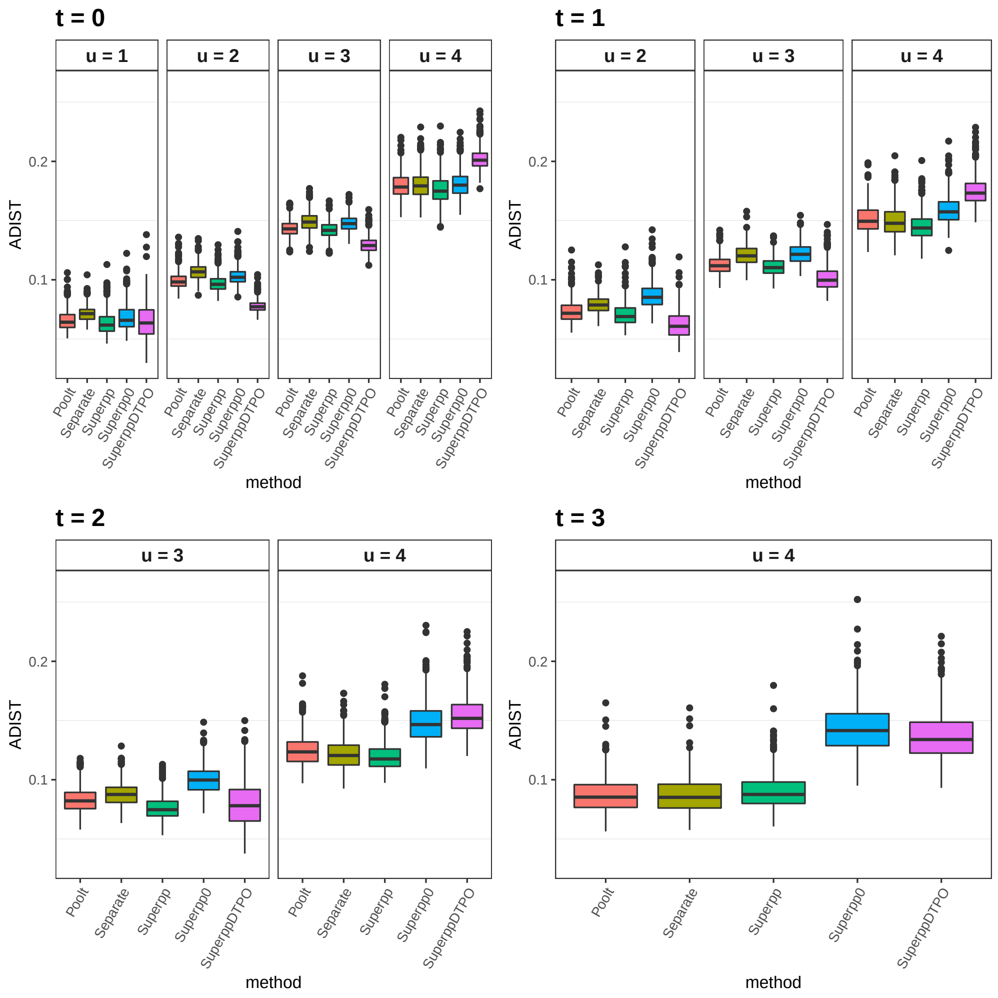


**Figure S1.6:** Simulation results comparing the distribution of ADIST on test sets across methods for each pair of $(t, u)$, trained on sample data of size 1000, 10% censoring rate, generated following a Weibull distribution with a nonlinear survival relationship under the scenario 2TI + 4TV, low signal-to-noise ratio and strong autocorrelation. The number of periods $T = 4$.

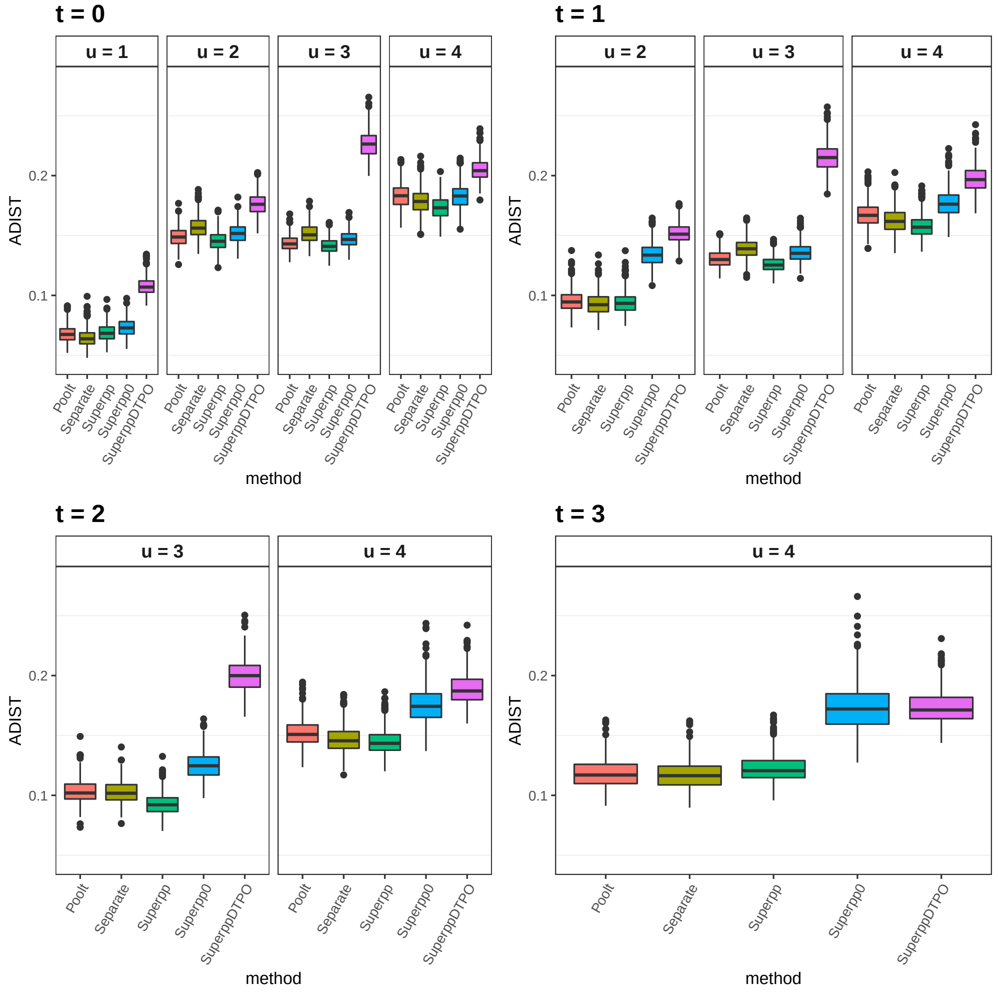


**Figure S1.7:** Simulation results comparing the distribution of ADIST on test sets across methods for each pair of $(t, u)$, trained on sample data of size 1000, 10% censoring rate, generated following a Weibull distribution with an interaction survival relationship under the scenario 2TI + 4TV, low signal-to-noise ratio and strong autocorrelation. The number of periods $T = 4$.

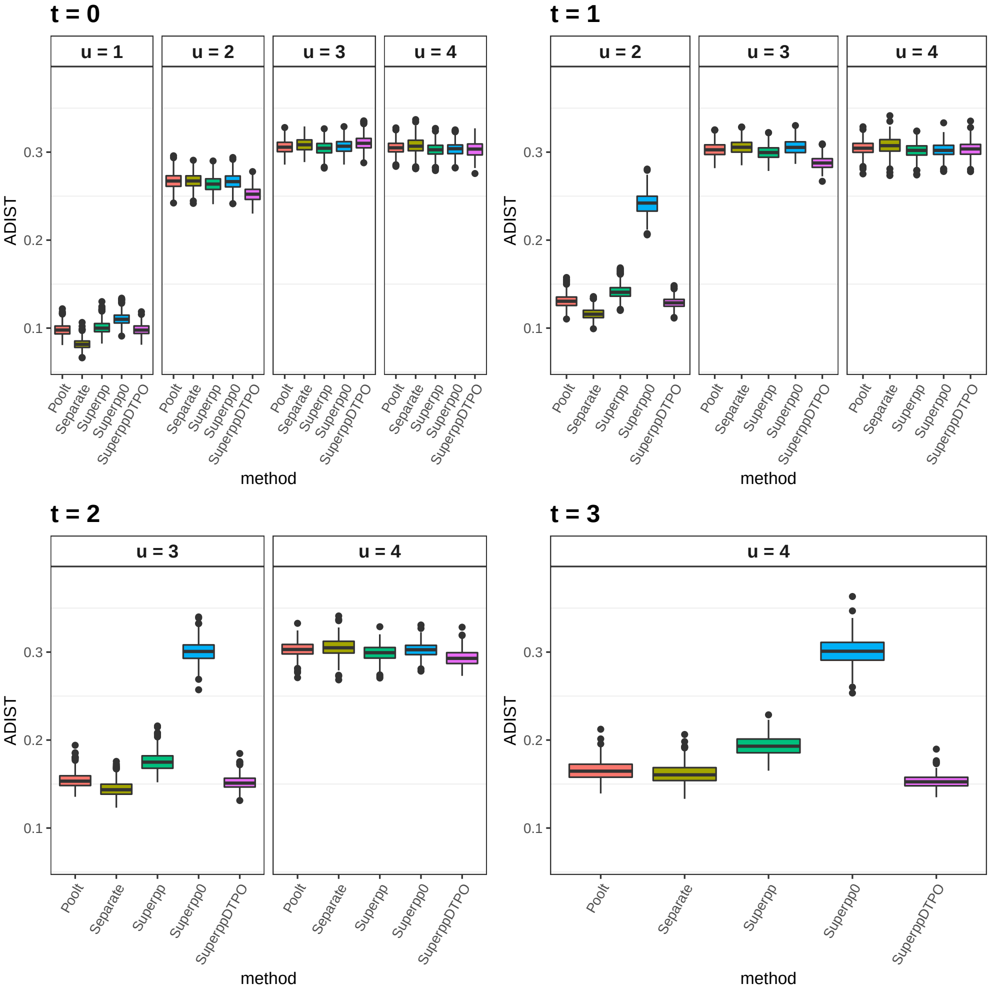


**Figure S1.8:** Simulation results comparing the distribution of ADIST on test sets across methods for each pair of $(t, u)$, trained on sample data of size 1000, 10% censoring rate, generated following a Weibull distribution with a linear survival relationship under the scenario 2TI + 4TV, high signal-to-noise ratio and weak autocorrelation. The number of periods $T = 4$.

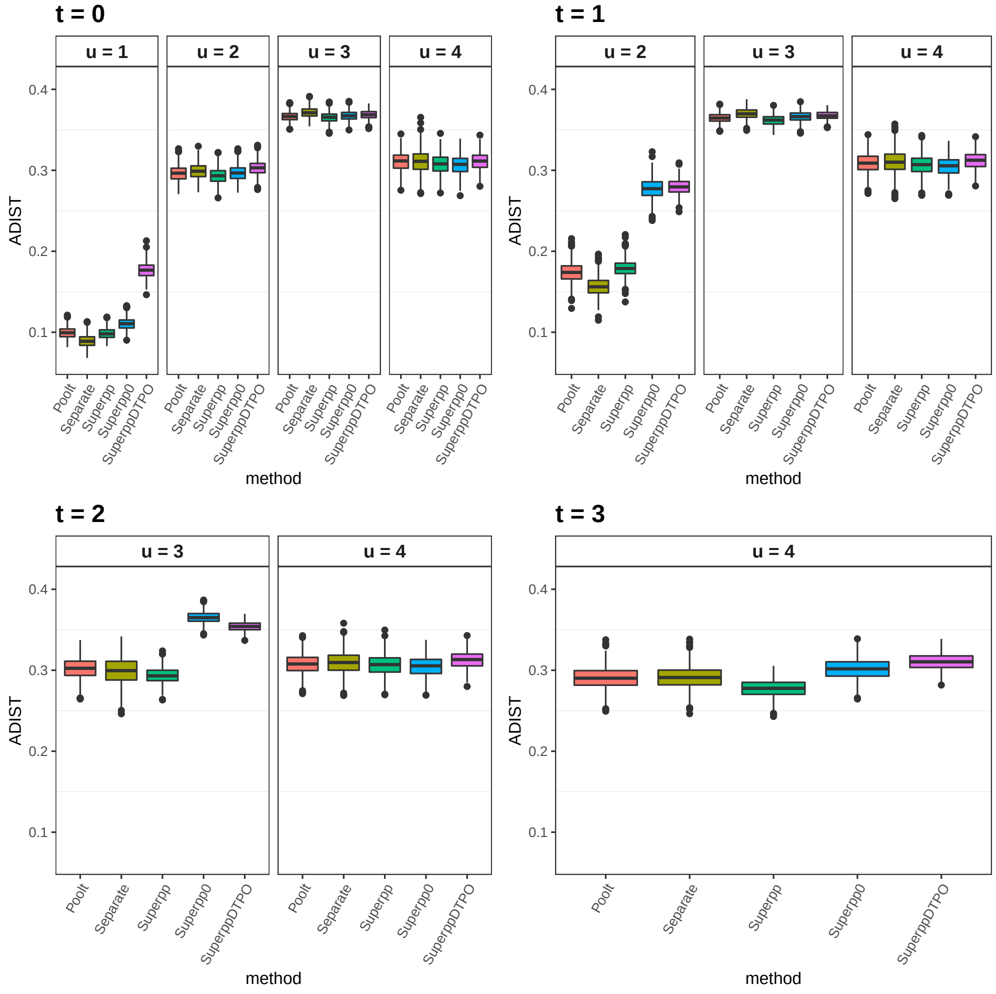


**Figure S1.9:** Simulation results comparing the distribution of ADIST on test sets across methods for each pair of $(t, u)$, trained on sample data of size 1000, 10% censoring rate, generated following a Weibull distribution with a nonlinear survival relationship under the scenario 2TI + 4TV, high signal-to-noise ratio and weak autocorrelation. The number of periods $T = 4$.

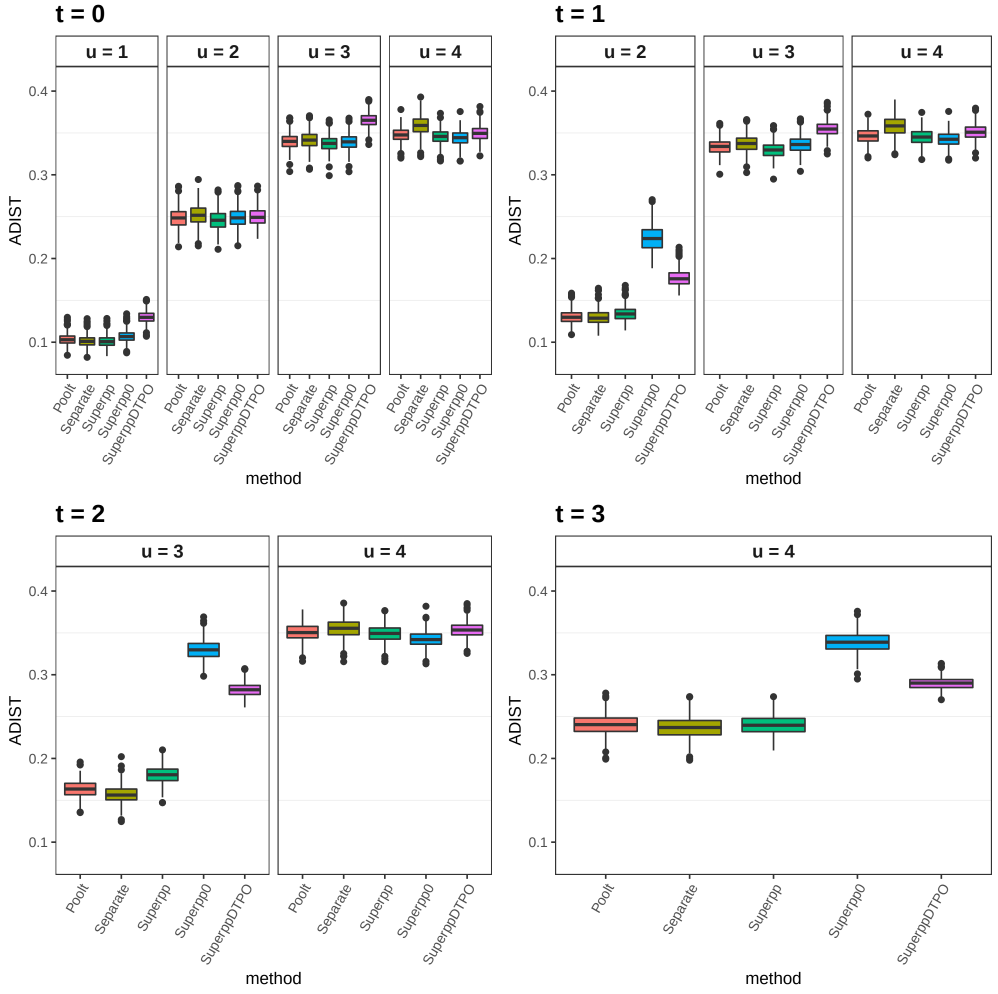


**Figure S1.10:** Simulation results comparing the distribution of ADIST on test sets across methods for each pair of $(t, u)$, trained on sample data of size 1000, 10% censoring rate, generated following a Weibull distribution with an interaction survival relationship under the scenario 2TI + 4TV, high signal-to-noise ratio and weak autocorrelation. The number of periods $T = 4$.

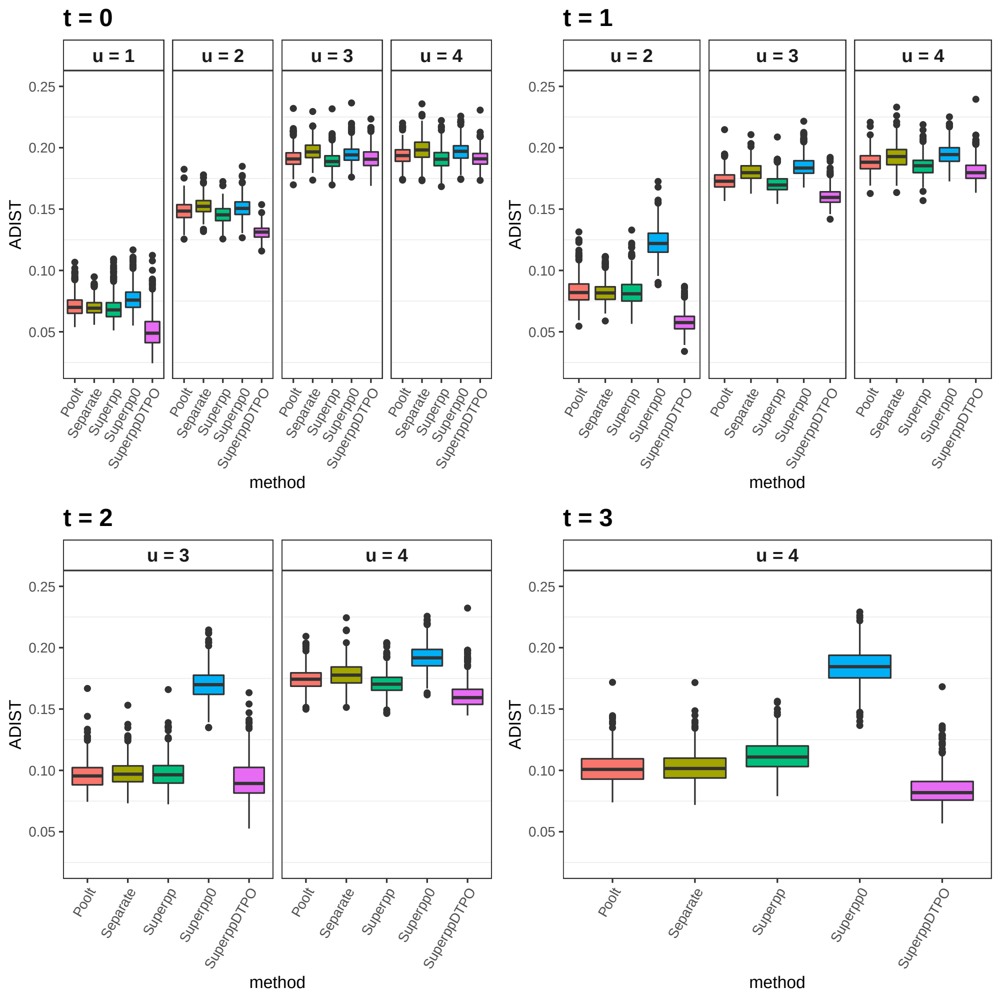


**Figure S1.11:** Simulation results comparing the distribution of ADIST on test sets across methods for each pair of $(t, u)$, trained on sample data of size 1000, 10% censoring rate, generated following a Weibull distribution with a linear survival relationship under the scenario 2TI + 4TV, low signal-to-noise ratio and weak autocorrelation. The number of periods $T = 4$.

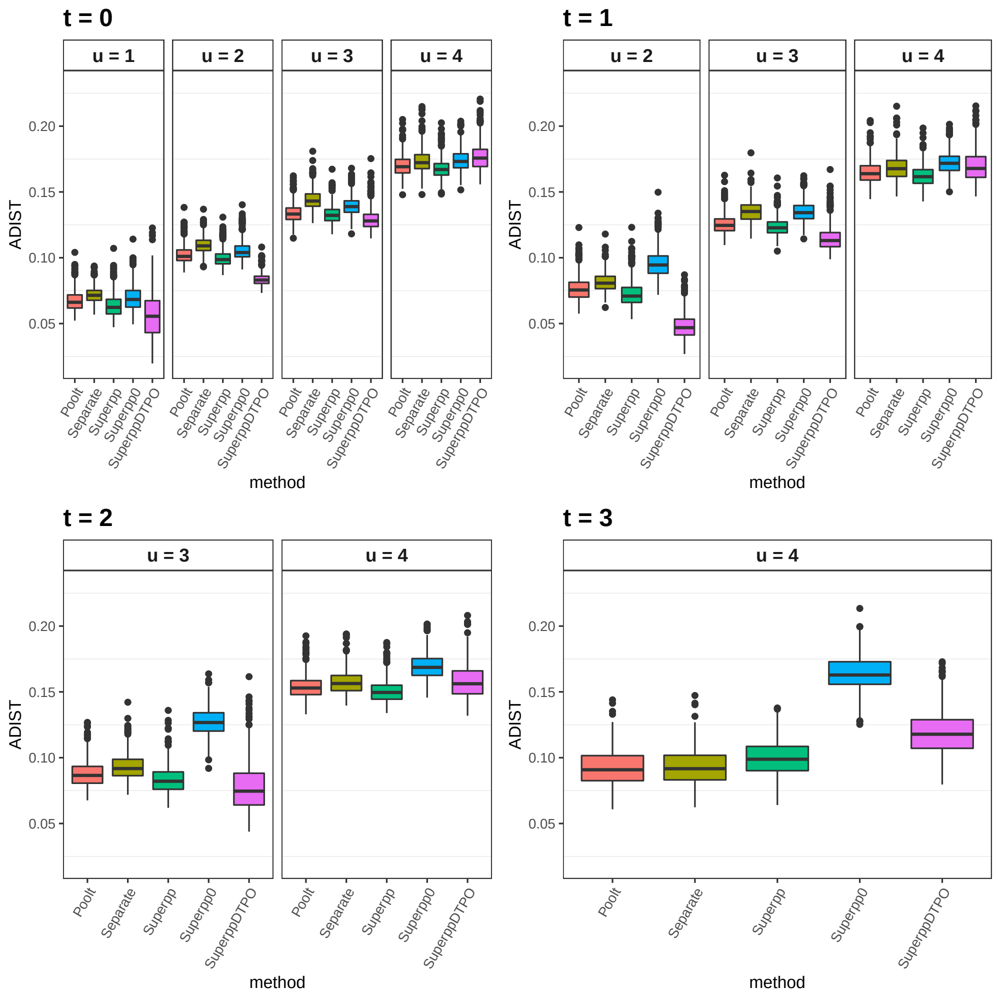


**Figure S1.12:** Simulation results comparing the distribution of ADIST on test sets across methods for each pair of $(t, u)$, trained on sample data of size 1000, 10% censoring rate, generated following a Weibull distribution with a nonlinear survival relationship under the scenario 2TI + 4TV, low signal-to-noise ratio and weak autocorrelation. The number of periods $T = 4$.

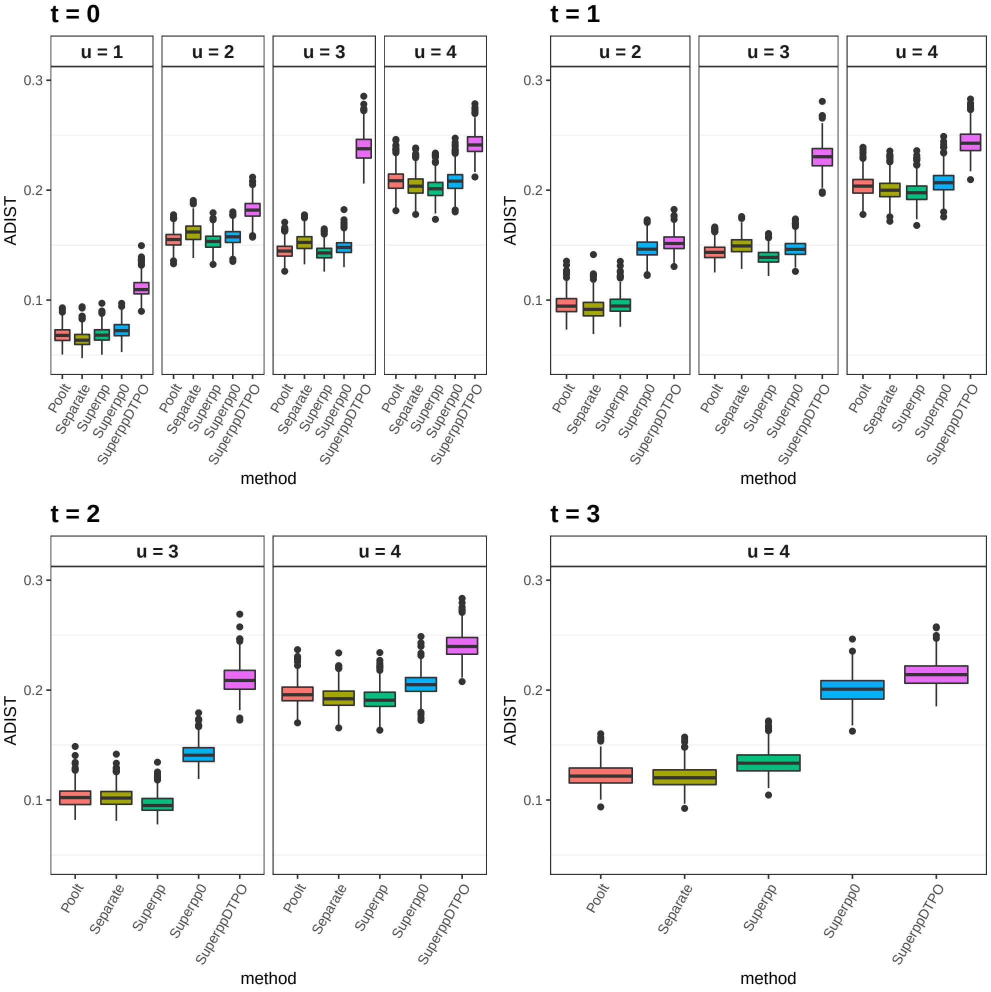


**Figure S1.13:** Simulation results comparing the distribution of ADIST on test sets across methods for each pair of $(t, u)$, trained on sample data of size 1000, 10% censoring rate, generated following a Weibull distribution with an interaction survival relationship under the scenario 2TI + 4TV, low signal-to-noise ratio and weak autocorrelation. The number of periods $T = 4$.

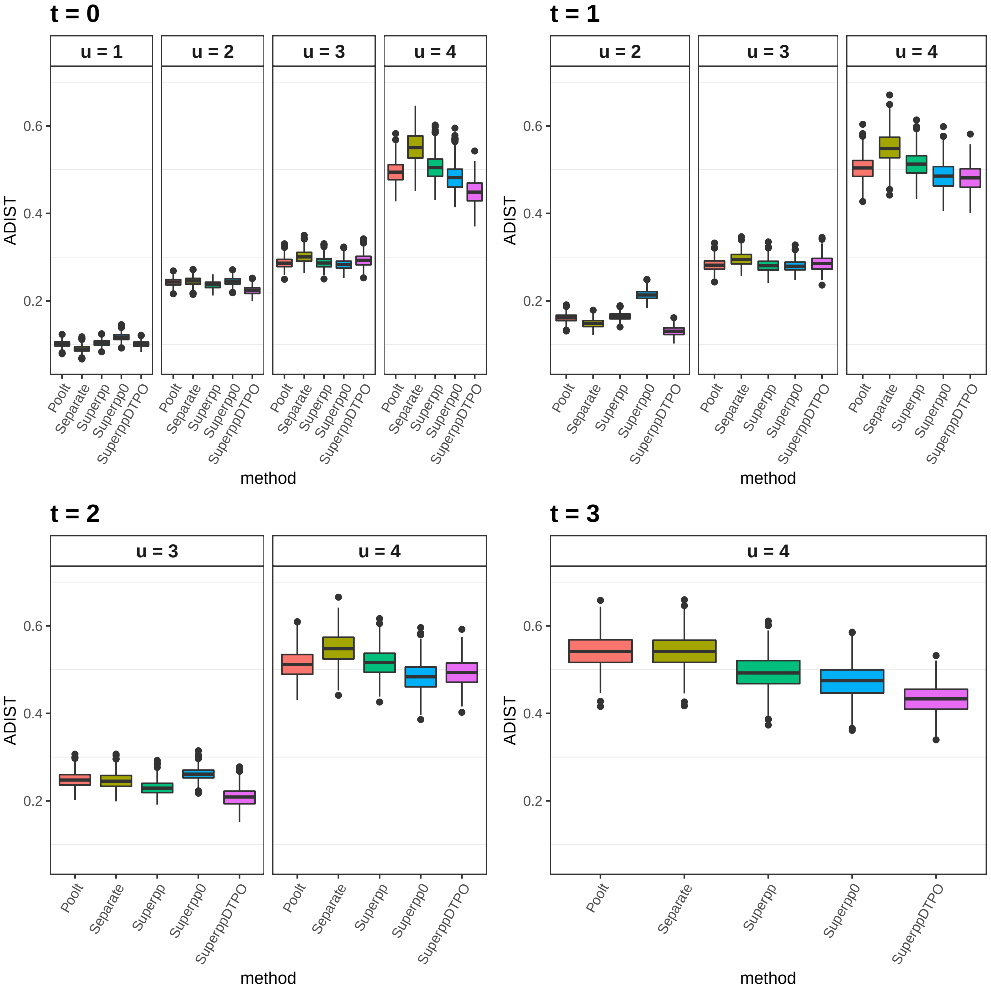


**Figure S1.14:** Simulation results comparing the distribution of ADIST on test sets across methods for each pair of $(t, u)$, trained on sample data of size 1000, 50% censoring rate, generated following a Weibull distribution with a linear survival relationship under the scenario 2TI + 4TV, high signal-to-noise ratio and strong autocorrelation. The number of periods $T = 4$.

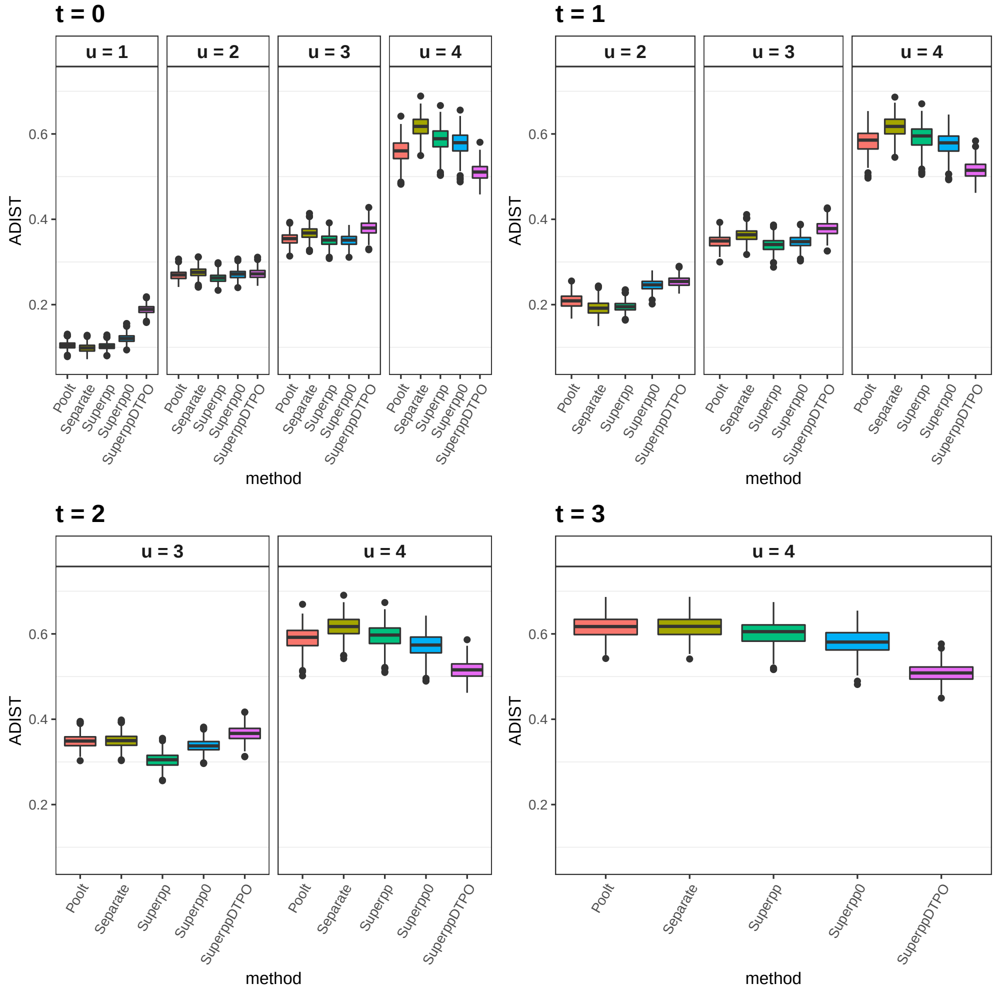


**Figure S1.15:** Simulation results comparing the distribution of ADIST on test sets across methods for each pair of $(t, u)$, trained on sample data of size 1000, 50% censoring rate, generated following a Weibull distribution with a nonlinear survival relationship under the scenario 2TI + 4TV, high signal-to-noise ratio and strong autocorrelation. The number of periods $T = 4$.

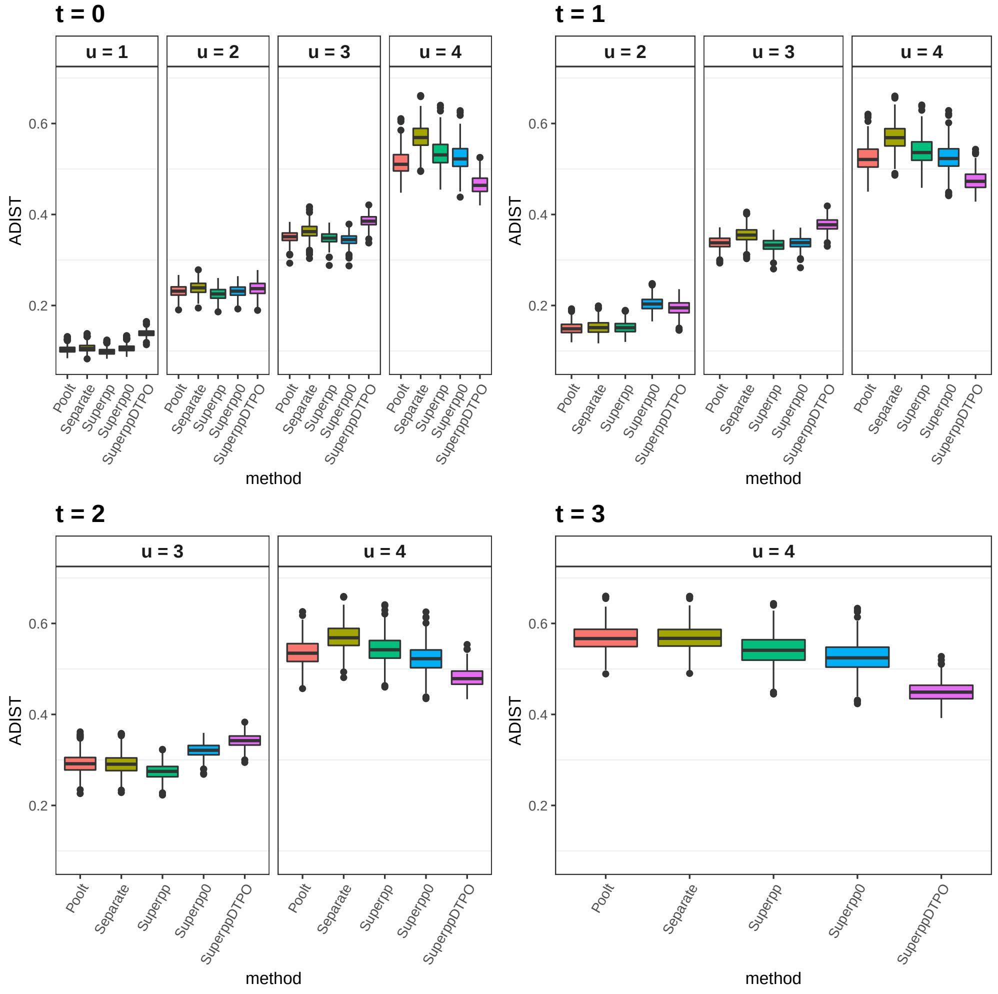


**Figure S1.16:** Simulation results comparing the distribution of ADIST on test sets across methods for each pair of $(t, u)$, trained on sample data of size 1000, 50% censoring rate, generated following a Weibull distribution with an interaction survival relationship under the scenario 2TI + 4TV, high signal-to-noise ratio and strong autocorrelation. The number of periods $T = 4$.

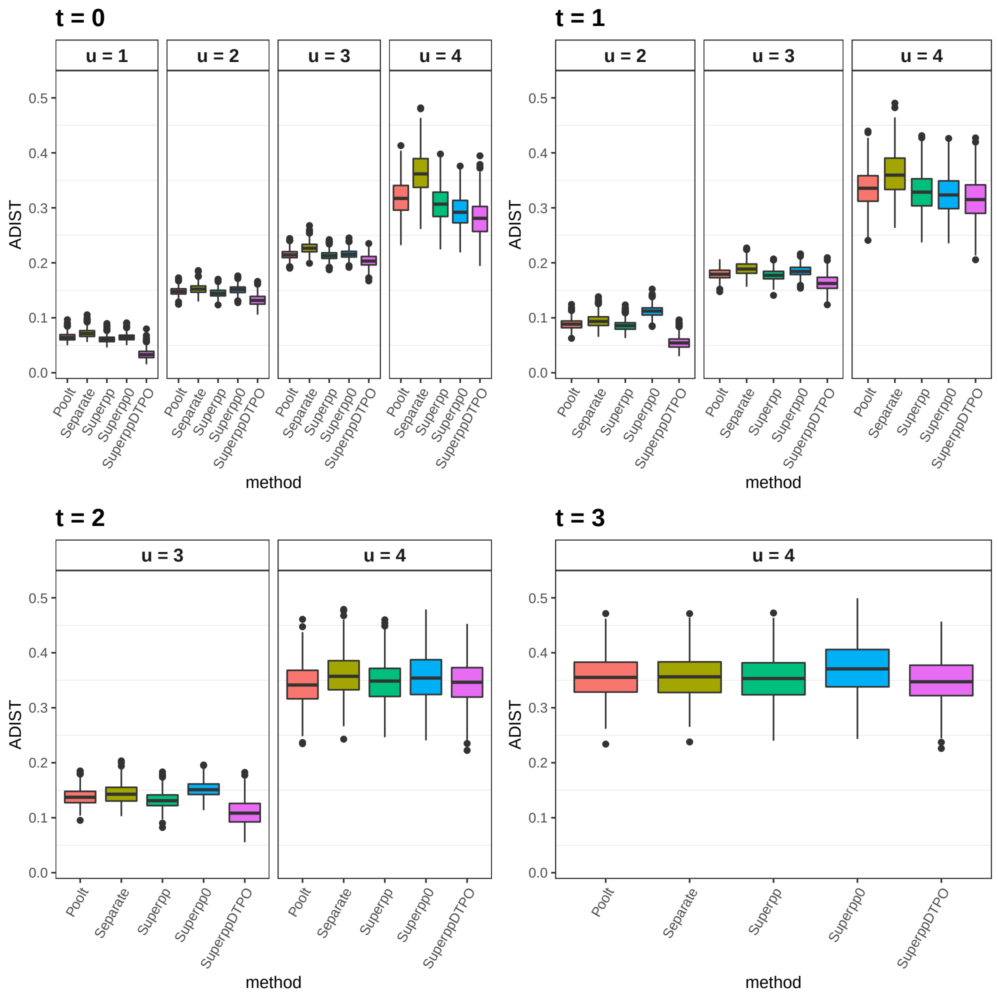


**Figure S1.17:** Simulation results comparing the distribution of ADIST on test sets across methods for each pair of $(t, u)$, trained on sample data of size 1000, 50% censoring rate, generated following a Weibull distribution with a linear survival relationship under the scenario 2TI + 4TV, low signal-to-noise ratio and strong autocorrelation. The number of periods $T = 4$.

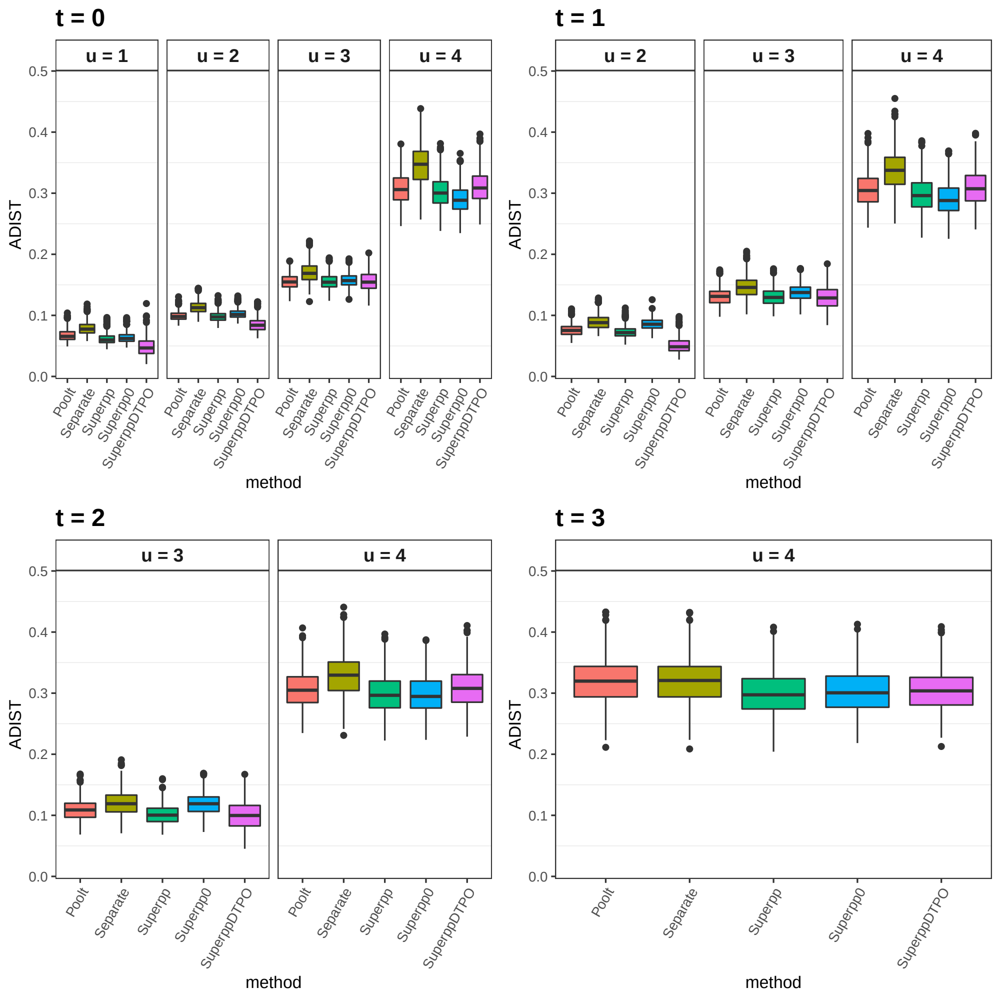


**Figure S1.18:** Simulation results comparing the distribution of ADIST on test sets across methods for each pair of $(t, u)$, trained on sample data of size 1000, 50% censoring rate, generated following a Weibull distribution with a nonlinear survival relationship under the scenario 2TI + 4TV, low signal-to-noise ratio and strong autocorrelation. The number of periods $T = 4$.

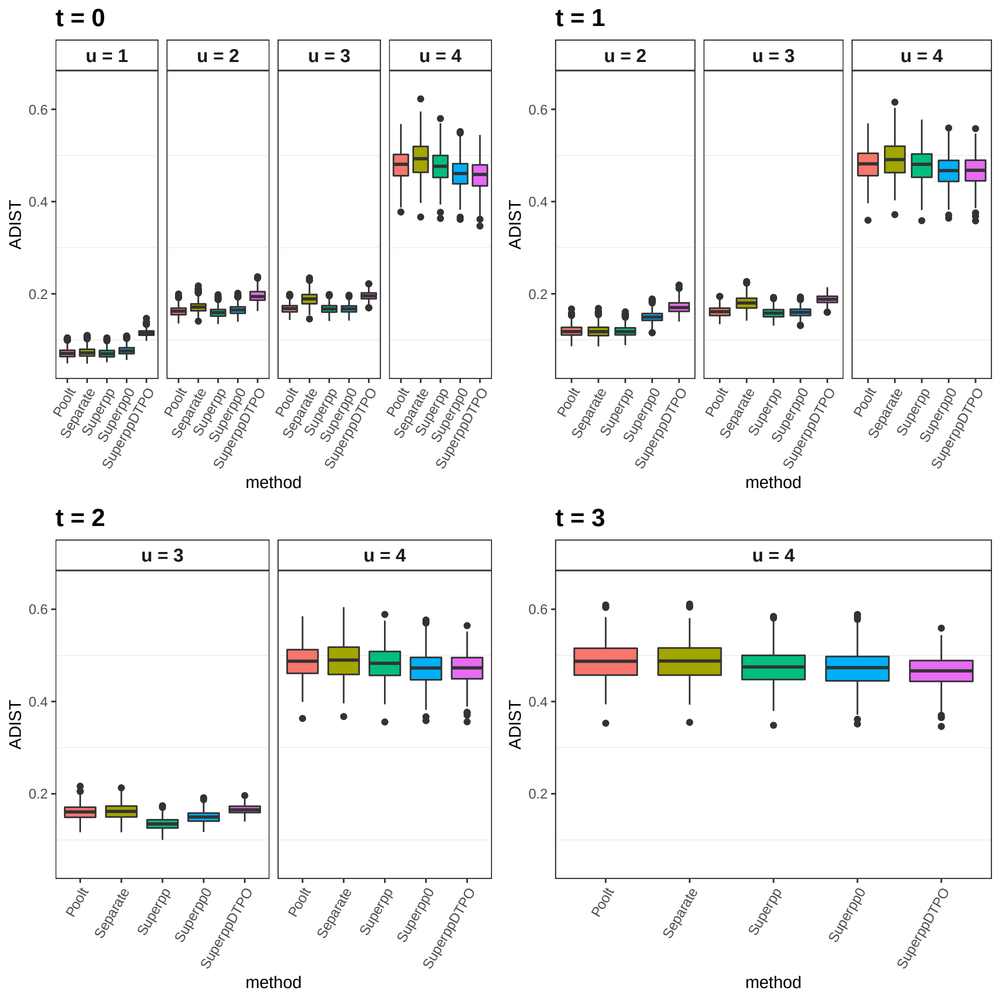


**Figure S1.19:** Simulation results comparing the distribution of ADIST on test sets across methods for each pair of $(t, u)$, trained on sample data of size 1000, 50% censoring rate, generated following a Weibull distribution with an interaction survival relationship under the scenario 2TI + 4TV, low signal-to-noise ratio and strong autocorrelation. The number of periods $T = 4$.

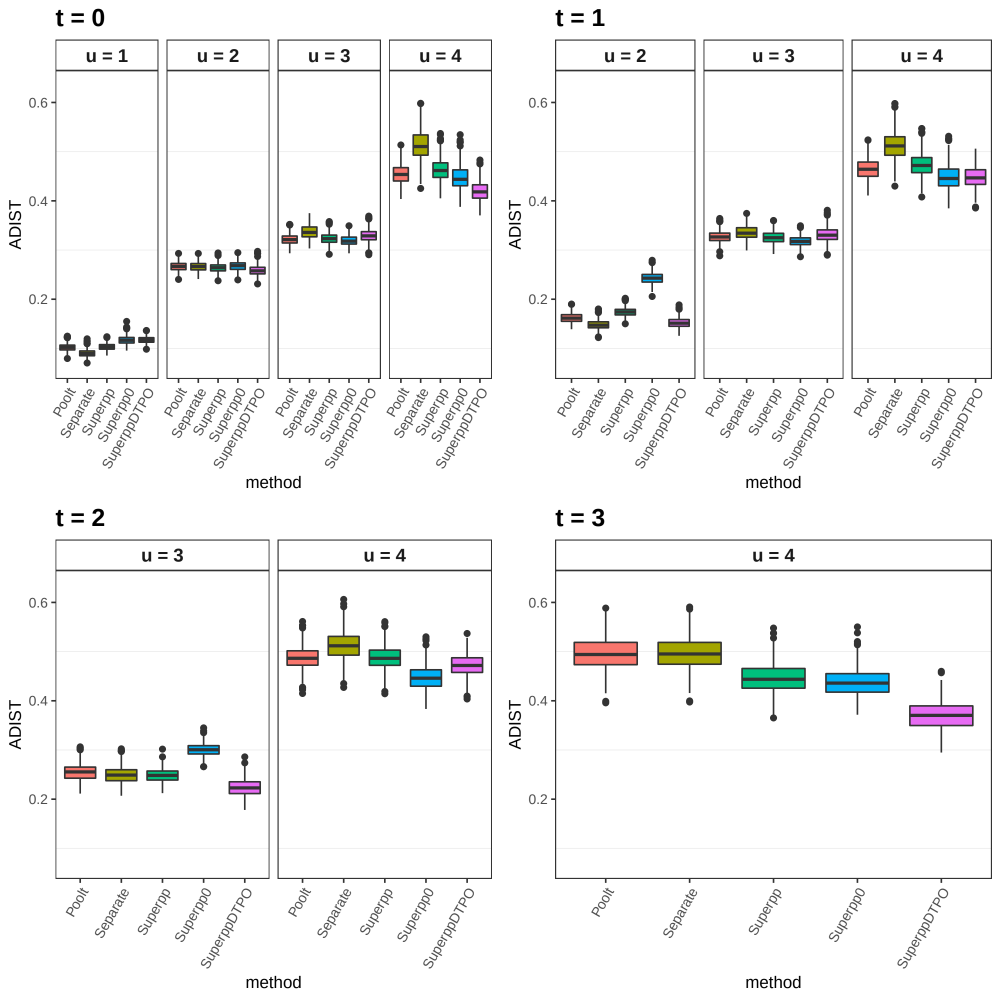


**Figure S1.20:** Simulation results comparing the distribution of ADIST on test sets across methods for each pair of $(t, u)$, trained on sample data of size 1000, 50% censoring rate, generated following a Weibull distribution with a linear survival relationship under the scenario 2TI + 4TV, high signal-to-noise ratio and weak autocorrelation. The number of periods $T = 4$.

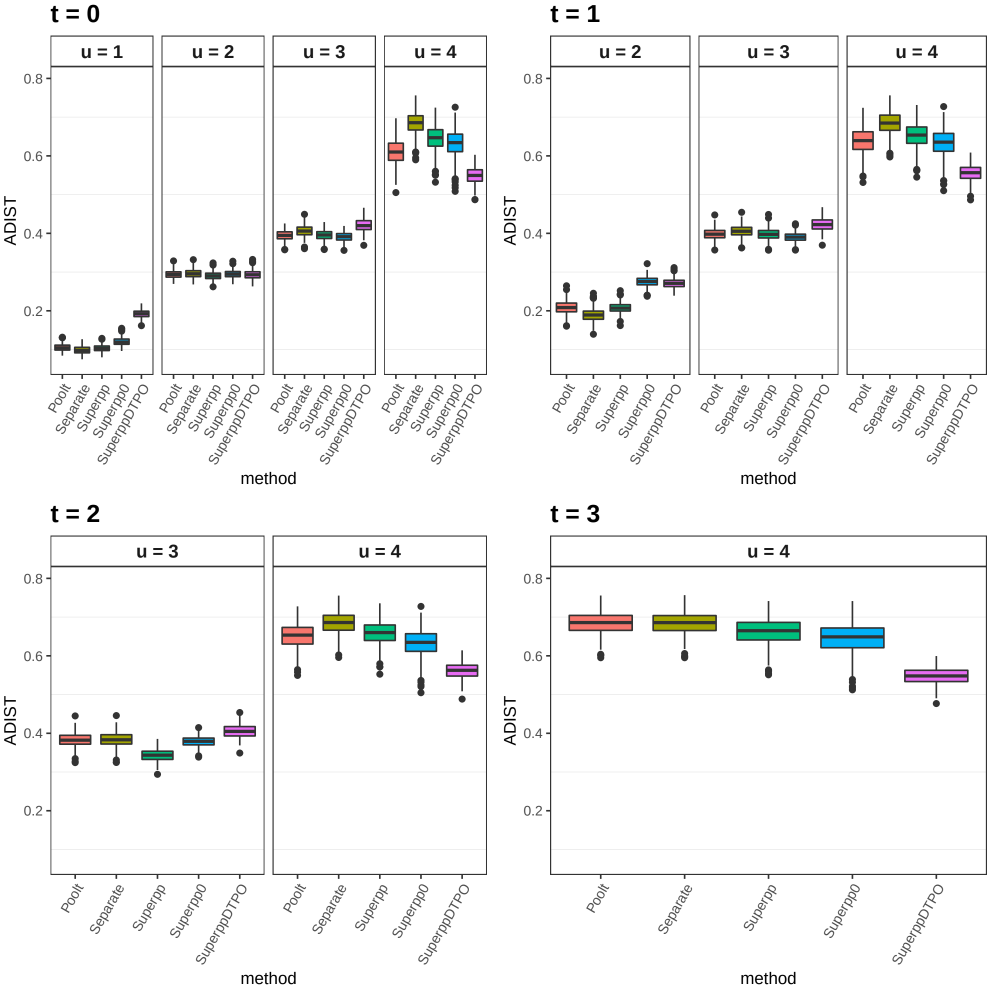


**Figure S1.21:** Simulation results comparing the distribution of ADIST on test sets across methods for each pair of $(t, u)$, trained on sample data of size 1000, 50% censoring rate, generated following a Weibull distribution with a nonlinear survival relationship under the scenario 2TI + 4TV, high signal-to-noise ratio and weak autocorrelation. The number of periods $T = 4$.

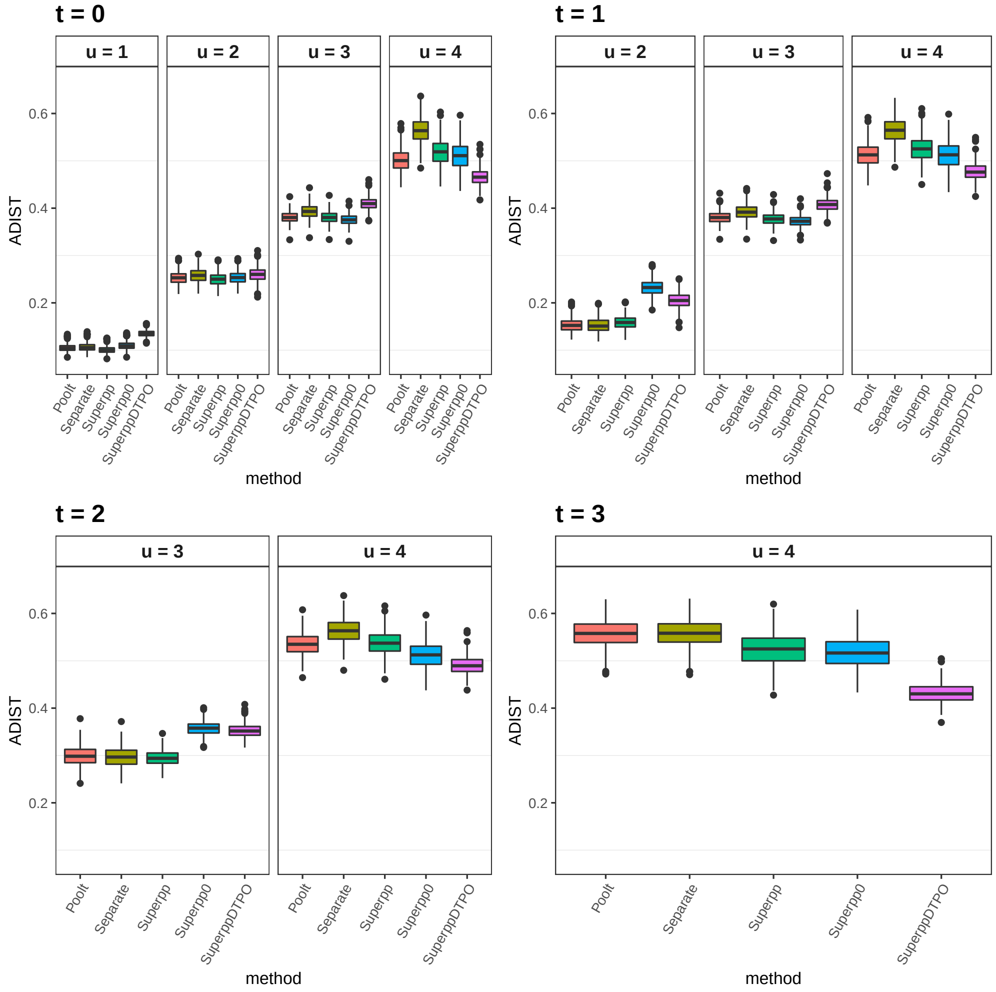


**Figure S1.22:** Simulation results comparing the distribution of ADIST on test sets across methods for each pair of $(t, u)$, trained on sample data of size 1000, 50% censoring rate, generated following a Weibull distribution with an interaction survival relationship under the scenario 2TI + 4TV, high signal-to-noise ratio and weak autocorrelation. The number of periods $T = 4$.

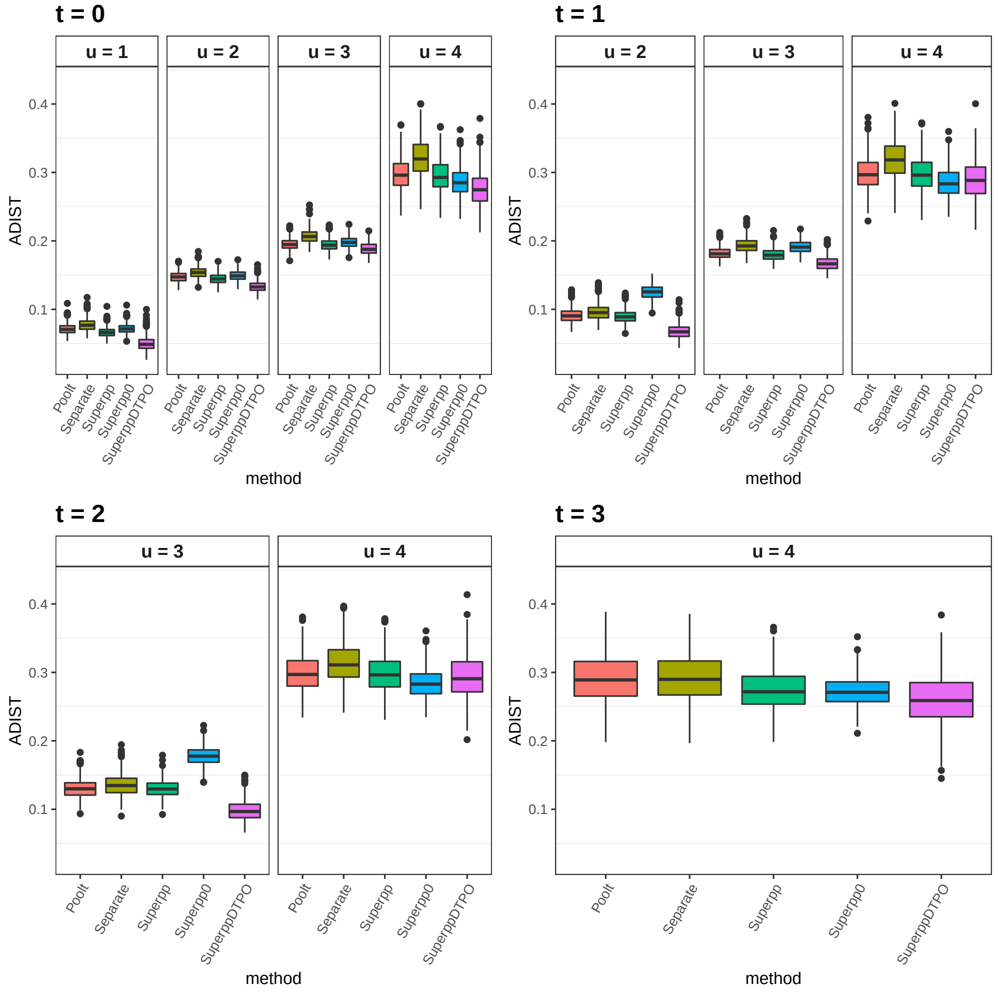


**Figure S1.23:** Simulation results comparing the distribution of ADIST on test sets across methods for each pair of $(t, u)$, trained on sample data of size 1000, 50% censoring rate, generated following a Weibull distribution with a linear survival relationship under the scenario 2TI + 4TV, low signal-to-noise ratio and weak autocorrelation. The number of periods $T = 4$.

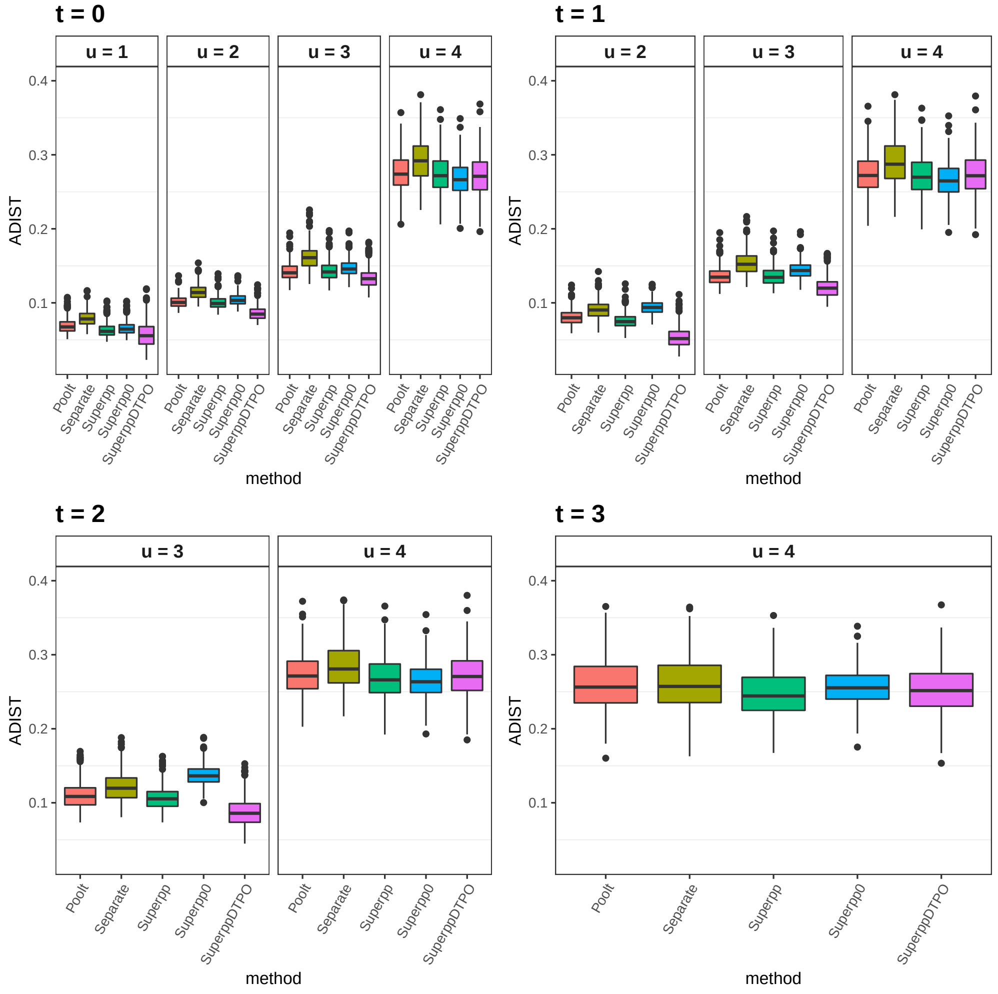


**Figure S1.24:** Simulation results comparing the distribution of ADIST on test sets across methods for each pair of $(t, u)$, trained on sample data of size 1000, 50% censoring rate, generated following a Weibull distribution with a nonlinear survival relationship under the scenario 2TI + 4TV, low signal-to-noise ratio and weak autocorrelation. The number of periods $T = 4$.

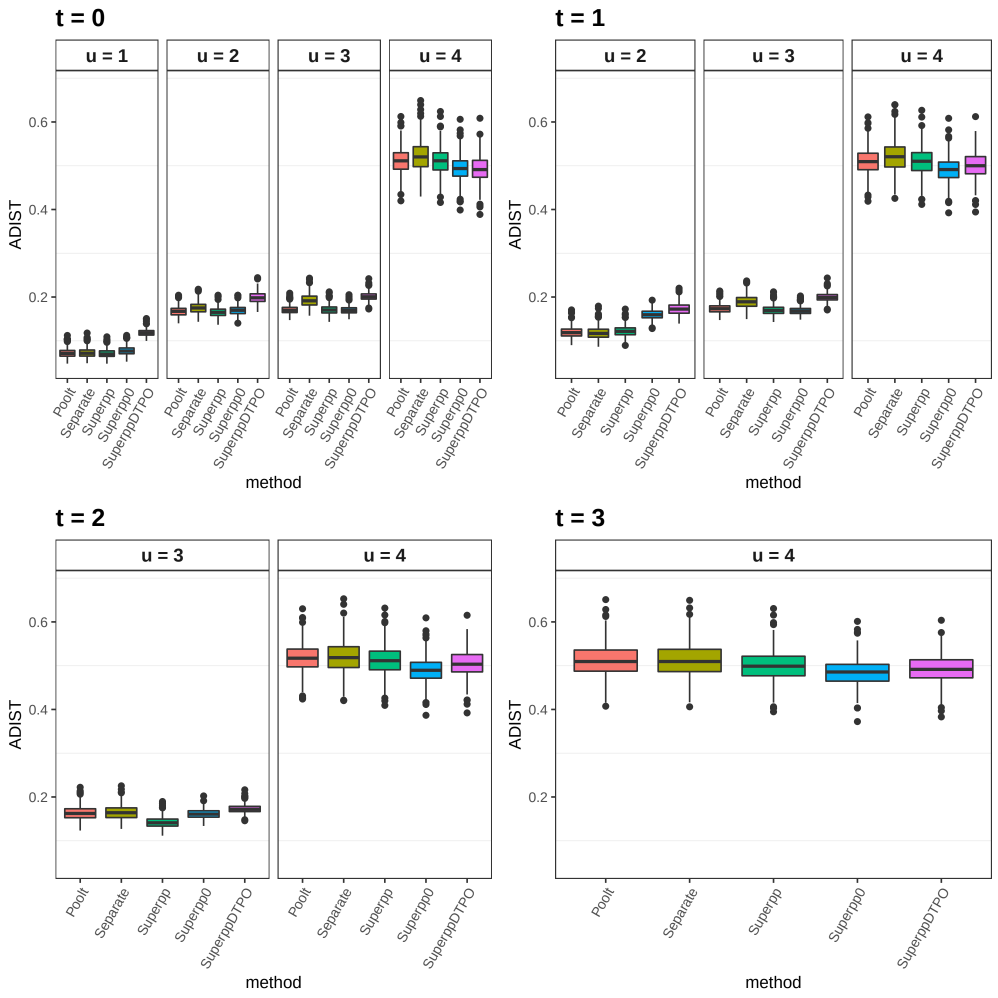


**Figure S1.25:** Simulation results comparing the distribution of ADIST on test sets across methods for each pair of $(t, u)$, trained on sample data of size 1000, 50% censoring rate, generated following a Weibull distribution with an interaction survival relationship under the scenario 2TI + 4TV, low signal-to-noise ratio and weak autocorrelation. The number of periods $T = 4$.

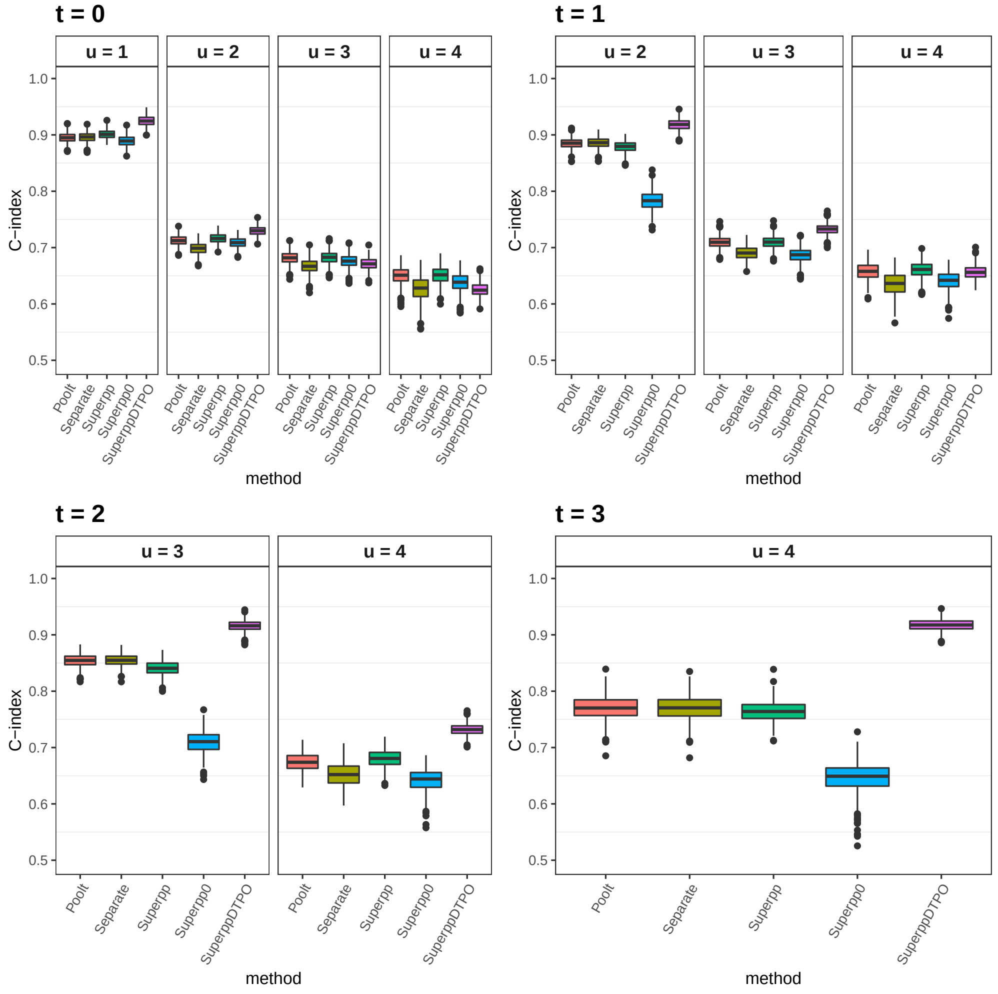


**Figure S1.26:** Simulation results comparing the distribution of C-index on test sets across methods for each pair of $(t, u)$, trained on sample data of size 1000, 10% censoring rate, generated following a Weibull distribution with a linear survival relationship under the scenario 2TI + 4TV, high signal-to-noise ratio and strong autocorrelation. The number of periods $T = 4$.

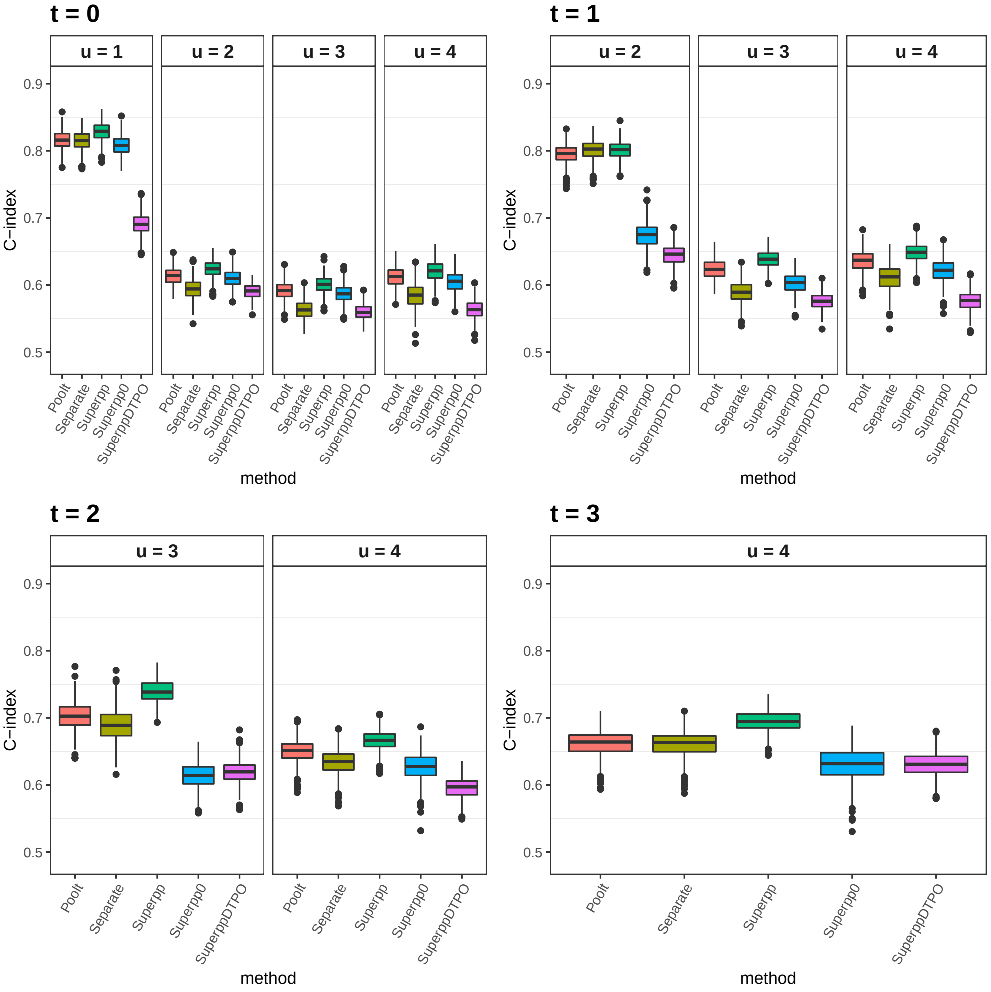


**Figure S1.27:** Simulation results comparing the distribution of C-index on test sets across methods for each pair of $(t, u)$, trained on sample data of size 1000, 10% censoring rate, generated following a Weibull distribution with a nonlinear survival relationship under the scenario 2TI + 4TV, high signal-to-noise ratio and strong autocorrelation. The number of periods $T = 4$.

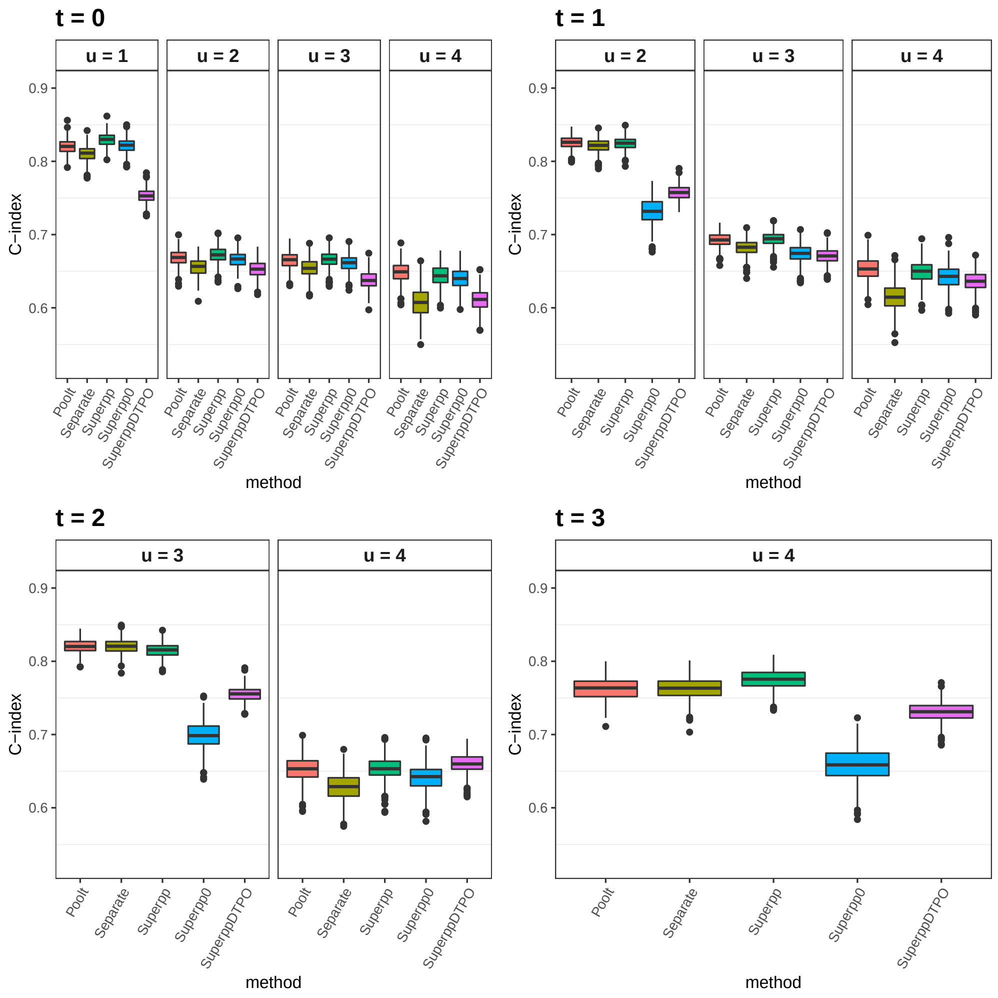


**Figure S1.28:** Simulation results comparing the distribution of C-index on test sets across methods for each pair of $(t, u)$, trained on sample data of size 1000, 10% censoring rate, generated following a Weibull distribution with an interaction survival relationship under the scenario 2TI + 4TV, high signal-to-noise ratio and strong autocorrelation. The number of periods $T = 4$.

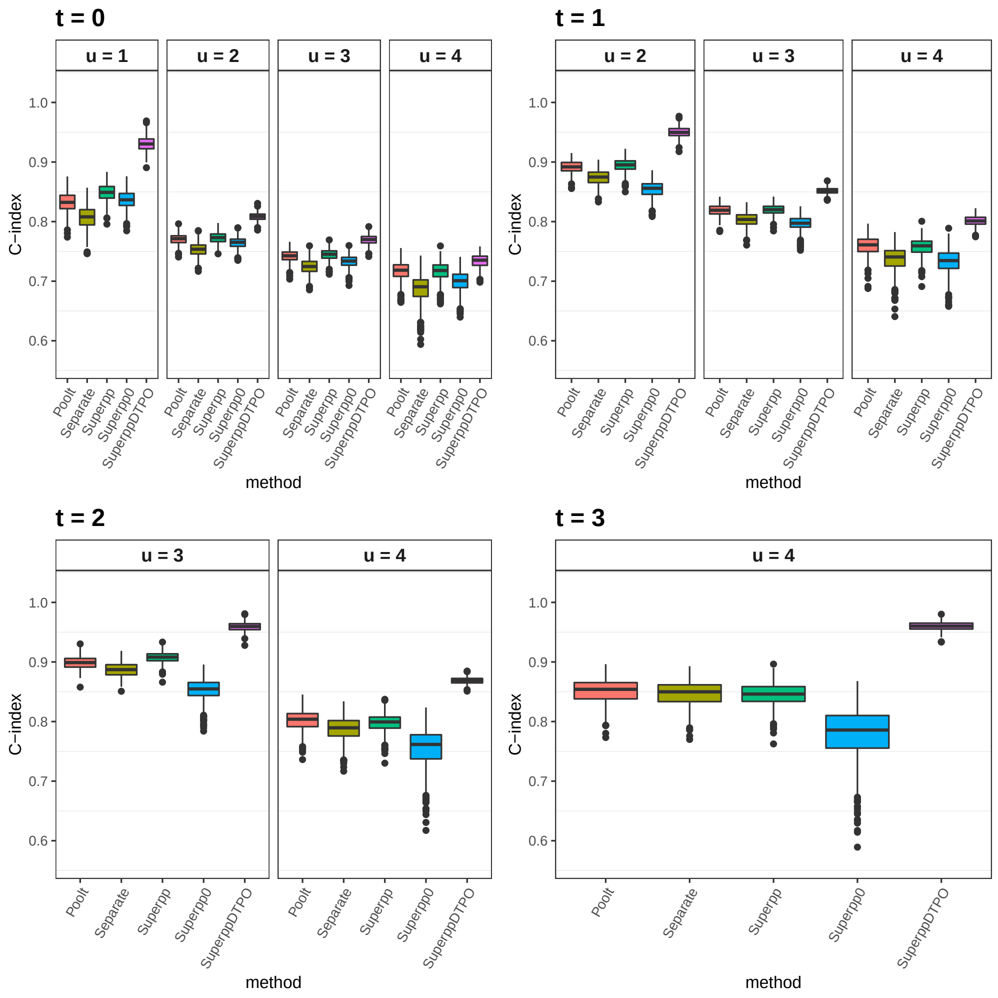


**Figure S1.29:** Simulation results comparing the distribution of C-index on test sets across methods for each pair of $(t, u)$, trained on sample data of size 1000, 10% censoring rate, generated following a Weibull distribution with a linear survival relationship under the scenario 2TI + 4TV, low signal-to-noise ratio and strong autocorrelation. The number of periods $T = 4$.

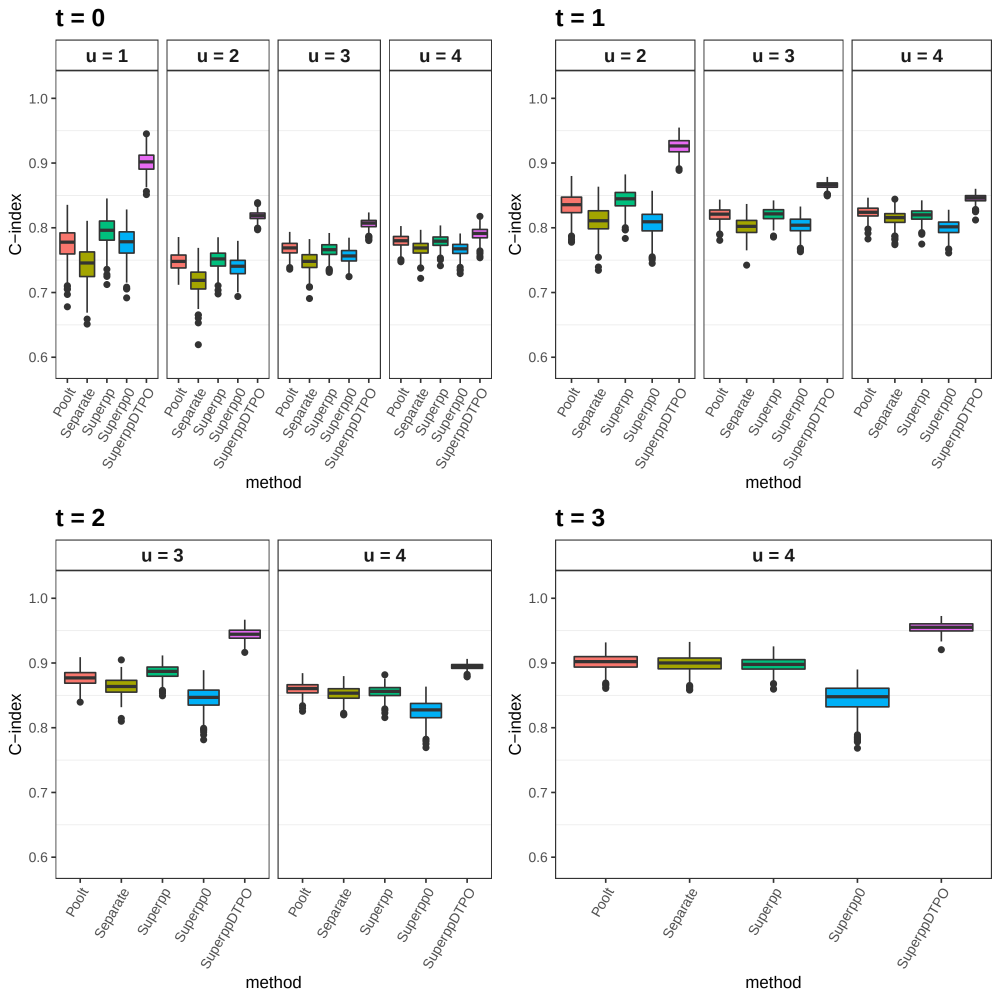


**Figure S1.30:** Simulation results comparing the distribution of C-index on test sets across methods for each pair of $(t, u)$, trained on sample data of size 1000, 10% censoring rate, generated following a Weibull distribution with a nonlinear survival relationship under the scenario 2TI + 4TV, low signal-to-noise ratio and strong autocorrelation. The number of periods $T = 4$.

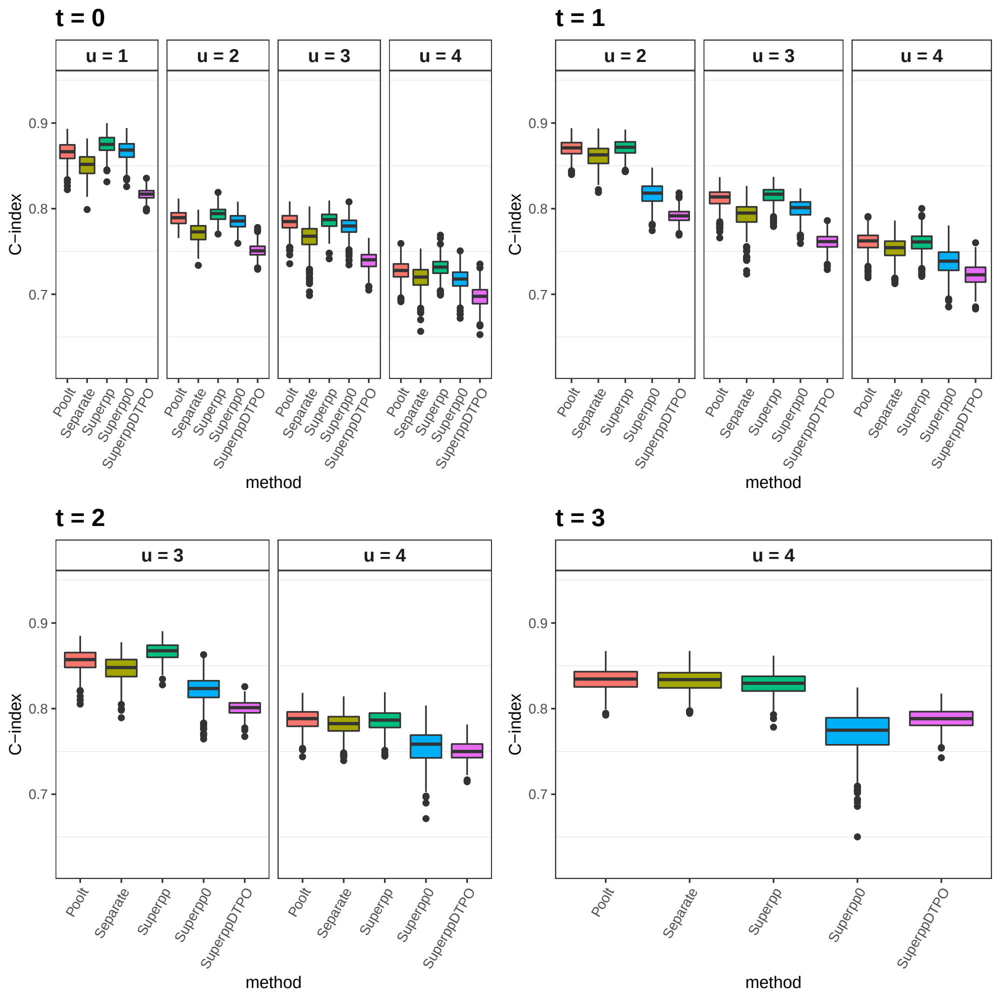


**Figure S1.31:** Simulation results comparing the distribution of C-index on test sets across methods for each pair of $(t, u)$, trained on sample data of size 1000, 10% censoring rate, generated following a Weibull distribution with an interaction survival relationship under the scenario 2TI + 4TV, low signal-to-noise ratio and strong autocorrelation. The number of periods $T = 4$.

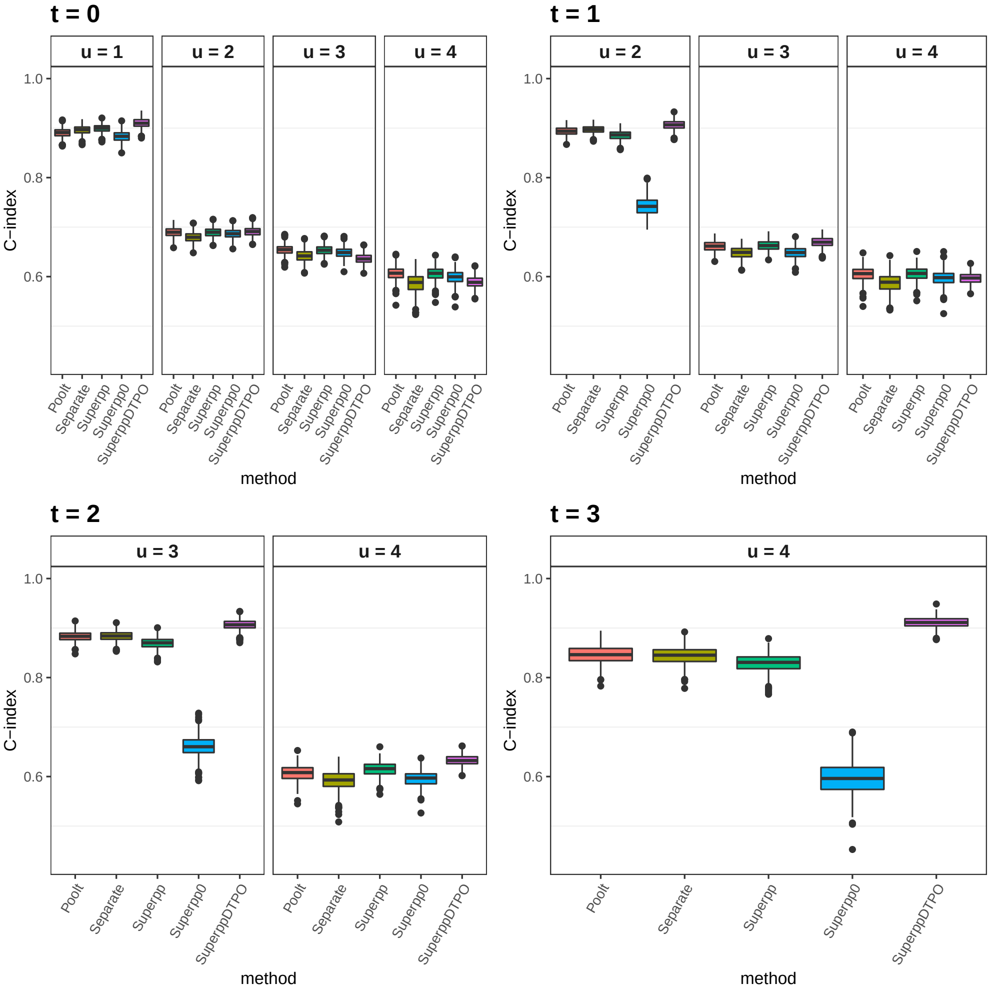


**Figure S1.32:** Simulation results comparing the distribution of C-index on test sets across methods for each pair of $(t, u)$, trained on sample data of size 1000, 10% censoring rate, generated following a Weibull distribution with a linear survival relationship under the scenario 2TI + 4TV, high signal-to-noise ratio and weak autocorrelation. The number of periods $T = 4$.

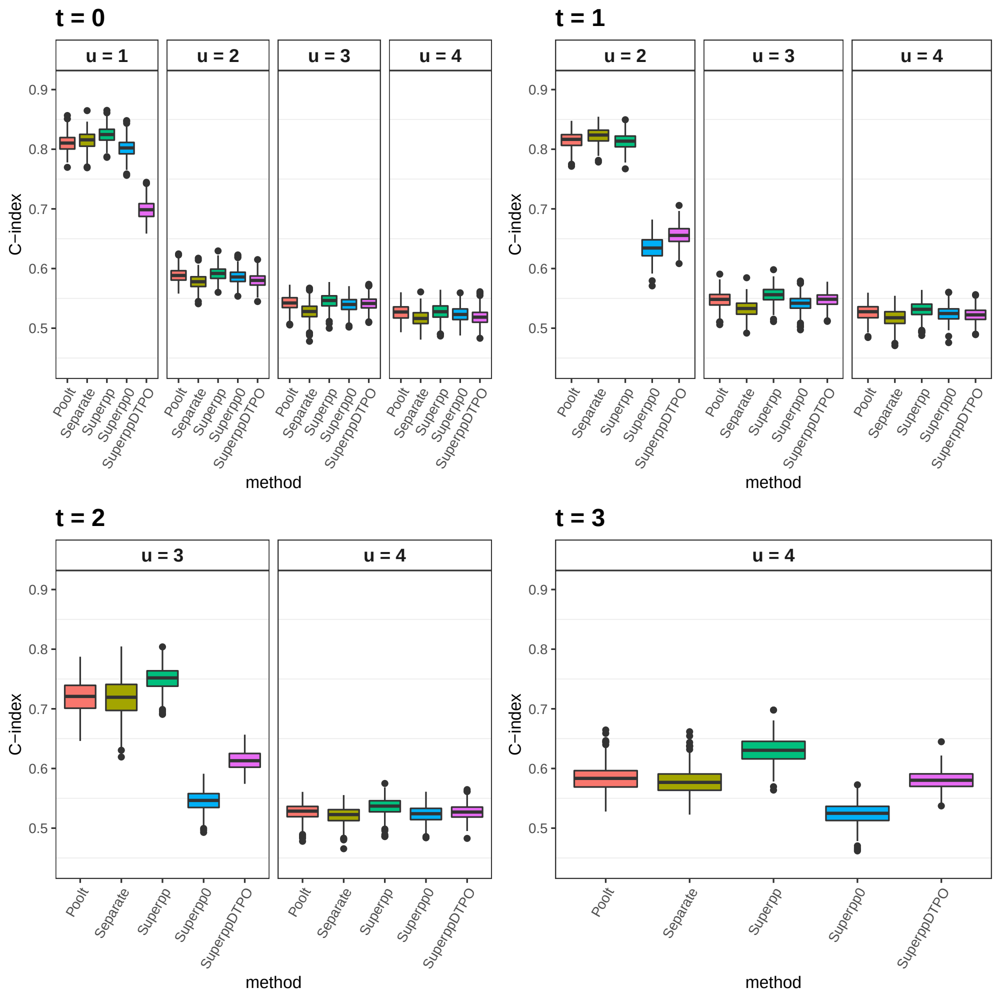


**Figure S1.33:** Simulation results comparing the distribution of C-index on test sets across methods for each pair of $(t, u)$, trained on sample data of size 1000, 10% censoring rate, generated following a Weibull distribution with a nonlinear survival relationship under the scenario 2TI + 4TV, high signal-to-noise ratio and weak autocorrelation. The number of periods $T = 4$.

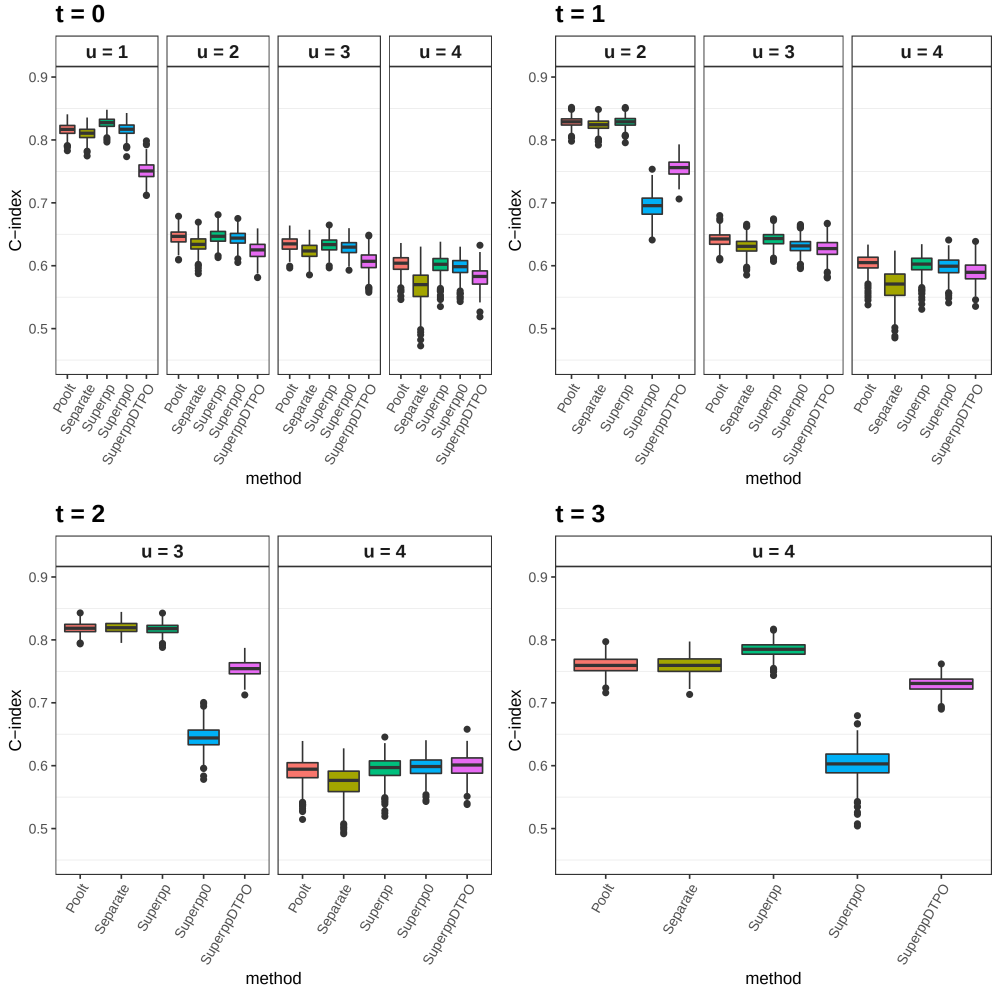


**Figure S1.34:** Simulation results comparing the distribution of C-index on test sets across methods for each pair of $(t, u)$, trained on sample data of size 1000, 10% censoring rate, generated following a Weibull distribution with an interaction survival relationship under the scenario 2TI + 4TV, high signal-to-noise ratio and weak autocorrelation. The number of periods $T = 4$.

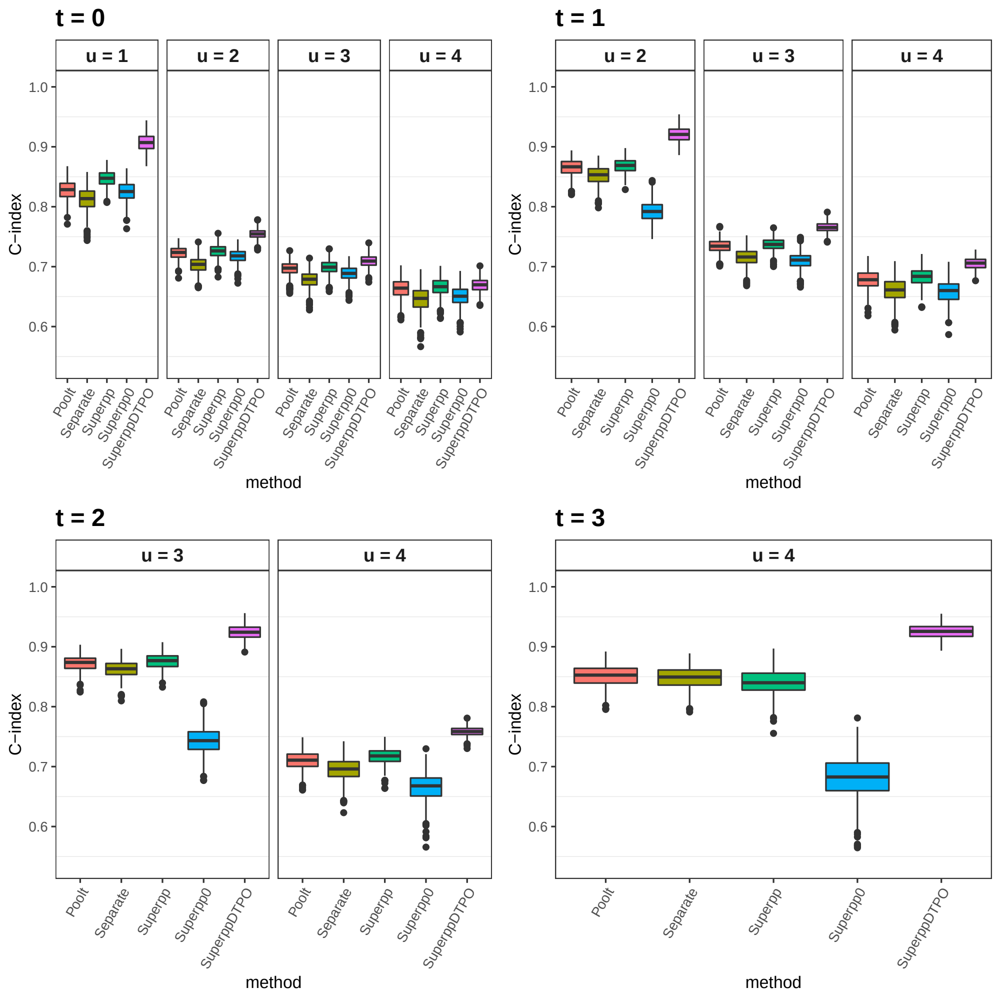


**Figure S1.35:** Simulation results comparing the distribution of C-index on test sets across methods for each pair of $(t, u)$, trained on sample data of size 1000, 10% censoring rate, generated following a Weibull distribution with a linear survival relationship under the scenario 2TI + 4TV, low signal-to-noise ratio and weak autocorrelation. The number of periods $T = 4$.

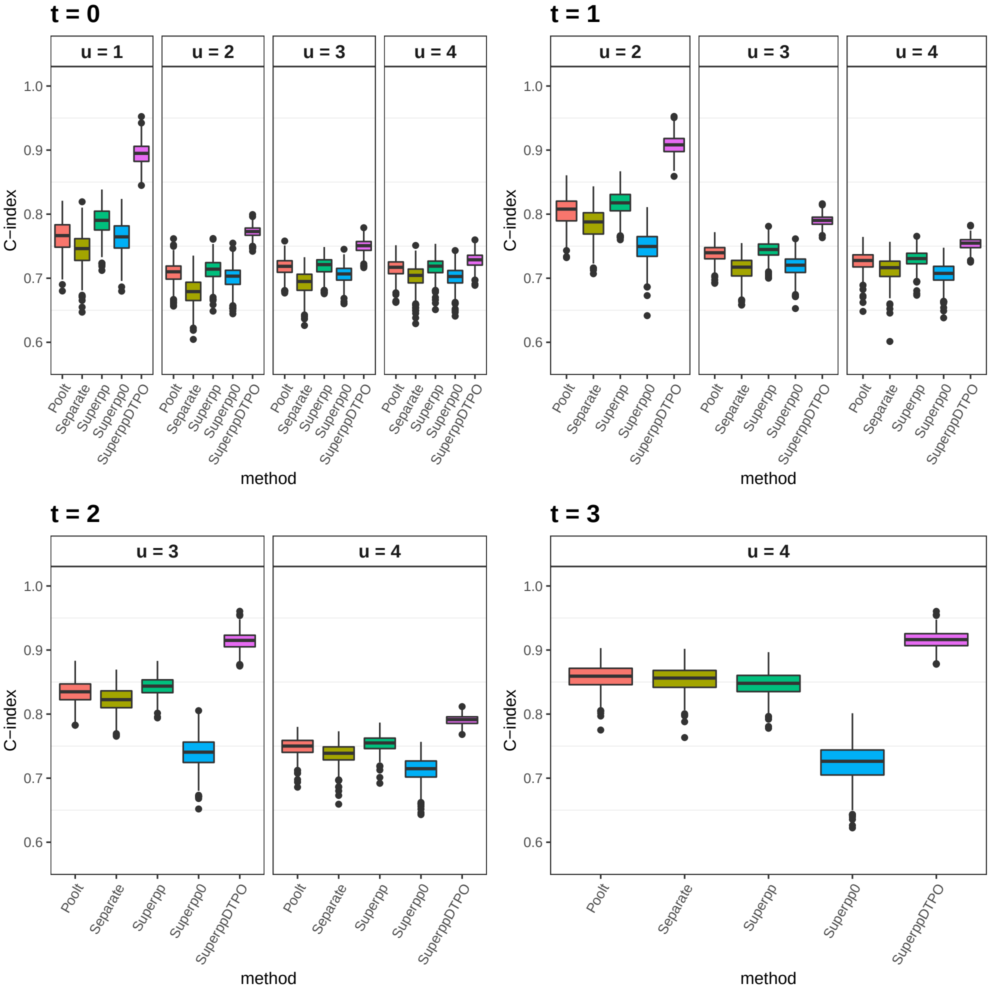


**Figure S1.36:** Simulation results comparing the distribution of C-index on test sets across methods for each pair of $(t, u)$, trained on sample data of size 1000, 10% censoring rate, generated following a Weibull distribution with a nonlinear survival relationship under the scenario 2TI + 4TV, low signal-to-noise ratio and weak autocorrelation. The number of periods $T = 4$.

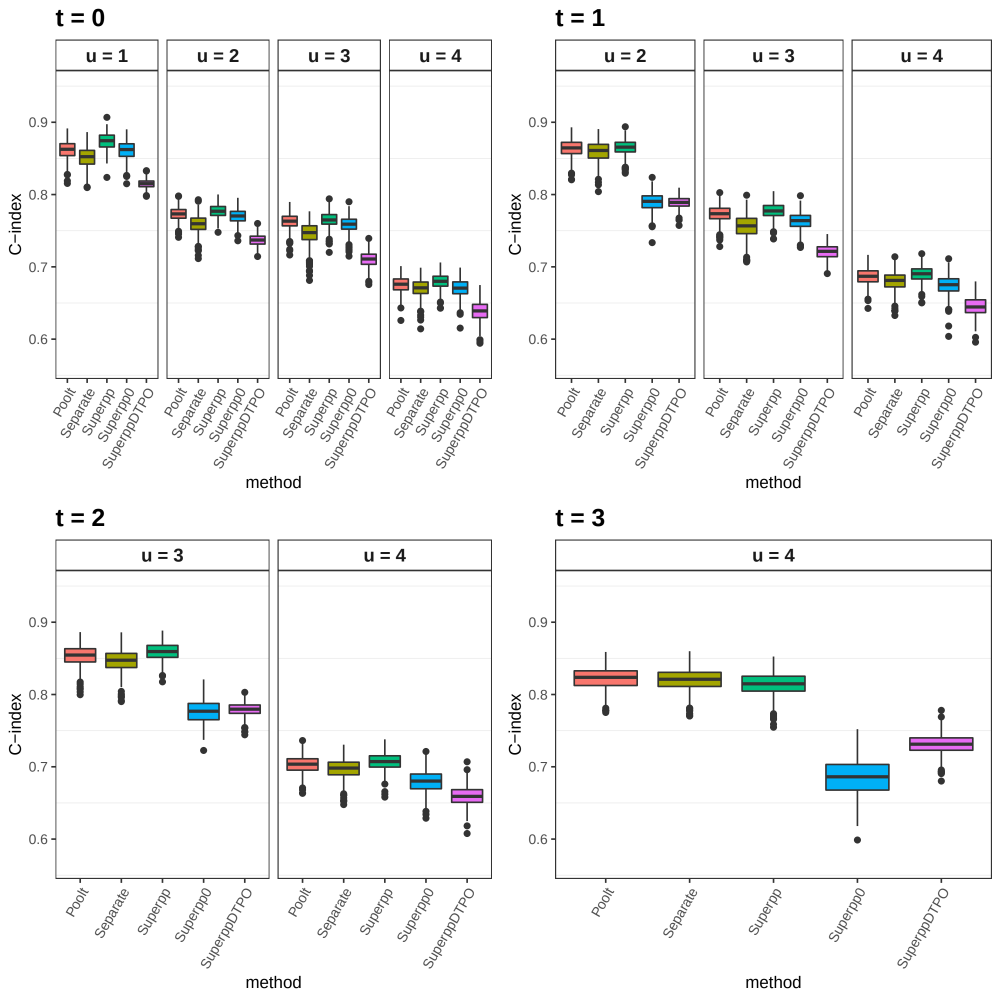


**Figure S1.37:** Simulation results comparing the distribution of C-index on test sets across methods for each pair of $(t, u)$, trained on sample data of size 1000, 10% censoring rate, generated following a Weibull distribution with an interaction survival relationship under the scenario 2TI + 4TV, low signal-to-noise ratio and weak autocorrelation. The number of periods $T = 4$.

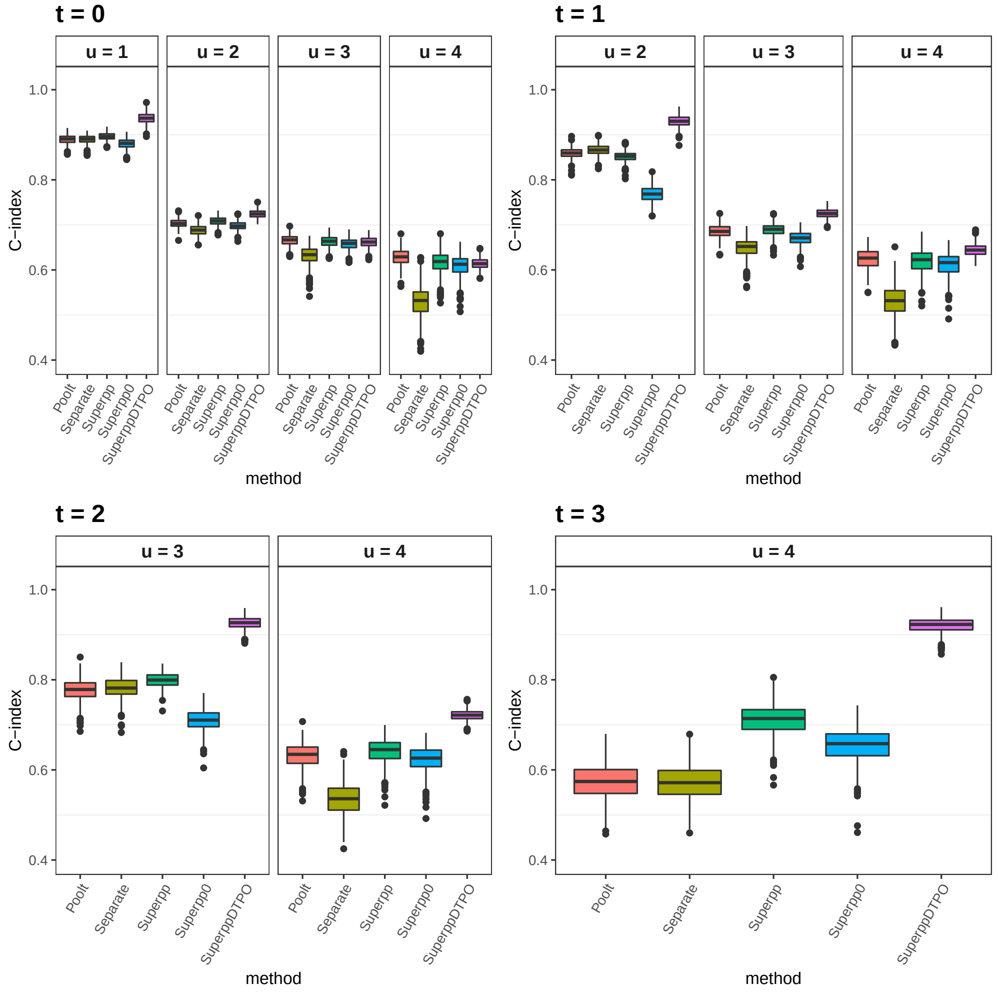


**Figure S1.38:** Simulation results comparing the distribution of C-index on test sets across methods for each pair of $(t, u)$, trained on sample data of size 1000, 50% censoring rate, generated following a Weibull distribution with a linear survival relationship under the scenario 2TI + 4TV, high signal-to-noise ratio and strong autocorrelation. The number of periods $T = 4$.

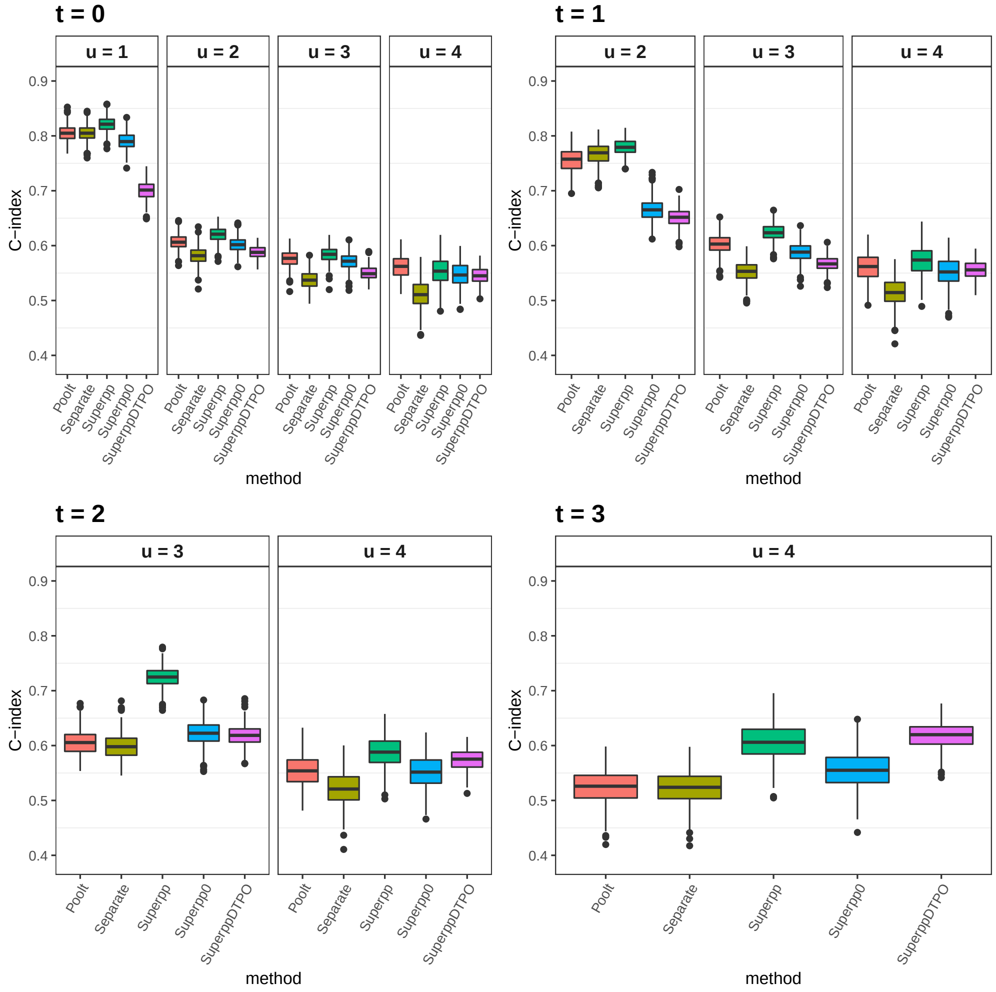


**Figure S1.39:** Simulation results comparing the distribution of C-index on test sets across methods for each pair of $(t, u)$, trained on sample data of size 1000, 50% censoring rate, generated following a Weibull distribution with a nonlinear survival relationship under the scenario 2TI + 4TV, high signal-to-noise ratio and strong autocorrelation. The number of periods $T = 4$.

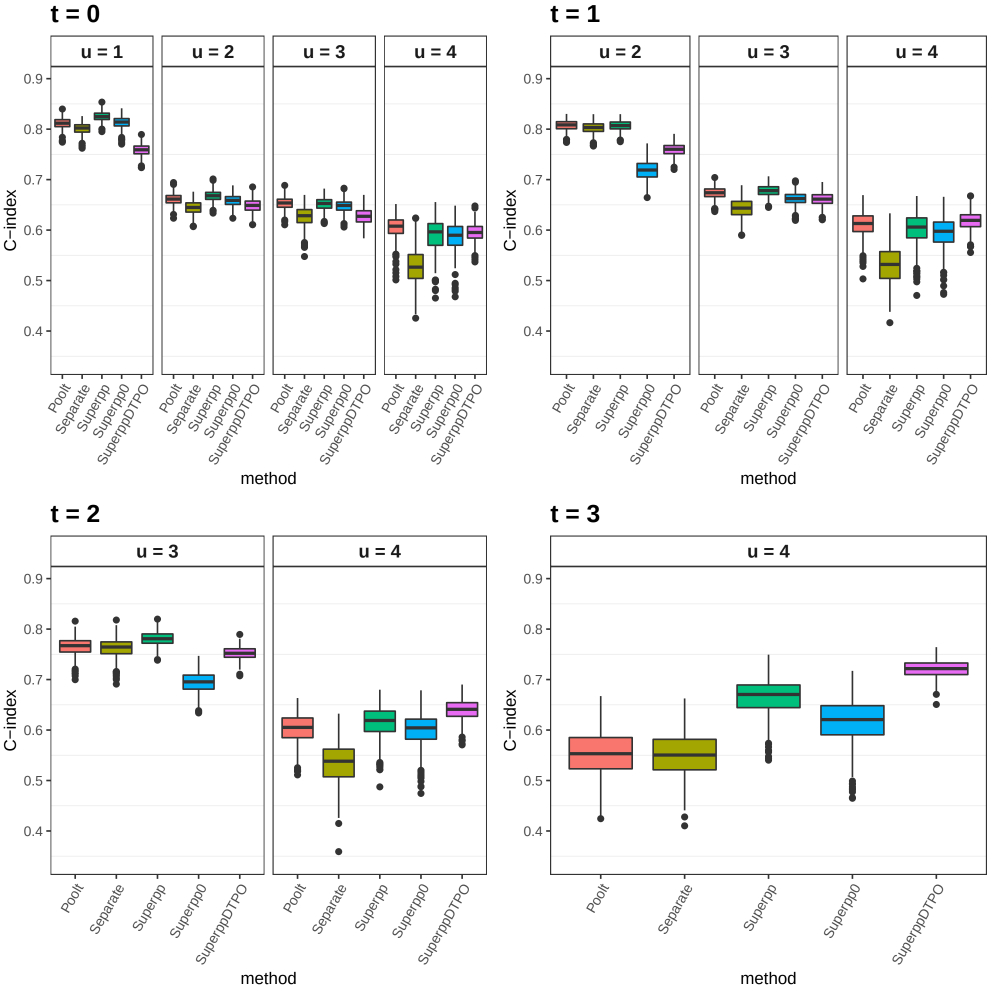


**Figure S1.40:** Simulation results comparing the distribution of C-index on test sets across methods for each pair of $(t, u)$, trained on sample data of size 1000, 50% censoring rate, generated following a Weibull distribution with an interaction survival relationship under the scenario 2TI + 4TV, high signal-to-noise ratio and strong autocorrelation. The number of periods $T = 4$.

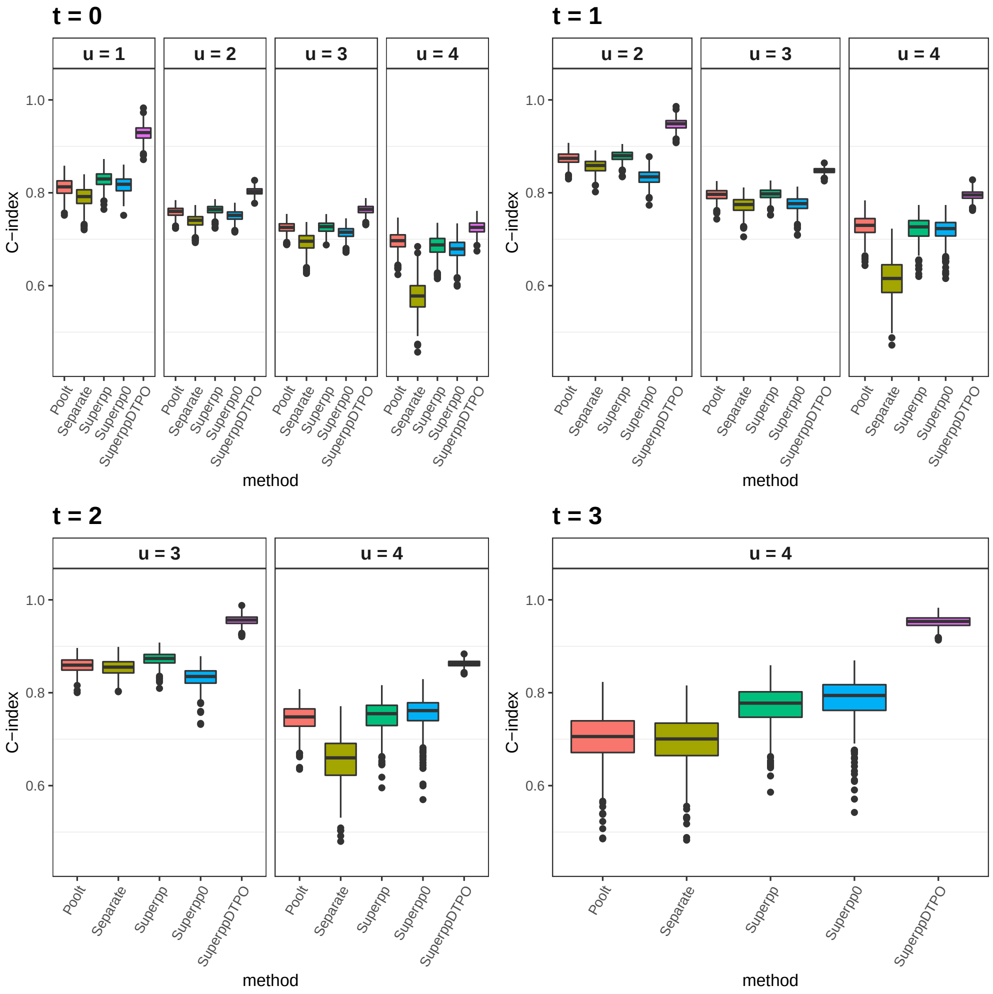


**Figure S1.41:** Simulation results comparing the distribution of C-index on test sets across methods for each pair of $(t, u)$, trained on sample data of size 1000, 50% censoring rate, generated following a Weibull distribution with a linear survival relationship under the scenario 2TI + 4TV, low signal-to-noise ratio and strong autocorrelation. The number of periods $T = 4$.

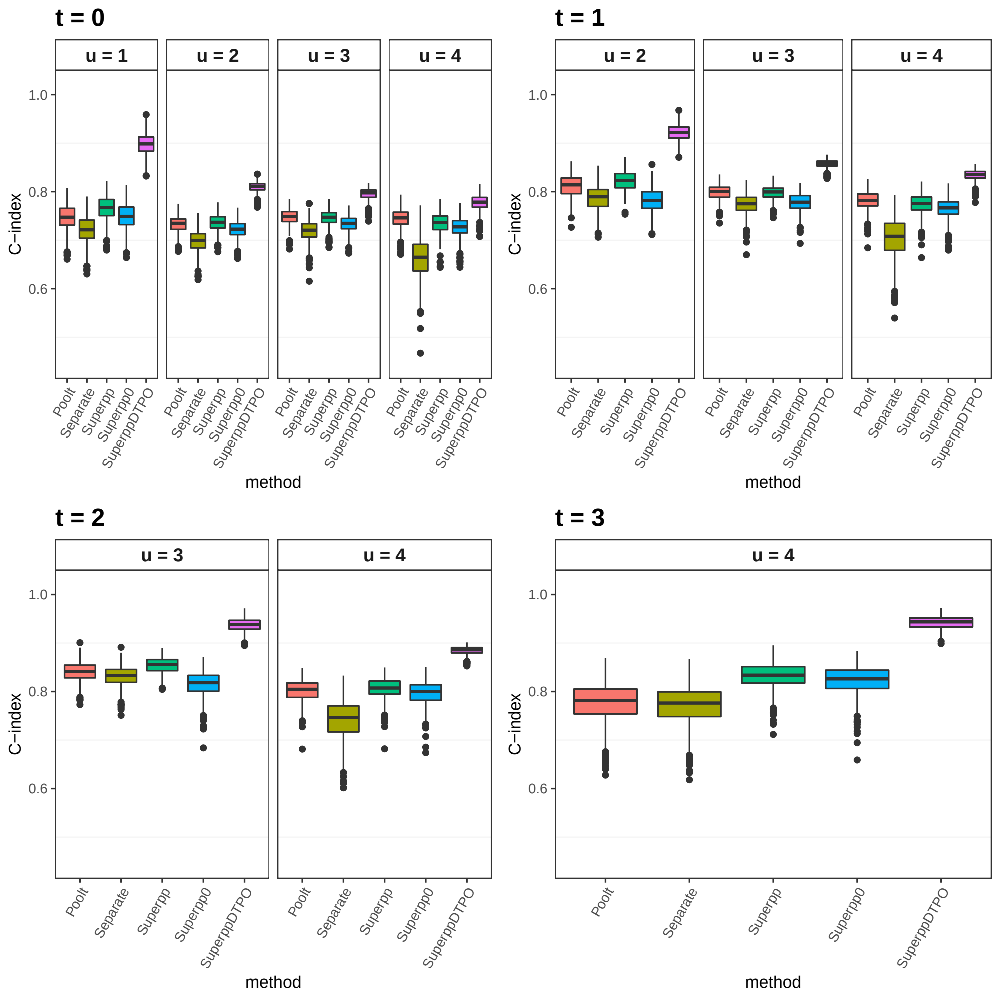


**Figure S1.42:** Simulation results comparing the distribution of C-index on test sets across methods for each pair of $(t, u)$, trained on sample data of size 1000, 50% censoring rate, generated following a Weibull distribution with a nonlinear survival relationship under the scenario 2TI + 4TV, low signal-to-noise ratio and strong autocorrelation. The number of periods $T = 4$.

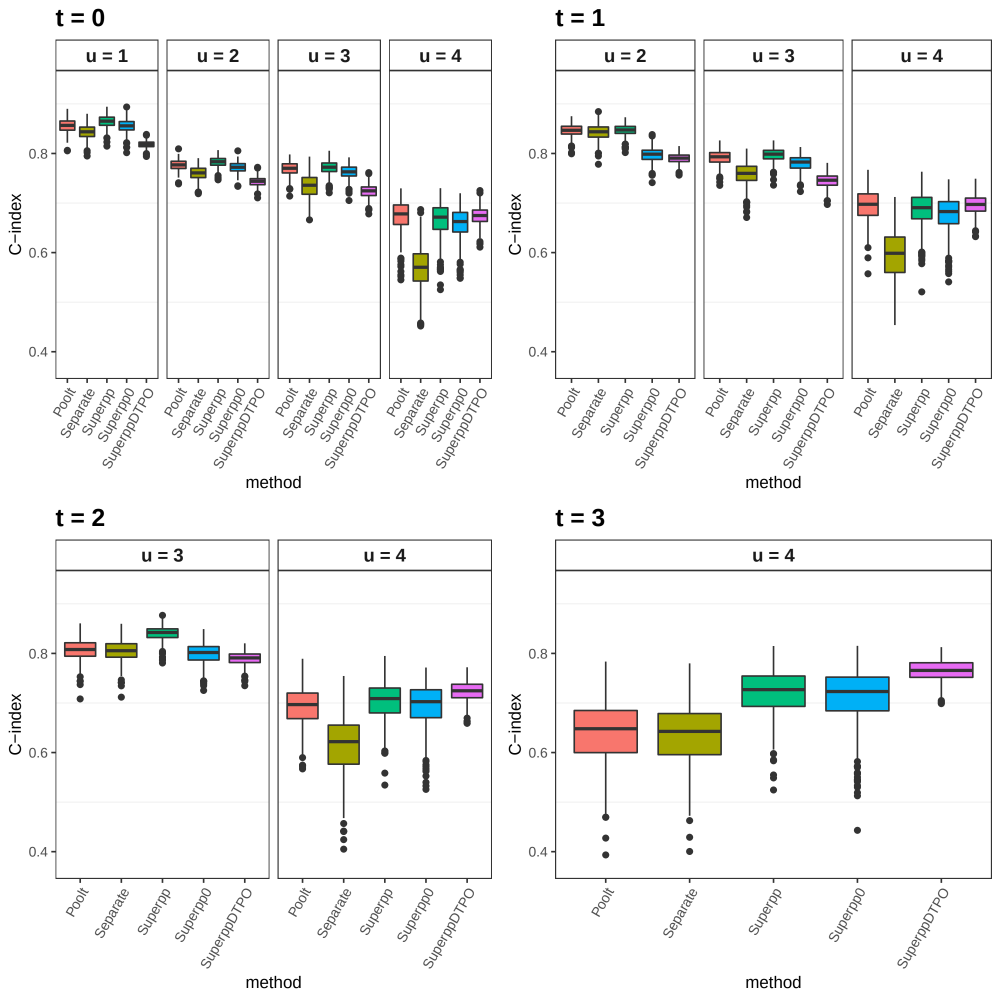


**Figure S1.43:** Simulation results comparing the distribution of C-index on test sets across methods for each pair of $(t, u)$, trained on sample data of size 1000, 50% censoring rate, generated following a Weibull distribution with an interaction survival relationship under the scenario 2TI + 4TV, low signal-to-noise ratio and strong autocorrelation. The number of periods $T = 4$.

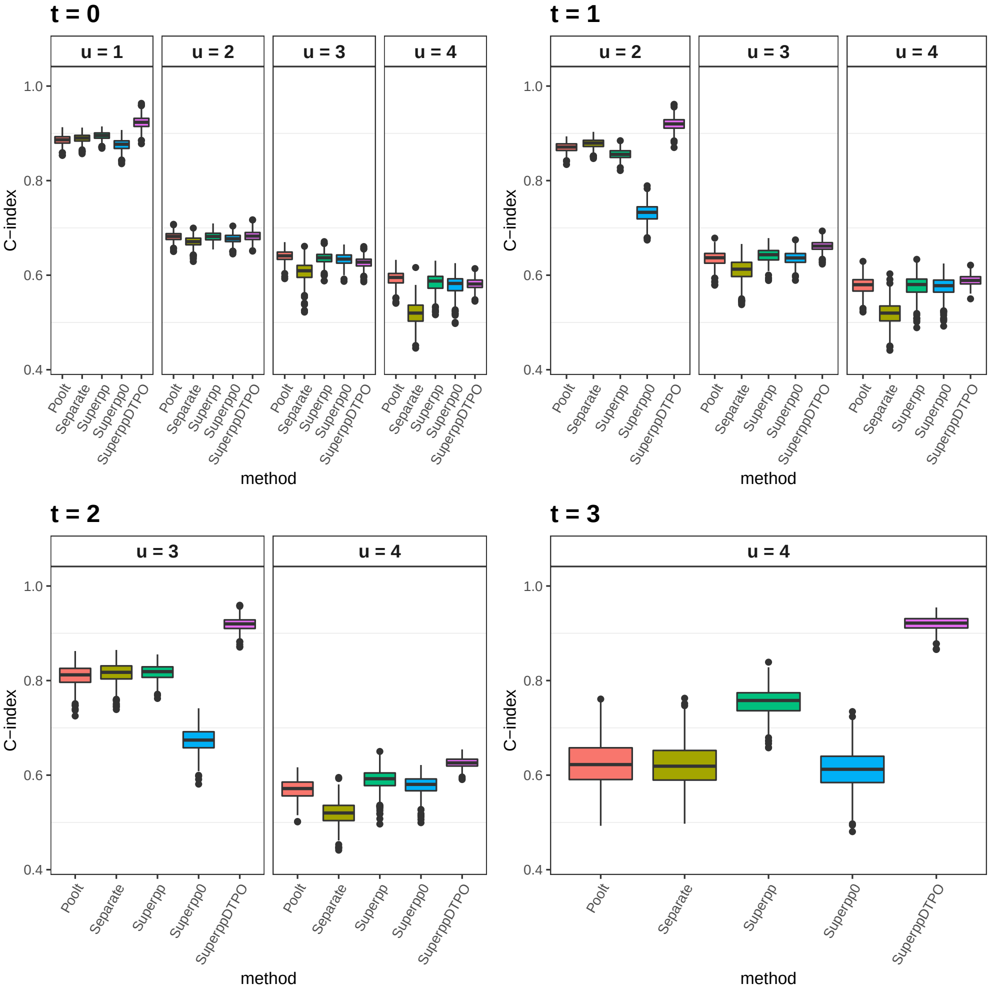


**Figure S1.44:** Simulation results comparing the distribution of C-index on test sets across methods for each pair of $(t, u)$, trained on sample data of size 1000, 50% censoring rate, generated following a Weibull distribution with a linear survival relationship under the scenario 2TI + 4TV, high signal-to-noise ratio and weak autocorrelation. The number of periods $T = 4$.

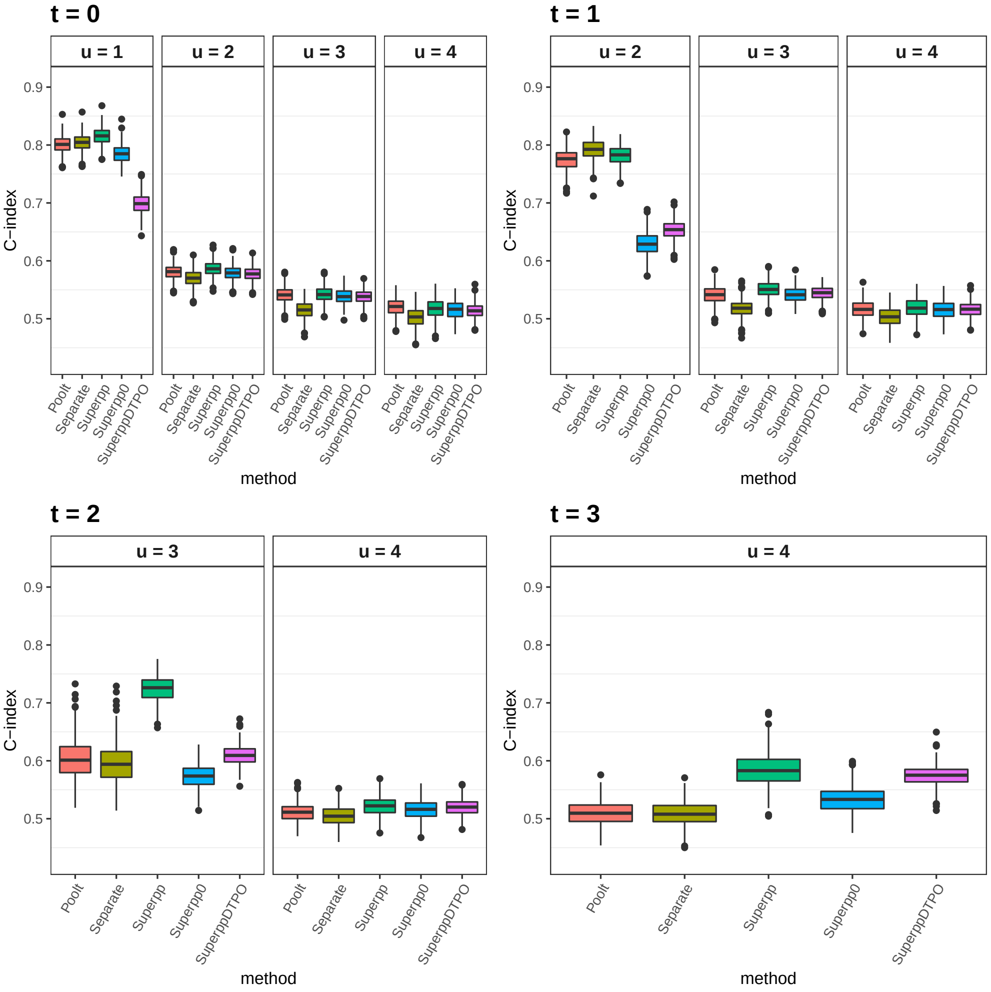


**Figure S1.45:** Simulation results comparing the distribution of C-index on test sets across methods for each pair of $(t, u)$, trained on sample data of size 1000, 50% censoring rate, generated following a Weibull distribution with a nonlinear survival relationship under the scenario 2TI + 4TV, high signal-to-noise ratio and weak autocorrelation. The number of periods $T = 4$.

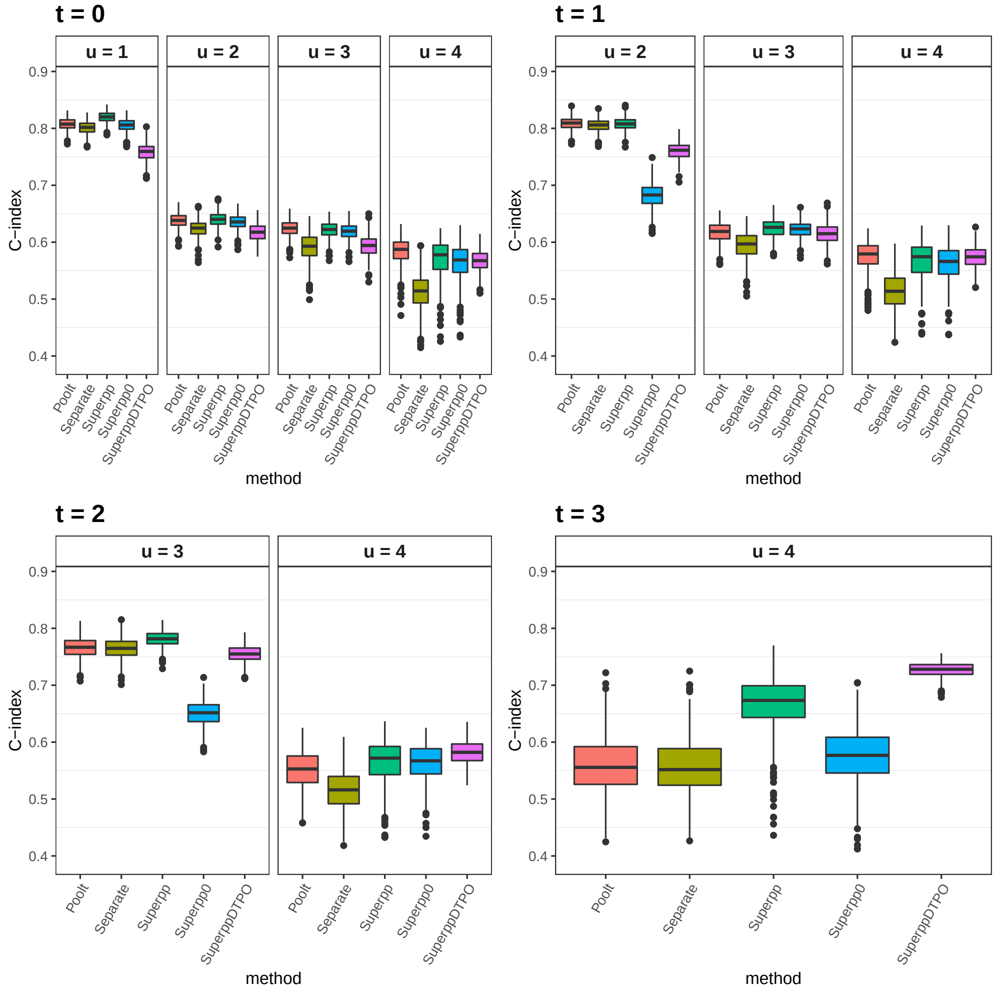


**Figure S1.46:** Simulation results comparing the distribution of C-index on test sets across methods for each pair of $(t, u)$, trained on sample data of size 1000, 50% censoring rate, generated following a Weibull distribution with an interaction survival relationship under the scenario 2TI + 4TV, high signal-to-noise ratio and weak autocorrelation. The number of periods $T = 4$.

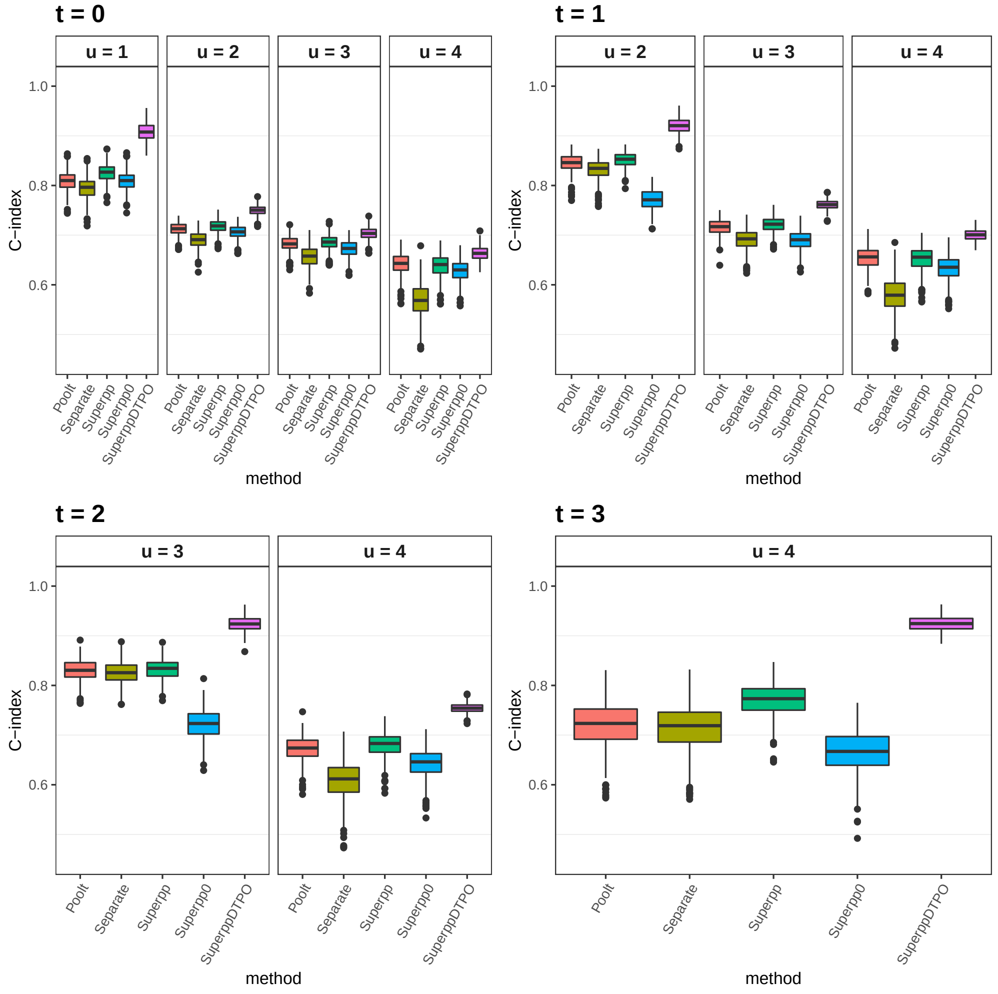


**Figure S1.47:** Simulation results comparing the distribution of C-index on test sets across methods for each pair of $(t, u)$, trained on sample data of size 1000, 50% censoring rate, generated following a Weibull distribution with a linear survival relationship under the scenario 2TI + 4TV, low signal-to-noise ratio and weak autocorrelation. The number of periods $T = 4$.

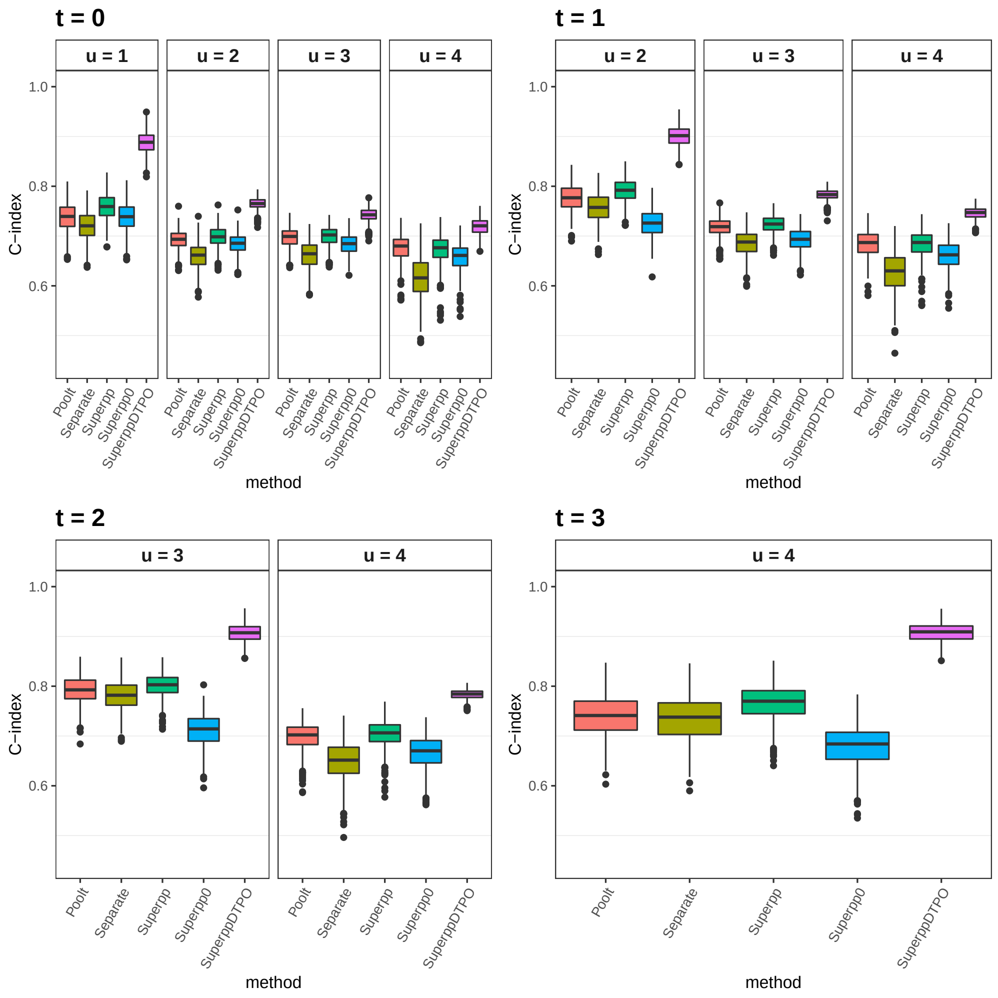


**Figure S1.48:** Simulation results comparing the distribution of C-index on test sets across methods for each pair of $(t, u)$, trained on sample data of size 1000, 50% censoring rate, generated following a Weibull distribution with a nonlinear survival relationship under the scenario 2TI + 4TV, low signal-to-noise ratio and weak autocorrelation. The number of periods $T = 4$.

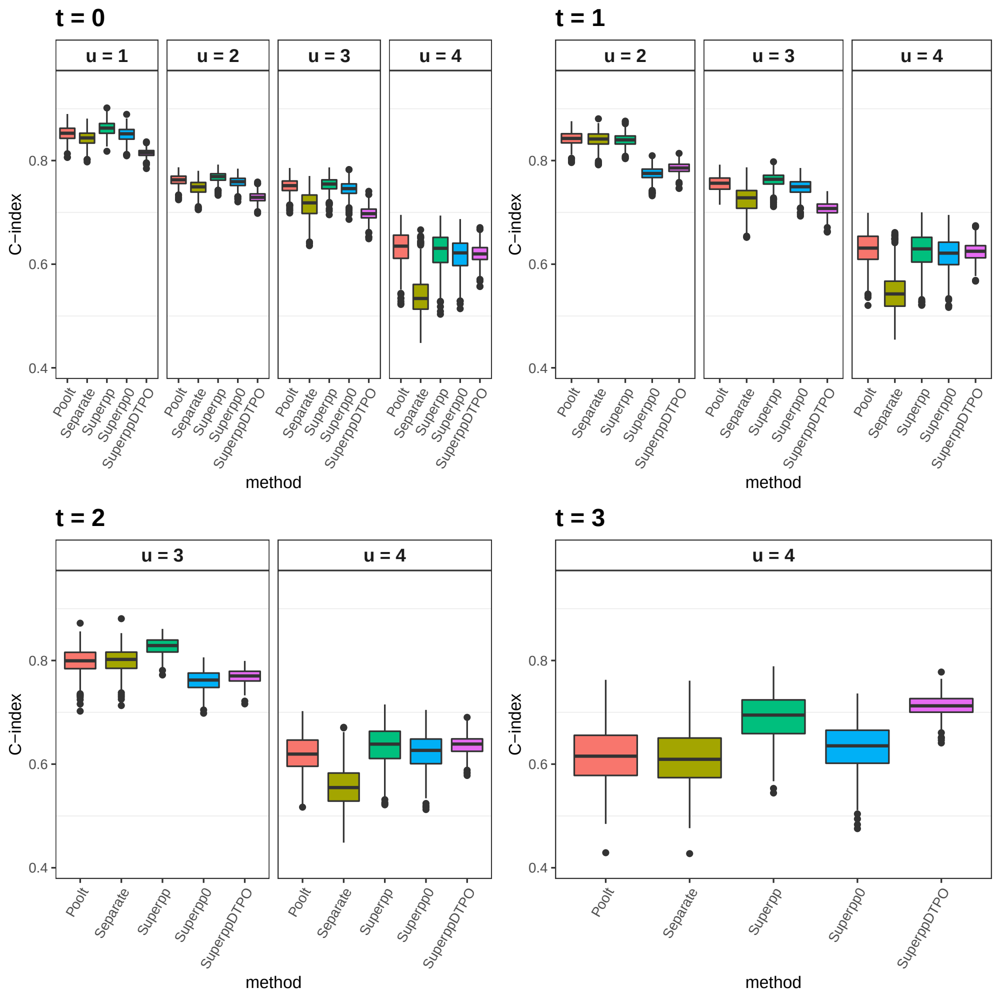


**Figure S1.49:** Simulation results comparing the distribution of C-index on test sets across methods for each pair of $(t, u)$, trained on sample data of size 1000, 50% censoring rate, generated following a Weibull distribution with an interaction survival relationship under the scenario 2TI + 4TV, low signal-to-noise ratio and weak autocorrelation. The number of periods $T = 4$.

## S1.3 Summary tables

Table S1.2 gives the performance comparison between two different numbers of periods, $T = 4$ and $T = 8$, when there are two time-invariant covariates and 4 time-varying covariates. Table S1.3 to S1.10 give performance comparison results when $T = 4$ for factor SNR, autocorrelation, survival relationship, survival distribution, censoring rate, training sample size, and estimation horizon, respectively.

In each of these summary tables, we provide *Value* and *Rank* for each method at every level of the factor. The average gains (in rank) for the method going from one level to the other are also provided to show how the factors affect the performance of a given method.

We will introduce how *Value* and *Rank* are computed, and then we will use Table S1.2 as an example to explain how one should interpret these values for performance comparison.

*Value* and *Rank* are computed as follows,

1. Given a specific level of $T$, SNR, autocorrelation, survival relationship, survival distribution, censoring rate, training sample size, and estimation horizon, we compute the mean rank over $n_{\text{sim}}$ simulations (here $n_{\text{sim}} = 500$) as follows:

   (a) In each round of the simulation, rank the method based on the

given measurement (ADIST, ALOR or C-index). Given a measurement, let $r_{1,M}, \ldots, r_{n_{\text{sim}},M}$ be the sequence of rank values for method $M$ from the $n_{\text{sim}}$ simulations;

(b) Average over the $n_{\text{sim}}$ simulations: $\bar{r}_M = n_{\text{sim}}^{-1} \sum_{i=1}^{n_{\text{sim}}} r_{i,M}$.

For $T = 4$, for example, we have 4320 values of $\bar{r}_M$, as we have a balanced factorial design:

5 (scenario) $\times$ 2 (SNR) $\times$ 2 (autocorrelation) $\times$ 3 (survival relationship) $\times$ 3 (survival distribution) $\times$ 2 (censoring rate) $\times$ 3 (training sample size) $\times$ 4 (estimation horizon) = 4320.

Therefore, given any factor with overall $L$ levels, say, SNR with $L = 2$, we have $4320/2 = 2160$ *directly comparable* pairs, which means within each pair, only the SNR levels are different among all factors (levels of all other factors are the same).

2. To summarize the performance comparison given $T = 4$ for a given factor with overall $L$ levels,

   - *Value* for method $M$ at each level $l$ is obtained by averaging $\bar{r}_M$ from Step 1 over all *directly comparable* cases of size $4320/L$ at this level $l$, $l = 1, \ldots, L$.

   - *Rank* for method $M$ at each level $l$ in the table then is obtained

by ranking *Value* among the three methods.

For summary of the comparison between $T = 4$ and $T = 8$ in the scenario 2TI + 4TV, *Value* and *Rank* for each level of $T$ can be obtained similarly based on the $\bar{r}_M$ from 864 cases computed in Step 1.

Table S1.2 provides the performance comparison among the three forest methods according to the factor $T$ (the number of periods), as well as the difference between the two levels, $T = 4$ and $T = 8$. First, we focus on the performance comparison at each level. When $T = 4$, based on the evaluation method ADIST, the average rank for the Separate method is 2.43, Poolt 2.02 and Superpp 1.55, while for C-index, the average rank for Separate is 2.75, Poolt 1.86 and Superpp 1.38. Under both measurements, Superpp gives the lowest mean rank over all *directly comparable* pairs and Separate gives the highest, which means Superpp outperforms the other two methods and Separate performs the worst. One can also tell that Superpp ranks the best more often when evaluated by C-index than when evaluated by ADIST since $1.38 < 1.55$. When $T = 8$, one can see that under all three measurements, Superpp is the best strategy and it ranks the best most often when evaluated by C-index, then by ADIST and least often by ALOR.

The last row "4 vs. 8" compares the two levels $T = 4$ and $T = 8$ using the difference $(\{T = 4\} - \{T = 8\})$ computed for each method under each

evaluation measurement. This gives the average gain (in rank) for the method when going from $T = 4$ to $T = 8$. The mean rank of the Separate method drops under all three evaluation measurements, that of Poolt stays roughly the same under ADIST but increases under ALOR and C-index, and that of Superpp increases under both ADIST and ALOR but drops under C-index. Based on these numbers, one can say that based on the goal of estimating hazard function more accurately, the Separate method gives slightly better comparative performance when the number of periods is smaller, and both Poolt and Superpp gain from the additional number of periods; based on the goal of classification and correct ranking, both Separate and Superpp relatively deteriorate when the number of periods gets smaller while Poolt relatively gains. Nevertheless, Superpp is always the best strategy for these two given number of periods.

**Table S1.2:** Summary table for different number of periods $T$ – Mean rank (Value) and the rank of mean rank (Rank) in the scenario of 2TI + 4TV.

| | ADIST | | | | | | ALOR | | | | | | C-index | | | | | |
|---|---|---|---|---|---|---|---|---|---|---|---|---|---|---|---|---|---|---|
| Number of | Separate | | Poolt | | Superpp | | Separate | | Poolt | | Superpp | | Separate | | Poolt | | Superpp | |
| periods | Value | Rank | Value | Rank | Value | Rank | Value | Rank | Value | Rank | Value | Rank | Value | Rank | Value | Rank | Value | Rank |
| $T = 4$ | 2.43 | 3 | 2.02 | 2 | 1.55 | 1 | 2.34 | 3 | 2.04 | 2 | 1.61 | 1 | 2.75 | 3 | 1.86 | 2 | 1.38 | 1 |
| $T = 8$ | 2.46 | 3 | 2.02 | 2 | 1.52 | 1 | 2.45 | 3 | 1.99 | 2 | 1.56 | 1 | 2.84 | 3 | 1.74 | 2 | 1.41 | 1 |
| 4 vs. 8 | −0.03 | 0 | 0.00 | 0 | 0.03 | 0 | −0.11 | 0 | 0.05 | 0 | 0.06 | 0 | −0.09 | 0 | 0.12 | 0 | −0.03 | 0 |

**Table S1.3:** Summary table for different scenarios in terms of different TI/TV combinations – Mean rank (Value) and the rank of mean rank (Rank) when $T = 4$.

| TI/TV | ADIST | | | | | | ALOR | | | | | | C-index | | | | | |
|---|---|---|---|---|---|---|---|---|---|---|---|---|---|---|---|---|---|---|
| | Separate | | Poolt | | Superpp | | Separate | | Poolt | | Superpp | | Separate | | Poolt | | Superpp | |
| | Value | Rank | Value | Rank | Value | Rank | Value | Rank | Value | Rank | Value | Rank | Value | Rank | Value | Rank | Value | Rank |
| 0/2 | 2.52 | 3 | 1.89 | 2 | 1.59 | 1 | 2.46 | 3 | 1.90 | 2 | 1.64 | 1 | 2.63 | 3 | 1.92 | 2 | 1.44 | 1 |
| 0/4 | 2.32 | 3 | 1.93 | 2 | 1.74 | 1 | 2.24 | 3 | 1.95 | 2 | 1.81 | 1 | 2.63 | 3 | 1.91 | 2 | 1.44 | 1 |
| 1/4 | 2.37 | 3 | 1.97 | 2 | 1.66 | 1 | 2.30 | 3 | 1.99 | 2 | 1.71 | 1 | 2.67 | 3 | 1.88 | 2 | 1.44 | 1 |
| 2/1 | 2.63 | 3 | 2.04 | 2 | 1.33 | 1 | 2.52 | 3 | 2.05 | 2 | 1.43 | 1 | 2.87 | 3 | 1.91 | 2 | 1.21 | 1 |
| 2/4 | 2.44 | 3 | 2.02 | 2 | 1.55 | 1 | 2.34 | 3 | 2.04 | 2 | 1.61 | 1 | 2.75 | 3 | 1.86 | 2 | 1.38 | 1 |
| 0/2 vs. 0/4 | 0.19 | 0 | −0.04 | 0 | −0.15 | 0 | 0.21 | 0 | −0.05 | 0 | −0.17 | 0 | 0.00 | 0 | 0.01 | 0 | 0.00 | 0 |
| 1/4 vs. 2/4 | −0.07 | 0 | −0.04 | 0 | 0.11 | 0 | −0.04 | 0 | −0.06 | 0 | 0.10 | 0 | −0.08 | 0 | 0.02 | 0 | 0.06 | 0 |
| 2/1 vs. 2/4 | 0.19 | 0 | 0.03 | 0 | −0.22 | 0 | 0.18 | 0 | 0.01 | 0 | −0.18 | 0 | 0.12 | 0 | 0.05 | 0 | −0.17 | 0 |

**Table S1.4:** Summary table for different signal-to-noise ratios (SNR) – Mean rank (Value) and the rank of mean rank (Rank) when $T = 4$.

| SNR | ADIST | | | | | | ALOR | | | | | | C-index | | | | | |
|---|---|---|---|---|---|---|---|---|---|---|---|---|---|---|---|---|---|---|
| | Separate | | Poolt | | Superpp | | Separate | | Poolt | | Superpp | | Separate | | Poolt | | Superpp | |
| | Value | Rank | Value | Rank | Value | Rank | Value | Rank | Value | Rank | Value | Rank | Value | Rank | Value | Rank | Value | Rank |
| High | 2.28 | 3 | 2.05 | 2 | 1.67 | 1 | 2.16 | 3 | 2.08 | 2 | 1.77 | 1 | 2.64 | 3 | 1.93 | 2 | 1.42 | 1 |
| Low | 2.63 | 3 | 1.89 | 2 | 1.47 | 1 | 2.58 | 3 | 1.90 | 2 | 1.52 | 1 | 2.78 | 3 | 1.86 | 2 | 1.35 | 1 |
| H vs. L | −0.36 | 0 | 0.16 | 0 | 0.20 | 0 | −0.43 | 0 | 0.18 | 0 | 0.25 | 0 | −0.14 | 0 | 0.07 | 0 | 0.07 | 0 |

**Table S1.5:** Summary table for different autocorrelation types – Mean rank (Value) and the rank of mean rank (Rank) when $T = 4$.

| | ADIST | | | | | | ALOR | | | | | | C-index | | | | | |
|---|---|---|---|---|---|---|---|---|---|---|---|---|---|---|---|---|---|---|
| Auto- | Separate | | Poolt | | Superpp | | Separate | | Poolt | | Superpp | | Separate | | Poolt | | Superpp | |
| correlation | Value | Rank | Value | Rank | Value | Rank | Value | Rank | Value | Rank | Value | Rank | Value | Rank | Value | Rank | Value | Rank |
| Strong | 2.48 | 3 | 1.99 | 2 | 1.53 | 1 | 2.38 | 3 | 2.01 | 2 | 1.61 | 1 | 2.77 | 3 | 1.87 | 2 | 1.35 | 1 |
| Weak | 2.43 | 3 | 1.95 | 2 | 1.62 | 1 | 2.36 | 3 | 1.96 | 2 | 1.68 | 1 | 2.66 | 3 | 1.93 | 2 | 1.41 | 1 |
| S vs. W | 0.05 | 0 | 0.04 | 0 | −0.09 | 0 | 0.02 | 0 | 0.06 | 0 | −0.07 | 0 | 0.11 | 0 | −0.06 | 0 | −0.06 | 0 |

**Table S1.6:** Summary table for different survival distributions – Mean rank (Value) and the rank of mean rank (Rank) when $T = 4$.

| Distribution | ADIST | | | | | | ALOR | | | | | | C-index | | | | | |
|---|---|---|---|---|---|---|---|---|---|---|---|---|---|---|---|---|---|---|
| | Separate | | Poolt | | Superpp | | Separate | | Poolt | | Superpp | | Separate | | Poolt | | Superpp | |
| | Value | Rank | Value | Rank | Value | Rank | Value | Rank | Value | Rank | Value | Rank | Value | Rank | Value | Rank | Value | Rank |
| Exponential | 2.49 | 3 | 1.93 | 2 | 1.58 | 1 | 2.37 | 3 | 1.94 | 2 | 1.69 | 1 | 2.70 | 3 | 1.88 | 2 | 1.40 | 1 |
| Gompertz | 2.35 | 3 | 2.05 | 2 | 1.60 | 1 | 2.29 | 3 | 2.06 | 2 | 1.65 | 1 | 2.69 | 3 | 1.92 | 2 | 1.39 | 1 |
| Weibull-I | 2.52 | 3 | 1.94 | 2 | 1.54 | 1 | 2.45 | 3 | 1.96 | 2 | 1.59 | 1 | 2.75 | 3 | 1.89 | 2 | 1.36 | 1 |
| E vs. G | 0.14 | 0 | −0.12 | 0 | −0.02 | 0 | 0.08 | 0 | −0.12 | 0 | 0.04 | 0 | 0.02 | 0 | −0.04 | 0 | 0.01 | 0 |
| E vs. W | −0.03 | 0 | −0.02 | 0 | 0.05 | 0 | −0.09 | 0 | −0.02 | 0 | 0.10 | 0 | −0.04 | 0 | −0.01 | 0 | 0.03 | 0 |
| G vs. W | −0.17 | 0 | 0.10 | 0 | 0.06 | 0 | −0.16 | 0 | 0.10 | 0 | 0.06 | 0 | −0.06 | 0 | 0.04 | 0 | 0.02 | 0 |

**Table S1.7:** Summary table for different survival relationships – Mean rank (Value) and the rank of mean rank (Rank) when $T = 4$.

| Model | ADIST | | | | | | ALOR | | | | | | C-index | | | | | |
|---|---|---|---|---|---|---|---|---|---|---|---|---|---|---|---|---|---|---|
| | Separate | | Poolt | | Superpp | | Separate | | Poolt | | Superpp | | Separate | | Poolt | | Superpp | |
| | Value | Rank | Value | Rank | Value | Rank | Value | Rank | Value | Rank | Value | Rank | Value | Rank | Value | Rank | Value | Rank |
| Interaction | 2.38 | 3 | 2.02 | 2 | 1.60 | 1 | 2.27 | 3 | 2.04 | 2 | 1.69 | 1 | 2.65 | 3 | 1.94 | 2 | 1.40 | 1 |
| Linear | 2.49 | 3 | 1.92 | 2 | 1.59 | 1 | 2.46 | 3 | 1.91 | 2 | 1.63 | 1 | 2.75 | 3 | 1.86 | 2 | 1.39 | 1 |
| Nonlinear | 2.49 | 3 | 1.97 | 2 | 1.53 | 1 | 2.39 | 3 | 2.00 | 2 | 1.61 | 1 | 2.74 | 3 | 1.90 | 2 | 1.36 | 1 |
| I vs. L | −0.11 | 0 | 0.10 | 0 | 0.01 | 0 | −0.19 | 0 | 0.13 | 0 | 0.06 | 0 | −0.09 | 0 | 0.08 | 0 | 0.01 | 0 |
| I vs. N | −0.11 | 0 | 0.05 | 0 | 0.07 | 0 | −0.13 | 0 | 0.05 | 0 | 0.08 | 0 | −0.08 | 0 | 0.04 | 0 | 0.04 | 0 |
| L vs. N | 0.00 | 0 | −0.06 | 0 | 0.05 | 0 | 0.06 | 0 | −0.09 | 0 | 0.02 | 0 | 0.01 | 0 | −0.04 | 0 | 0.03 | 0 |

**Table S1.8:** Summary table for different censoring rates – Mean rank (Value) and the rank of mean rank (Rank) when $T = 4$.

| Censoring rate | ADIST | | | | | | ALOR | | | | | | C-index | | | | | |
|---|---|---|---|---|---|---|---|---|---|---|---|---|---|---|---|---|---|---|
| | Separate | | Poolt | | Superpp | | Separate | | Poolt | | Superpp | | Separate | | Poolt | | Superpp | |
| | Value | Rank | Value | Rank | Value | Rank | Value | Rank | Value | Rank | Value | Rank | Value | Rank | Value | Rank | Value | Rank |
| 10% | 2.31 | 3 | 2.09 | 2 | 1.60 | 1 | 2.22 | 3 | 2.13 | 2 | 1.65 | 1 | 2.70 | 3 | 1.89 | 2 | 1.41 | 1 |
| 50% | 2.60 | 3 | 1.85 | 2 | 1.55 | 1 | 2.53 | 3 | 1.84 | 2 | 1.63 | 1 | 2.73 | 3 | 1.90 | 2 | 1.36 | 1 |
| L vs. H | −0.28 | 0 | 0.23 | 0 | 0.05 | 0 | −0.31 | 0 | 0.29 | 0 | 0.02 | 0 | −0.03 | 0 | −0.01 | 0 | 0.05 | 0 |

**Table S1.9:** Summary table for different training sample sizes – Mean rank (Value) and the rank of mean rank (Rank) when $T = 4$.

| Sample size | ADIST | | | | | | ALOR | | | | | | C-index | | | | | |
|---|---|---|---|---|---|---|---|---|---|---|---|---|---|---|---|---|---|---|
| | Separate | | Poolt | | Superpp | | Separate | | Poolt | | Superpp | | Separate | | Poolt | | Superpp | |
| | Value | Rank | Value | Rank | Value | Rank | Value | Rank | Value | Rank | Value | Rank | Value | Rank | Value | Rank | Value | Rank |
| $n = 200$ | 2.39 | 3 | 2.06 | 2 | 1.55 | 1 | 2.36 | 3 | 2.06 | 2 | 1.58 | 1 | 2.65 | 3 | 1.92 | 2 | 1.42 | 1 |
| $n = 1000$ | 2.47 | 3 | 1.95 | 2 | 1.58 | 1 | 2.38 | 3 | 1.96 | 2 | 1.66 | 1 | 2.73 | 3 | 1.87 | 2 | 1.40 | 1 |
| $n = 5000$ | 2.51 | 3 | 1.91 | 2 | 1.59 | 1 | 2.38 | 3 | 1.94 | 2 | 1.68 | 1 | 2.76 | 3 | 1.90 | 2 | 1.33 | 1 |
| 200 vs. 1000 | −0.19 | 0 | 0.13 | 0 | 0.06 | 0 | −0.09 | 0 | 0.08 | 0 | 0.01 | 0 | −0.11 | 0 | 0.10 | 0 | 0.01 | 0 |
| 1000 vs. 5000 | 0.06 | 0 | −0.08 | 0 | 0.02 | 0 | 0.01 | 0 | −0.04 | 0 | 0.03 | 0 | 0.00 | 0 | −0.05 | 0 | 0.05 | 0 |

**Table S1.10:** Summary table for different values of estimation horizon $(u-t)$ – Mean rank (Value) and the rank of mean rank (Rank) when $T=4$.

| | ADIST | | | | | | ALOR | | | | | | C-index | | | | | |
|---|---|---|---|---|---|---|---|---|---|---|---|---|---|---|---|---|---|---|
| Estimation | Separate | | Poolt | | Superpp | | Separate | | Poolt | | Superpp | | Separate | | Poolt | | Superpp | |
| horizon | Value | Rank | Value | Rank | Value | Rank | Value | Rank | Value | Rank | Value | Rank | Value | Rank | Value | Rank | Value | Rank |
| $u-t=1$ | 2.13 | 2 | 2.16 | 3 | 1.71 | 1 | 2.04 | 2 | 2.13 | 3 | 1.82 | 1 | 2.49 | 3 | 2.10 | 2 | 1.39 | 1 |
| $u-t=2$ | 2.71 | 3 | 1.89 | 2 | 1.40 | 1 | 2.63 | 3 | 1.93 | 2 | 1.43 | 1 | 2.91 | 3 | 1.81 | 2 | 1.28 | 1 |
| $u-t=3$ | 2.68 | 3 | 1.78 | 2 | 1.54 | 1 | 2.59 | 3 | 1.82 | 2 | 1.58 | 1 | 2.84 | 3 | 1.72 | 2 | 1.44 | 1 |
| $u-t=4$ | 2.56 | 3 | 1.83 | 2 | 1.61 | 1 | 2.46 | 3 | 1.88 | 2 | 1.66 | 1 | 2.77 | 3 | 1.70 | 2 | 1.54 | 1 |

## S1.4 The shrinkage effect of the Superpp method

Let $h$ be the true hazard and $\hat{h}_M$ the estimated hazard using method $M$. Figure S1.50 shows that a regression of the $h - \hat{h}_{\text{Superpp}}$ values on the $h - \hat{h}_{\text{Separate}}$ values for all of the $(t, u)$ pairs under all model setups. The regression has a slope less than 1 in 88% of the cases under all model setups, indicating that the hazard estimates using Superpp are shrunk towards a common value relative to those for Separate.

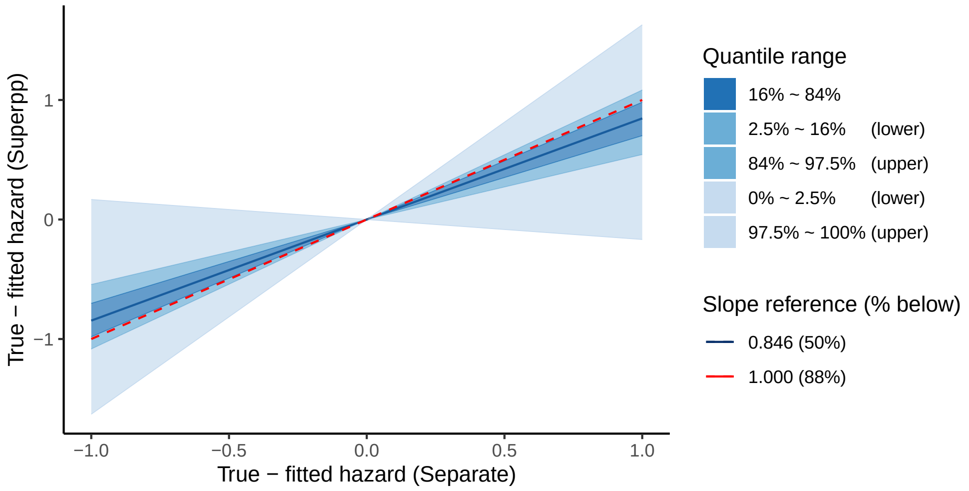


**Figure S1.50:** The regression of True - fitted hazard (Superpp) on True - fitted hazard (Separate) under all model setups.

## S2 Real data example

In this section, we revisit the bankruptcy data in Section 3 of Bou-Hamad et al. (2011a) about United States firms that conducted IPOs (Initial Public Offerings) between 1990 and 1999. The data comes from COMPUSTAT and each firm is followed yearly starting from its IPO until 2006. The target variable is the bankruptcy, measured in number of years after the IPO. All firms that filed for bankruptcy under Chapter 7 or 11 are considered bankrupt. The data set includes 1143 firms, of which 189 went bankrupt during the study. The time-varying covariates are the following financial ratios collected yearly:

- $X_1$ = Current Assets/Current Liabilities
- $X_2$ = Net Working Capital/Total Assets
- $X_3$ = Sales/Net Working Capital
- $X_4$ = Sales/Net Fixed Assets
- $X_5$ = Sales/Total Assets
- $X_6$ = Total Debt/Total Assets
- $X_7$ = Long–Term Debt/(Long–Term Debt+Total Equity)
- $X_8$ = Net Income/Total Assets

**Table S2.1:** The 10 different estimation problems $(year, t, u)$ with covariate information given at *year*. The initial IPO occurred in $year - t$ and the goal is to estimate hazard probability for bankruptcy in $year - t + u$ (with a estimation horizon $u - t$ after the IPO).

| Year after IPO | estimation needed for $(u)$ | | | |
|---|---|---|---|---|
| Current $(t)$ | 3 | 4 | 5 | 6 |
| 0 | ✓ | ✓ | ✓ | ✓ |
| 1 | | ✓ | ✓ | ✓ |
| 2 | | | ✓ | ✓ |
| 3 | | | | ✓ |

- $X_9$ = Net Income/Total Equity
- $X_{10}$ = Market Value of Equity/Book Value of Total Debt.

  In addition, the following time-invariant covariate is included:

- $X_{11}$ = Category based on Standard Industrial Classification (SIC) Division Structure.

In Bou-Hamad et al. (2011a), estimation at a horizon of three years was considered and only aggregate results were reported. This time, to make the investigation more complete and closer to a real practical application, we incorporate the time factor and include other estimation horizons. More

precisely, we suppose that we are in a given year (here it will be 1997, 1998, or 1999), and we want to estimate the hazards probabilities for the firms that are still currently operating, for horizons between three and six years. More precisely, at any given year, the goal is to estimate their hazard probabilities for years 3, 4, 5 and 6 after the IPO, using the values of covariates at years 0, 1 and 2. Let the tuple $(year, t, u)$ denote the estimation problem where we are given the firm's covariate information at $year$, which is $t$ years after its initial IPO, and we want to estimate the firm's hazard probability at $(year - t + u)$. Table S2.1 describes the scenarios that we investigate, which gives all possible combinations of $(year, t, u)$ for a given value of $year$. For example, suppose we are in $year = 1997$ and supplied with all the latest covariate information in $year = 1997$, we focus on those companies who are still operating and have their initial IPO in 1997, 1996 and 1995, i.e., $t = 0, 1, 2$, respectively, and estimate their hazard probabilities in 1998, 1999, 2000 and 2001, i.e., $u = 3, 4, 5, 6$, respectively. These companies make up the test data sets for the 10 estimation problems given in Table S2.1, $(year, t, u)$ with $year = 1997$.

Note that the training data set used to solve each of these ten estimation problems are constructed using the information strictly prior the the ones used in the corresponding test data set. For example, given the estimation problem $(year, t, u) = (1997, 3, 6)$, all companies that are still operating three years after their initial IPO (regardless which year the IPO was in), with

their covariate information at the third year and their event status at sixth year, can potentially be used to construct the training data set used in the Separate method. However, since realistically we should have no access to any information after the current $year = 1997$, the training data set should contain only those companies who have their initial IPO at least 6 years prior to $year = 1997$. Hence, the covariate information included in the training data set should come from the time that is at least 3 years prior to $year = 1997$, whereas the covariate information used to construct the corresponding test set are exactly extracted in $year = 1997$. The important issue is that this setup respects the chronological order and these analyses could all be performed in a real application.

We repeat this process for year 1998 and 1999. Consequently, we have 30 scenarios, 3 years $\times$ 10 pairs, for all possible combinations of $(year, t, u)$. To solve each of the corresponding estimation problems, one training data set and one test data set are constructed. Table S2.2 presents summary statistics for the number of firms at risk, the number of bankruptcies, and the percentage of bankruptcies for the overall 30 training data sets used in the Separate method and the 30 test data sets.

Note that the event for a given company may appear several times across different training data sets or test data sets. For example, for a company who had its initial IPO in year 1996 and went bankrupt in year 2002, its

event status in year 2002 can appear in three different test data sets: with its covariate information in $year = 1997, 1998, 1999$, it is part of the test data set for the estimation problem $(year, t, u) = (1997, 1, 6)$, $(1998, 2, 6)$, $(1998, 3, 6)$, respectively. The same company is also used to construct the training data sets: with its covariate information in 1996 and its event status in 1997, it appears in the training data sets for estimation problems $(year, t, u) = (1997, 0, 1), (1998, 0, 1), (1999, 0, 1)$. For another company who had its initial IPO in year 1991 and went bankrupt in 1996, it is not included in any test data sets but is included in 9 training data sets with the same event status in 1996: for estimation problems $(year, t, u) = (1997, 0, 5)$, $(1998, 0, 5)$, $(1999, 0, 5)$ with its covariate information in 1991; for the estimation problems $(year, t, u) = (1997, 1, 5)$, $(1998, 1, 5)$, $(1999, 1, 5)$ with its covariate information in 1992; for $(year, t, u) = (1997, 2, 5)$, $(1998, 2, 5)$, $(1999, 2, 5)$ with its covariate information in 1993. Although the same event for a given company is used multiple times to construct overall 30 training data sets or testing datasets, each time it is used is to supply different covariate information for a different estimation problem. That means for each of these estimation problems, the covariate information from a given firm appears only once in the corresponding training or testing data set. Therefore, no redundant or repeated information is used for solving a specific estimation problem. The following performance comparison is conducted with respect to each of the

**Table S2.2:** Summary of the data over the 30 scenarios

| | Training data | | |
|---|---|---|---|
| | Number of firms at risk | Number of bankruptcies | Proportion of bankruptcies (%) |
| Mean | 315.5 | 10.6 | 3.23 |
| Min | 95 | 2 | 2.10 |
| Max | 730 | 23 | 4.20 |
| | Test data | | |
| | Number of firms at risk | Number of bankruptcies | Proportion of bankruptcies (%) |
| Mean | 131.1 | 3.53 | 2.69 |
| Min | 93 | 1 | 0.68 |
| Max | 163 | 11 | 6.75 |

distinctive estimation problem.

The fact that bankruptcy is a rare event is clearly apparent which makes it challenging for both estimating the models and evaluating their performances. The same four forests-based methods are used to estimate the hazard probabilities for bankruptcy. To be clear, for a given year (e.g. 1997), 10 forests are built for the Separate method (one for each pair $((t, u))$), four forests are built for the Poolt method (one for each $t$), one forest is built for

the Superpp method, and another one for Superpp0. This process is used for each of the three years 1997, 1998, and 1999.

Figure S2.1 gives an example showing the estimated hazard probabilities for company INDUSTRIAL DISTRIBUTION GRP INC, using the Separate, Poolt and Superpp method, respectively. INDUSTRIAL DISTRIBUTION GRP INC had its initial IPO in 1997. Its estimated hazard probabilities in year 2000, 2001, 2002 and 2003 can be obtained by solving the estimation problems $(year, t, u)$ as in Table S2.1 with its covariate information provided at a given value of $year$. For example, the four estimated hazard probabilities on the red solid line are obtained by solving $(1997, 0, 3)$, $(1997, 0, 4)$, $(1997, 0, 5)$ and $(1997, 0, 6)$, respectively; the ones on the green short-dash line are obtained by solving $(1998, 1, 4)$, $(1998, 1, 5)$ and $(1998, 1, 6)$; the ones one the blue long-dash line are obtained by solving $(1999, 2, 5)$ and $(1999, 2, 6)$. Therefore, the red solid lines always use the covariate information obtained at the time of initial IPO; the green short-dash lines use information provided in year 1998 for estimation after year 2001; and the blue long-dash lines show results with covariate information given in year 1999 for estimation of hazard probabilities since year 2002.

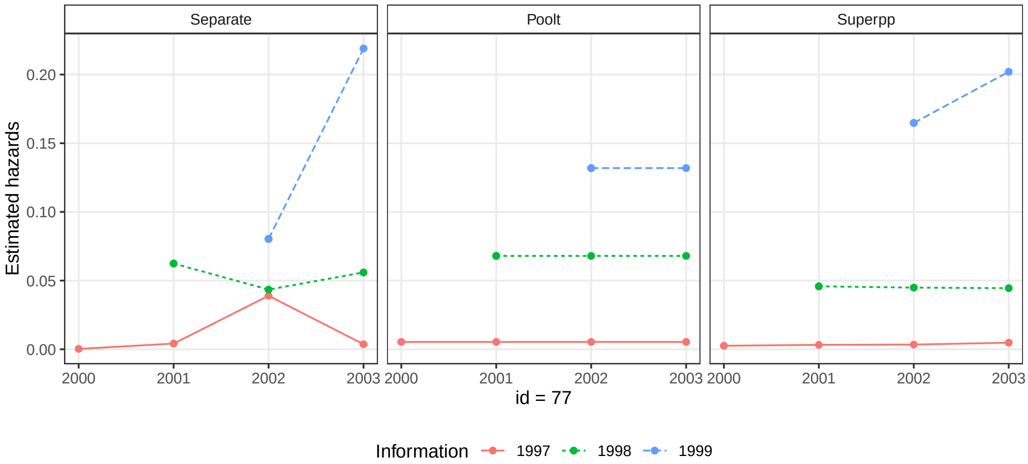


**Figure S2.1:** Estimated hazard probabilities for bankruptcy from year 2000 to 2002 for company INDUSTRIAL DISTRIBUTION GRP INC, using the Separate, Poolt and Superpp method, respectively. For each of the three methods used, the red solid line gives the estimated hazard probabilities with the firm's covariate information given in year 1997; the green short-dash line shows the estimated hazard probabilities for 2001, 2002 and 2003, with the covariate information given in year 1998; the blue long-dash line shows results with information given in 1999 for estimation in year 2002 and 2003.

Figure S2.1 illustrates the change of estimated hazard probabilities for bankruptcy in time given covariate information at some specific time point. For example, given the information in year 1997, the estimated hazard probabilities for bankruptcy in the subsequent years from 2000 to 2002 always remain low, since the information was obtained in the first year of the IPO. As we use the new covariate information in 1998 to estimate for hazards

from 2001 to 2003, the updated estimation shows a higher level of hazard probability, but still around the same level for all of the subsequent three years. Furthermore, with the covariate information available in 1999, the estimated hazard probabilities for the years since 2002 start from a higher level, and we see a huge increase from year 2002 to 2003 using both Separate and Superpp method. A sudden change in the hazards could happen if an important covariate changed dramatically. For example, an infusion of cash or a successful launch of a new product may bring a drop in the hazard probability for bankruptcy, while economic downturns usually have a huge negative impact on individual company, bringing an upturn in hazard probability. The financial crisis in the late 1990's may well explain the increasing level of hazard probabilities as we update the information. Regulators may want to use this information to further investigate whether these sudden changes may indicate a deeper management problem or are a result of global economic downturns. It would also help investors to make better judgements when looking for new promising startups in which to invest.

The true hazard functions are of course unknown for these companies. Cumulative gains charts, Area Under the Cumulative Gain Curve (AUCGC), and the Brier score (BS), each obtained based on the test data, are used to evaluate the performance. A cumulative gains chart plots the percentage of events (here bankruptcies) detected if the $p\%$ of the observations with

the highest estimated probabilities are classified as events, as a function of $p$. Hence it measures the ability of a model to detect events compared to random assignment. The area under this curve provides a single value performance measure, larger being better. The Brier score for a binary problem is defined as follows

$$\text{BS} = \frac{1}{n_{\text{test}}} \sum_{i=1}^{n_{\text{test}}} \left(\hat{h}_i - y_i\right)^2 \tag{1}$$

and measures the difference between the estimated hazards $\hat{h}_i$ and the binary realization of the event $y_i$ over the test data set. Note that the cumulative gains and the Brier score evaluate methods from different perspectives. The cumulative gains is a ranking-based metric to measure effectiveness while the Brier score measures the quality of the estimation (calibration). The cumulative gains and Brier scores on the test data are computed separately for each method and each of the 30 scenarios. Figures S2.2 and S2.3 provide the average cumulative gains curves for the 12 scenarios with an estimation horizon of 3 years and for the 18 scenarios with a horizon greater than 3 years, respectively. Table S2.3 provides the average AUCGC and Brier scores for the same two groups of scenarios. Variable importance (VIMP) values (Breiman, 2001), which are calculated by permuting a variable and then calculating the change in prediction error compared to the original ordering of the values, are obtained for all 11 covariates on the training data set using the Superpp

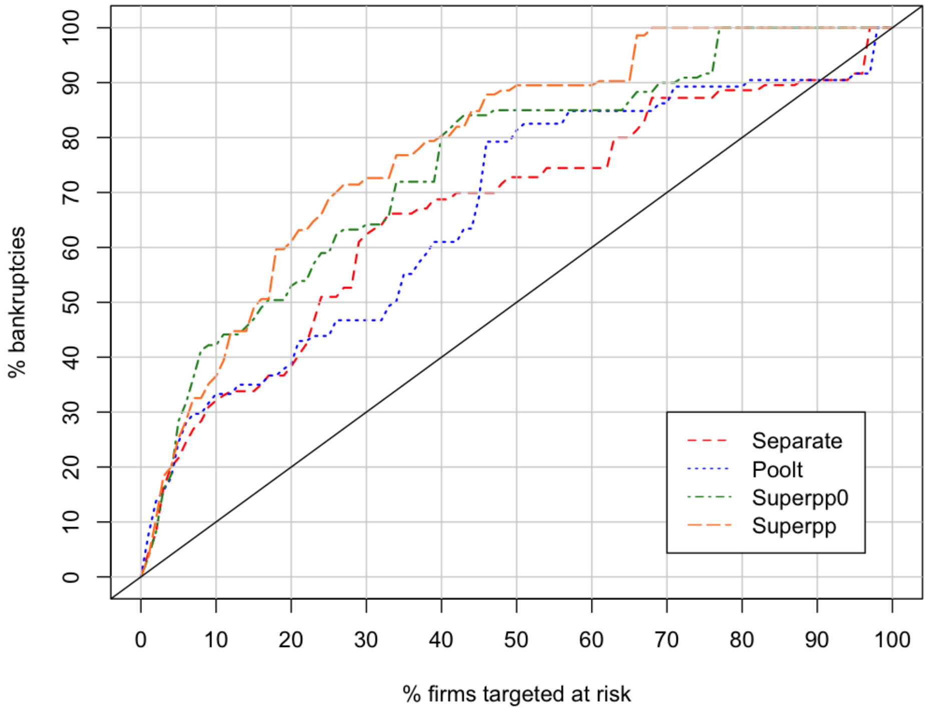


**Figure S2.2:** Average cumulative gains curves for the 12 scenarios with an estimation horizon of 3 years

method. The results are given in Figure S2.4.

When the estimation horizon is 3 years, Figure S2.2 and the AUCGC values in Table S2.3 show that all methods perform better than random assignment (the diagonal line). In particular, Figure S2.2 shows that Superpp and Superpp0 outperform the other two methods, and the Superpp method has a slight edge over Superpp0. For instance, if we target 20% of the firms with the highest probability of bankruptcies, then Superpp detects around

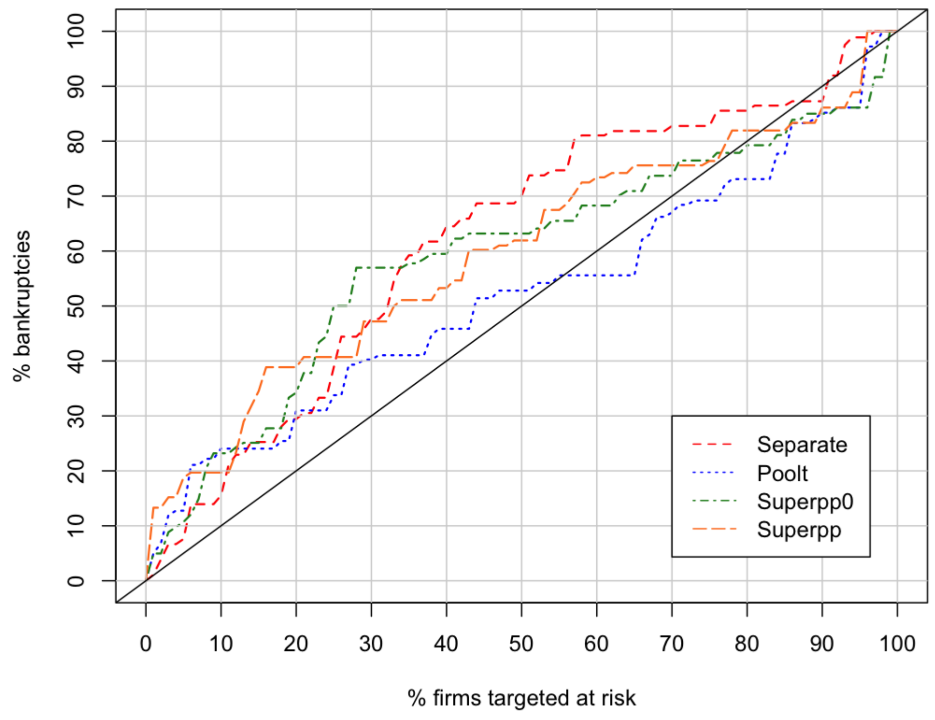


**Figure S2.3:** Average cumulative gains curves for the 18 scenarios with an estimation horizon greater than 3 years

61% of the bankruptcies on average, and Superpp0 around 52%, which are both much higher than the better of the two other methods (which detects 40% of bankruptcies). In Table S2.3, one can also see Superpp has the highest AUCGC, Superpp0 follows, Poolt and Separate fall behind but still have values greater than 50 (random assignment).

**Table S2.3:** Average AUCGC and average Brier scores with respect to the estimation horizon

| AUCGC (larger the better) | | | | |
|---|---|---|---|---|
| Horizon | Separate | Poolt | Superpp0 | Superpp |
| 3 | 66.7 | 66.6 | 75.1 | 78.4 |
| 4 or more | 62.3 | 52.1 | 59.2 | 59.7 |
| **Brier score (lower the better)** | | | | |
| Horizon | Separate | Poolt | Superpp0 | Superpp |
| 3 | 0.0348 | 0.0355 | 0.0362 | 0.0342 |
| 4 or more | 0.0212 | 0.0216 | 0.0244 | 0.0214 |

When the estimation horizon is 4 or more years, values of AUCGC for all methods in Table S2.3 are still larger than 50 but become smaller, which indicates that the performance is still better than random assignment but worse than for the scenarios with a horizon of 3 years. That can also be concluded from Figure S2.3, where one can see the cumulative gain curves now lie closer to the diagonal line and sometimes fall below it. This is unsurprising, since it is more difficult to estimate the bankruptcy for horizons further away. Moreover, the Separate method has the highest detection rate when the target percentage is higher than 35%. It has a slightly higher value of AUCGC than the other methods, followed by Superpp and Superpp0.

Superpp detects a slightly higher percentage of bankruptcies than Superpp0 when the given target percentage is less than 20% or higher than 50%. Poolt performs the worst and its cumulative gain curve falls below the diagonal line when the target percentage is more than 55%.

For either estimation horizon, Figures S2.2 and S2.3 along with the AUCGC values given in Table S2.3 show that Superpp0 can perform as well as Superpp and sometimes much better than Separate and Poolt. This may seem puzzling since Superpp0 never updates its initial information for estimation at any later time. However, note that the evaluation results given in Figures S2.2, S2.3 and the AUCGC values given in Table S2.3 are made based on the cumulative gains, a rank-based metric. If we evaluate the performance from a calibration perspective by using the BS score, one can see from Table S2.3 that all other forest methods give smaller values of Brier scores than Superpp0 regardless of the estimation horizon, which implies that those methods give higher accuracy of probabilistic estimation in the binary problems.

In addition, Superpp0 performing well can also be partly explained by the extremely high censoring rate (around 97%) in the test sets. As the estimation horizon increases from 3 to 6 years, the number of events in the test sets for any given year decreases from 4 to 1. Presumably, the censoring rate is so high that the dynamic information can hardly help Superpp to gain an edge over Superpp0. A simpler method with a lower variance, though more

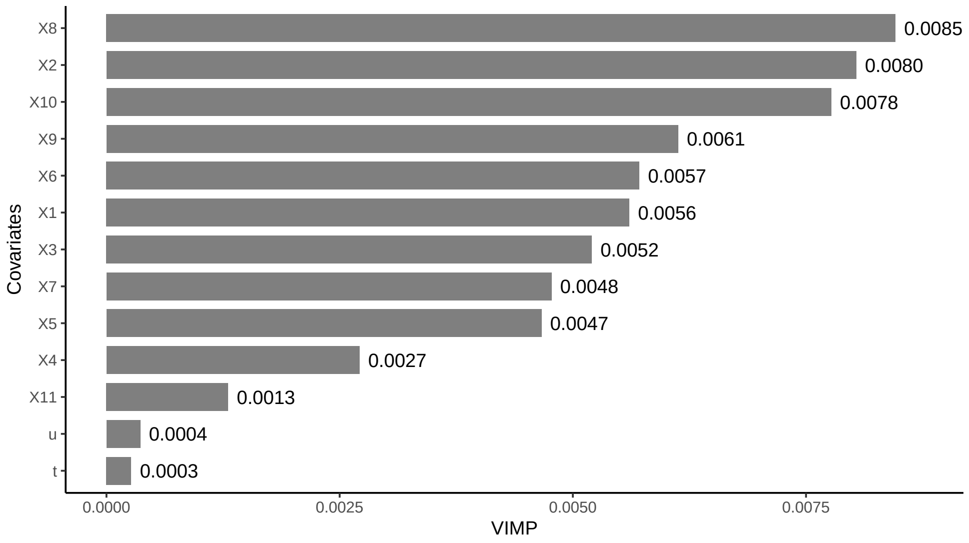


**Figure S2.4:** Average variable importance (VIMP) values of each covariate in estimation of bankruptcies using the Superpp method over year 1997, 1998 and 1999.

biased, can work well for ordering the firms according to their risks. This can also explain why Superpp performs better than both Separate and Poolt when the estimation horizon is as small as 3 years.

As the estimation horizon increases, the results from cumulative gains and BS indicate that the Superpp method loses its edge over Separate and Poolt. This does not, however, contradict the simulation results where we see Superpp gains advantage over the other two methods as the estimation horizon increases. In fact, the VIMP measures can help explain the reason why the gains of pooling are limited in the analysis. Figure S2.4 provides the averaged VIMP values for each covariate used in the Superpp method over

the three years. One can see that $t$ and $u$ are ranked as the least important covariates in the training process. VIMP measures indicate that there is little additional information in $t$ and $u$. Recall that the Superpp method estimates use all information available for each $(t, u)$ scenario, and it provides superior performance because of the additional information in varying $t$ and $u$. Thus, $t$ and $u$ being least important leaves Superpp in an unfavorable situation. In addition, $X_{11}$, the only time-invariant covariate among the 11 covariates, is apparently much less important than the other (time-varying) covariates. These data therefore resemble the cases in the simulation studies where we have a high proportion of time-varying covariates in the true model. In these cases, Separate (and Poolt) tend to outperform Superpp in this situation since they are more sensitive to the time-varying feature by design.
